# Supplementary material for: Identifying and Exploiting Structures for Reliable Deep Learning
Source: arXiv:2108.07083 source file (2021-08-16)
Supplement: Supplementary file 1 [file appendix_figs.tex]

\subsection*{Convergence graphs of $\vec{G}\vec{G}^\top$}

\begin{figure}[h]
  \centering
  \includegraphics[width=\textwidth]{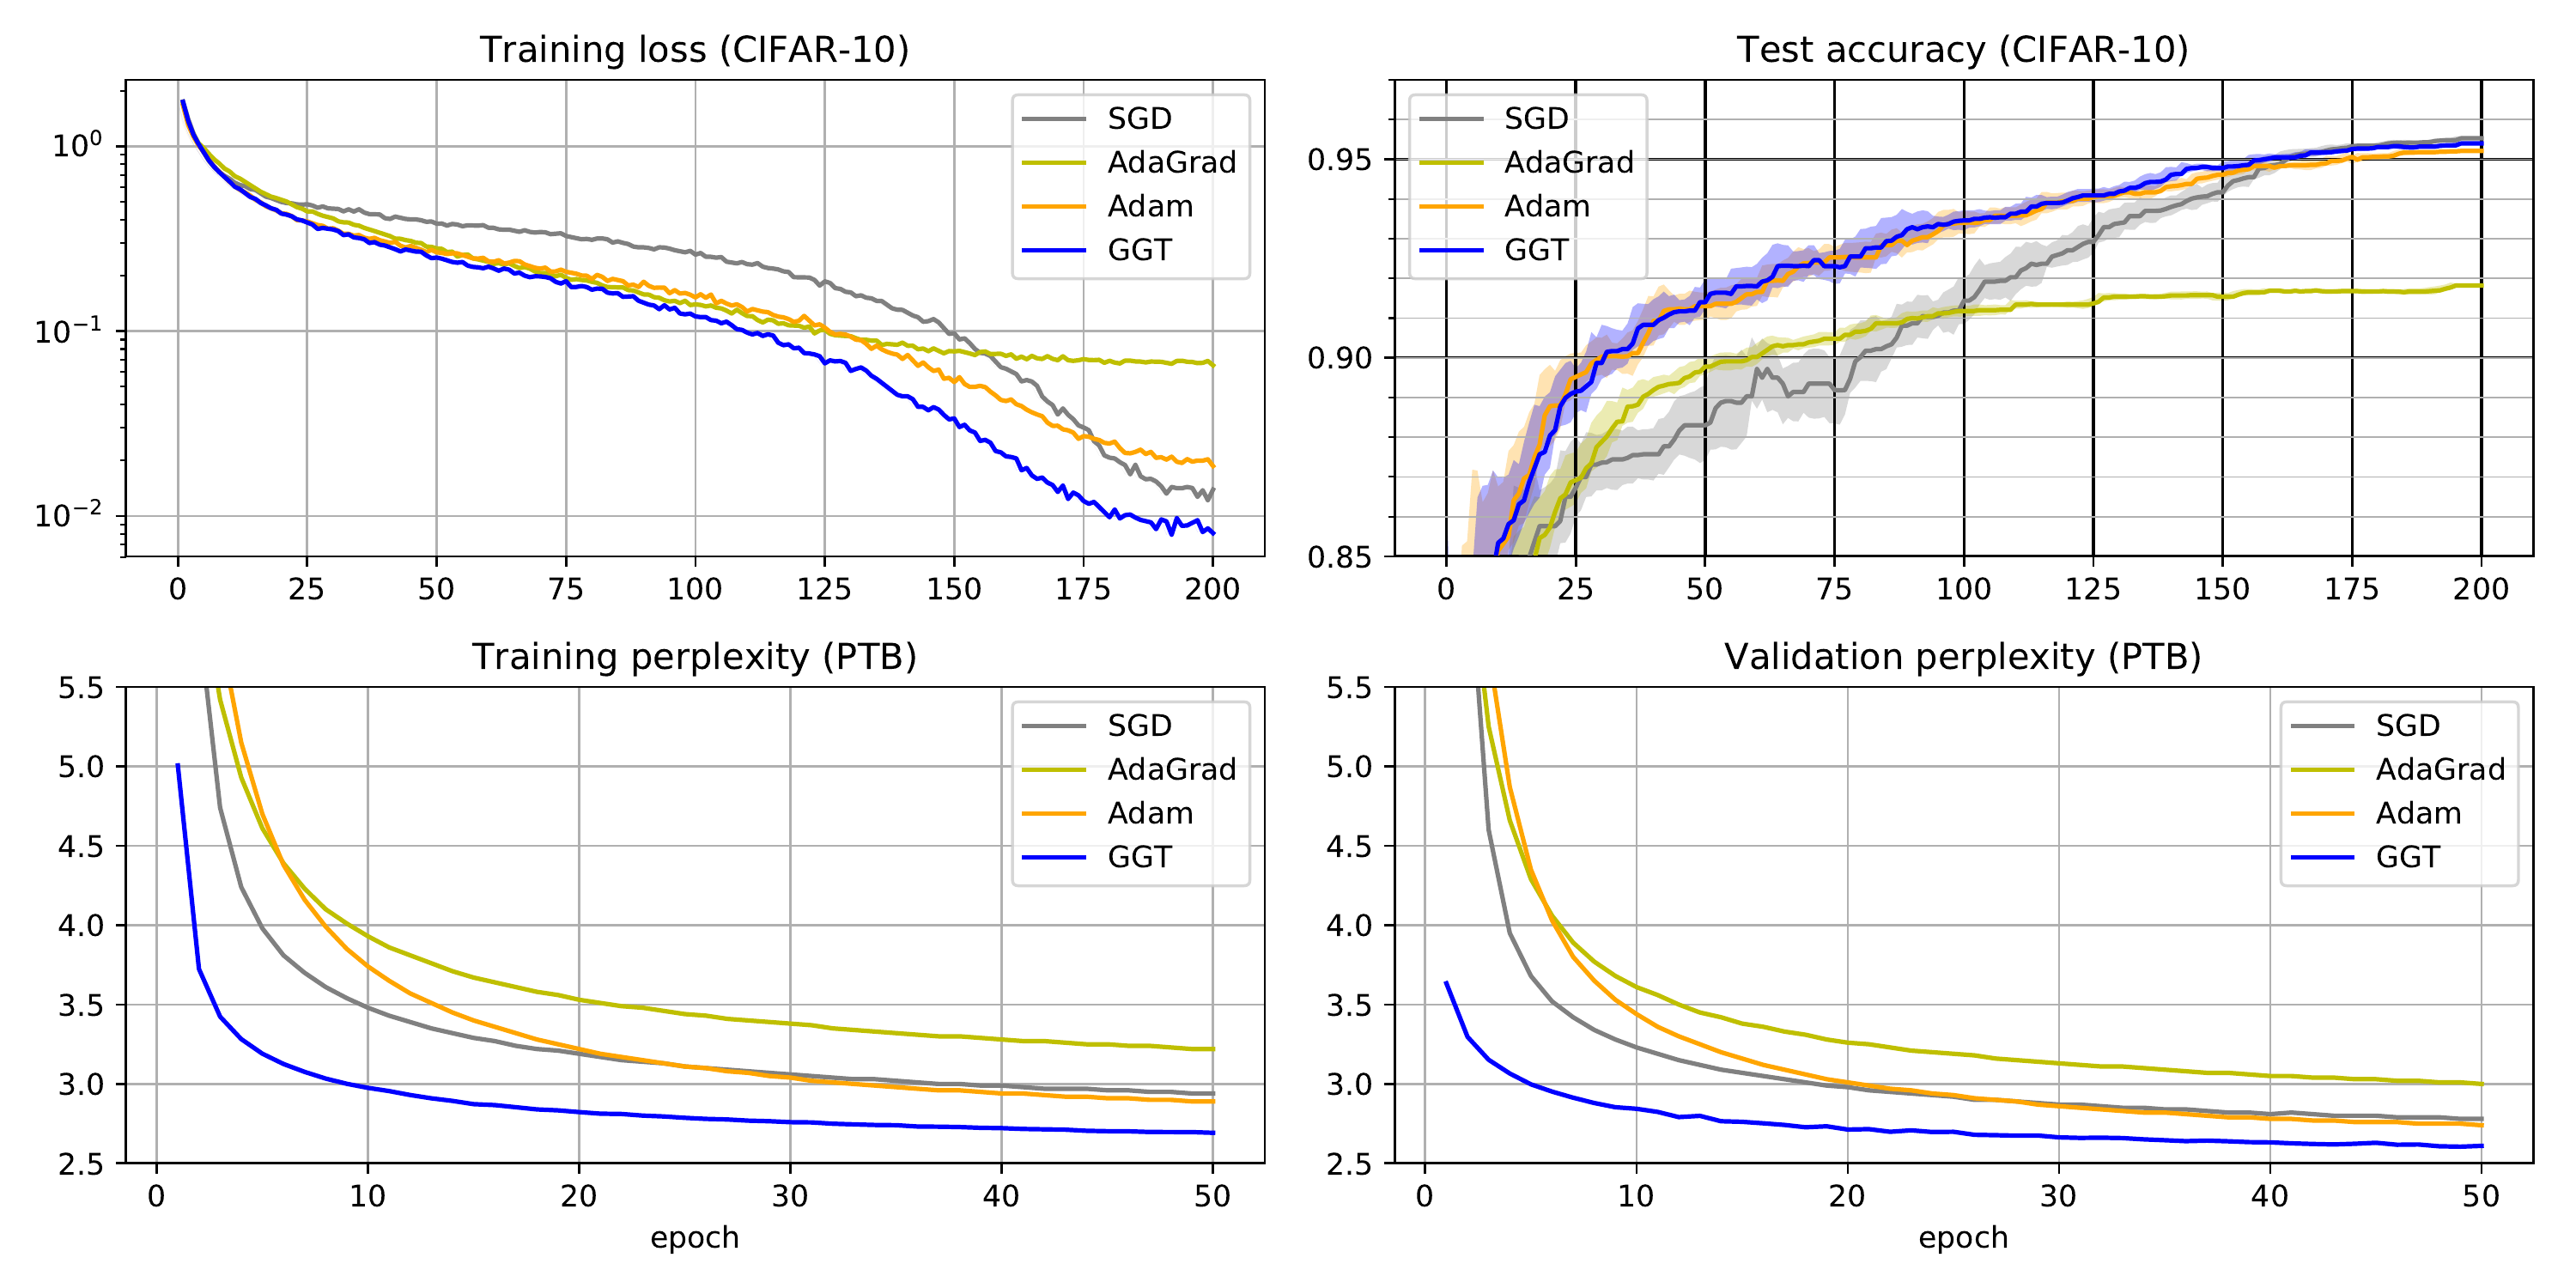}
  \caption{Results of CNN and RNN experiments. $\vec{G}\vec{G}^\top$ shows faster progress towards the beginning in the case of RNNs and towards the end in CNNs.
  }
  \label{fig:cnn-rnn}
\end{figure}

  \clearpage\subsection{Margin Distributions from~\cite{bartlett2017spectrally}}
\begin{figure}[h!]
  \centering
  \begin{subfigure}[t]{0.49\textwidth}
    \includegraphics[width = 1.0\textwidth]{paperplots_3_cifar_mnist-crop.pdf}
    \caption{MNIST is easier than CIFAR10.\label{fig:mnist:1}}
  \end{subfigure}\hfill
  \begin{subfigure}[t]{0.49\textwidth}
    \includegraphics[width = 1.0\textwidth]{paperplots_3_cifar_mnist_2-crop.pdf}
    \caption{Random MNIST is as hard as random CIFAR10!\label{fig:mnist:2}}
  \end{subfigure}
  \vfill
  \begin{subfigure}[t]{0.49\textwidth}
    \includegraphics[width = 1.0\textwidth]{paperplots_3_cifar100-crop.pdf}
    \caption{CIFAR100 is as hard as CIFAR10
    with random labels! \label{fig:cifar100}    }\end{subfigure}\hfill
    \begin{subfigure}[t]{0.49\textwidth}
    \includegraphics[width = 1.0\textwidth]{paperplots_3_rand_input-crop.pdf}
    \caption{Random inputs are harder than random labels.\label{fig:randim}}
  \end{subfigure}
  \caption{A variety of margin distributions.  Axes are re-scaled in \ref{fig:mnist:1},
  but identical in the other subplots;
  the CIFAR10 (blue) and random CIFAR10 (green) distributions are the same each time.}
\label{fig:spectral-images}
\end{figure}

\clearpage
\subsection*{Normal and Encrypted Prediction As a Service paradigms}

\begin{figure}[!htb]
  \centering
  \begin{subfigure}[t]{0.49\textwidth}
    \includegraphics[width=0.98\textwidth]{normal_paas.pdf}
    \caption{Prediction As a Service}
  \end{subfigure}
  \begin{subfigure}[t]{0.49\textwidth}
    \includegraphics[width=0.98\textwidth]{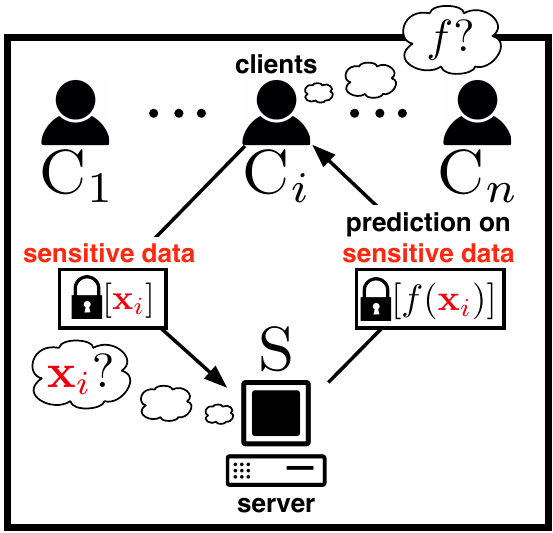}
    \caption{Prediction As a Service}
  \end{subfigure}
  \caption{Normal and Encrypted Prediction As a Service}
  \label{fig:paas-epaas}
\end{figure}
