# Supplementary material for: Identifying and Exploiting Structures for Reliable Deep Learning
Source: arXiv:2108.07083 source file (2021-08-16)
Supplement: Supplementary file 2 [file appendix_gen_bounds.tex]

\subsection*{Adversarial Robustness of LR Networks}
\label{sec:advers-robustn-lr}

The figure below shows the performance of ResNet~\citep{HZRS:2016} and the modified LR ResNet from~\citet{Sanyal2018} on two different attacks; the dotted lines represent the F-LR, which is a factored linear model, with same colour coding as other models for low-rank layer placement, the dashed line represents a black box attack on the same model. Below we plot certain properties of these networks and observe that higher adversarial robustness has a positive correlation with these structures, which in turn have a positive correlation with the generalisation bounds from ~\citet{bartlett2017spectrally} and~\citet{arora18b}.

\begin{center}
\begin{figure}[!h]
	\begin{subfigure}[c]{0.2\textwidth}
		\includegraphics[width=\textwidth]{legend.pdf}
	\end{subfigure}
	\begin{subfigure}[c]{0.38\textwidth}
		\includegraphics[width=0.95\textwidth, trim={0cm, 0cm, 0cm, 0cm}, clip]{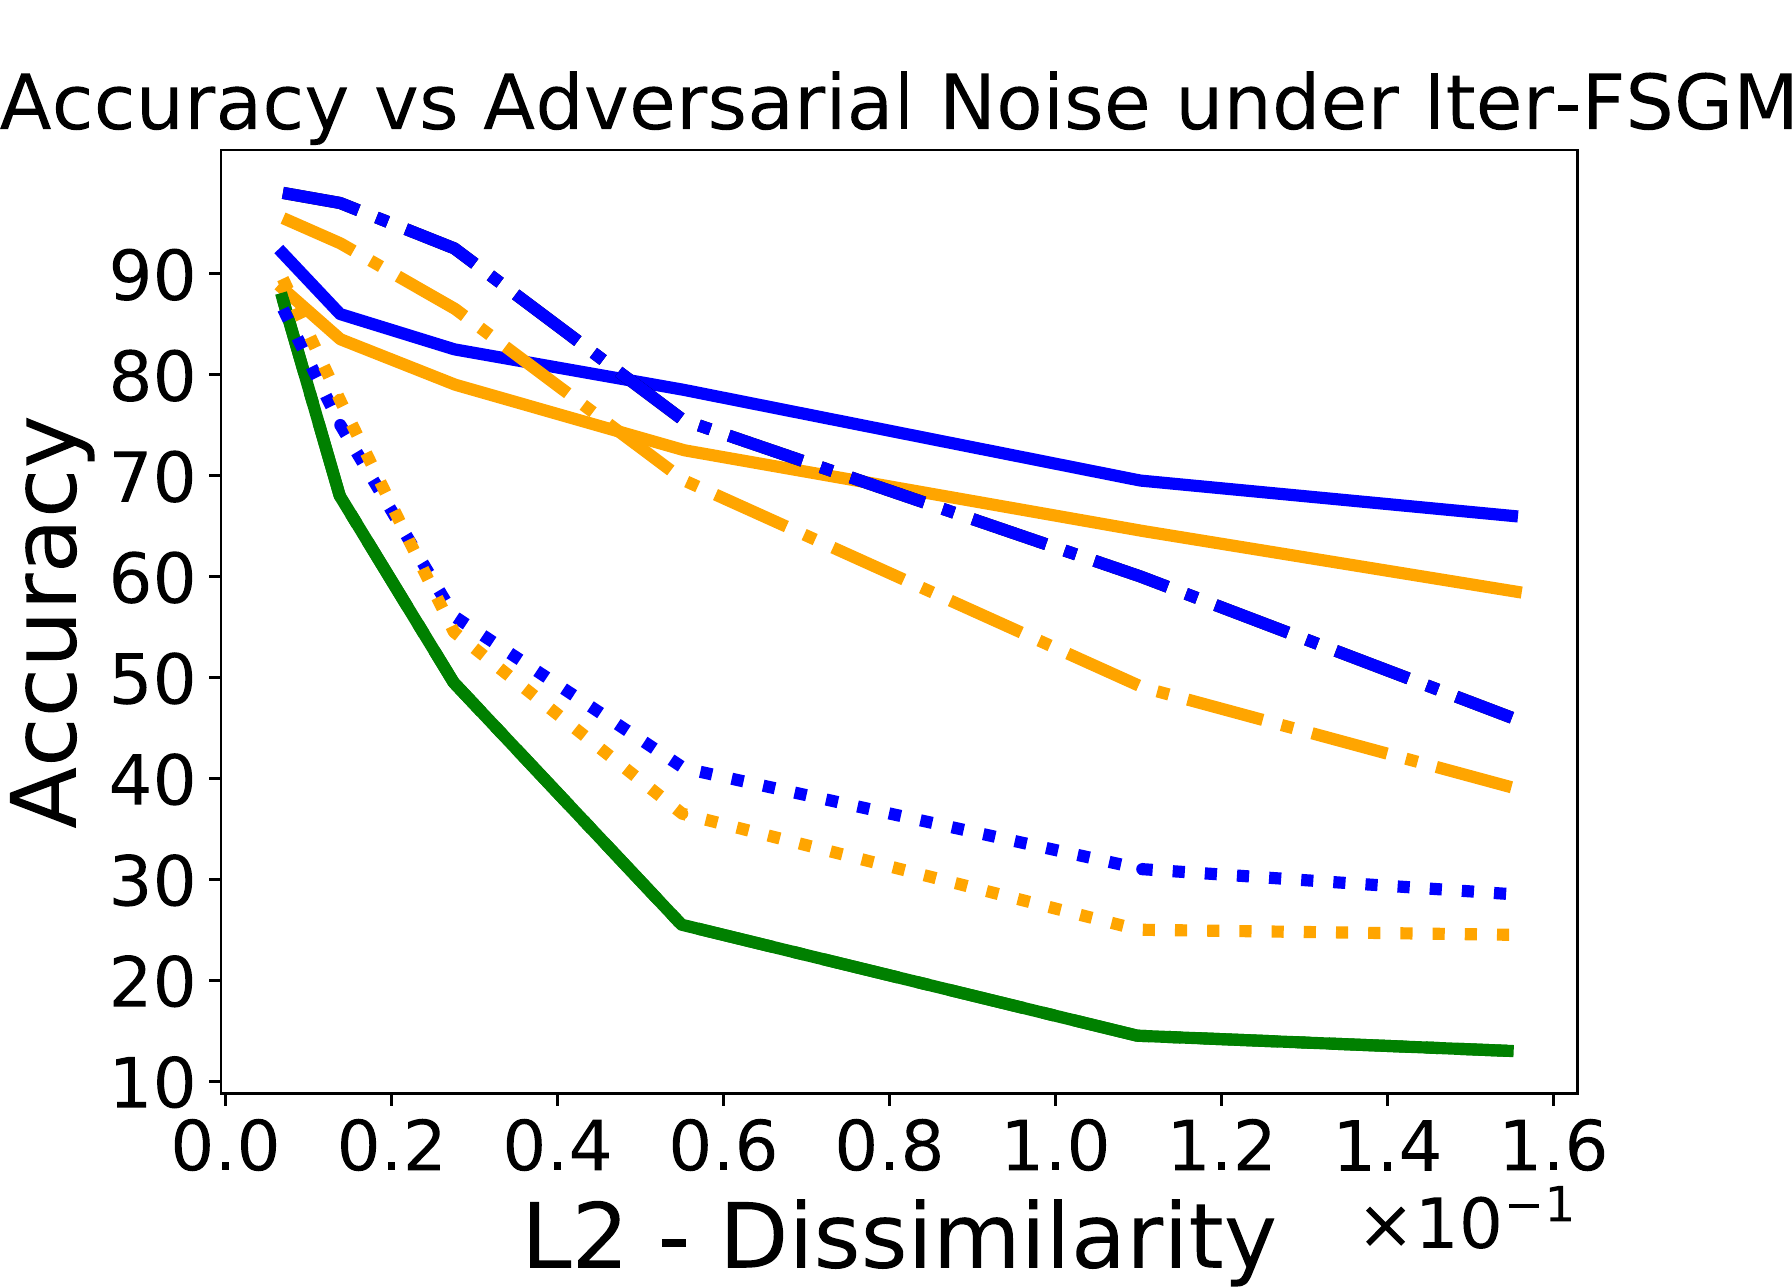}
	\end{subfigure}
	\begin{subfigure}[c]{0.38\textwidth}
		\includegraphics[width=0.99\textwidth, clip]{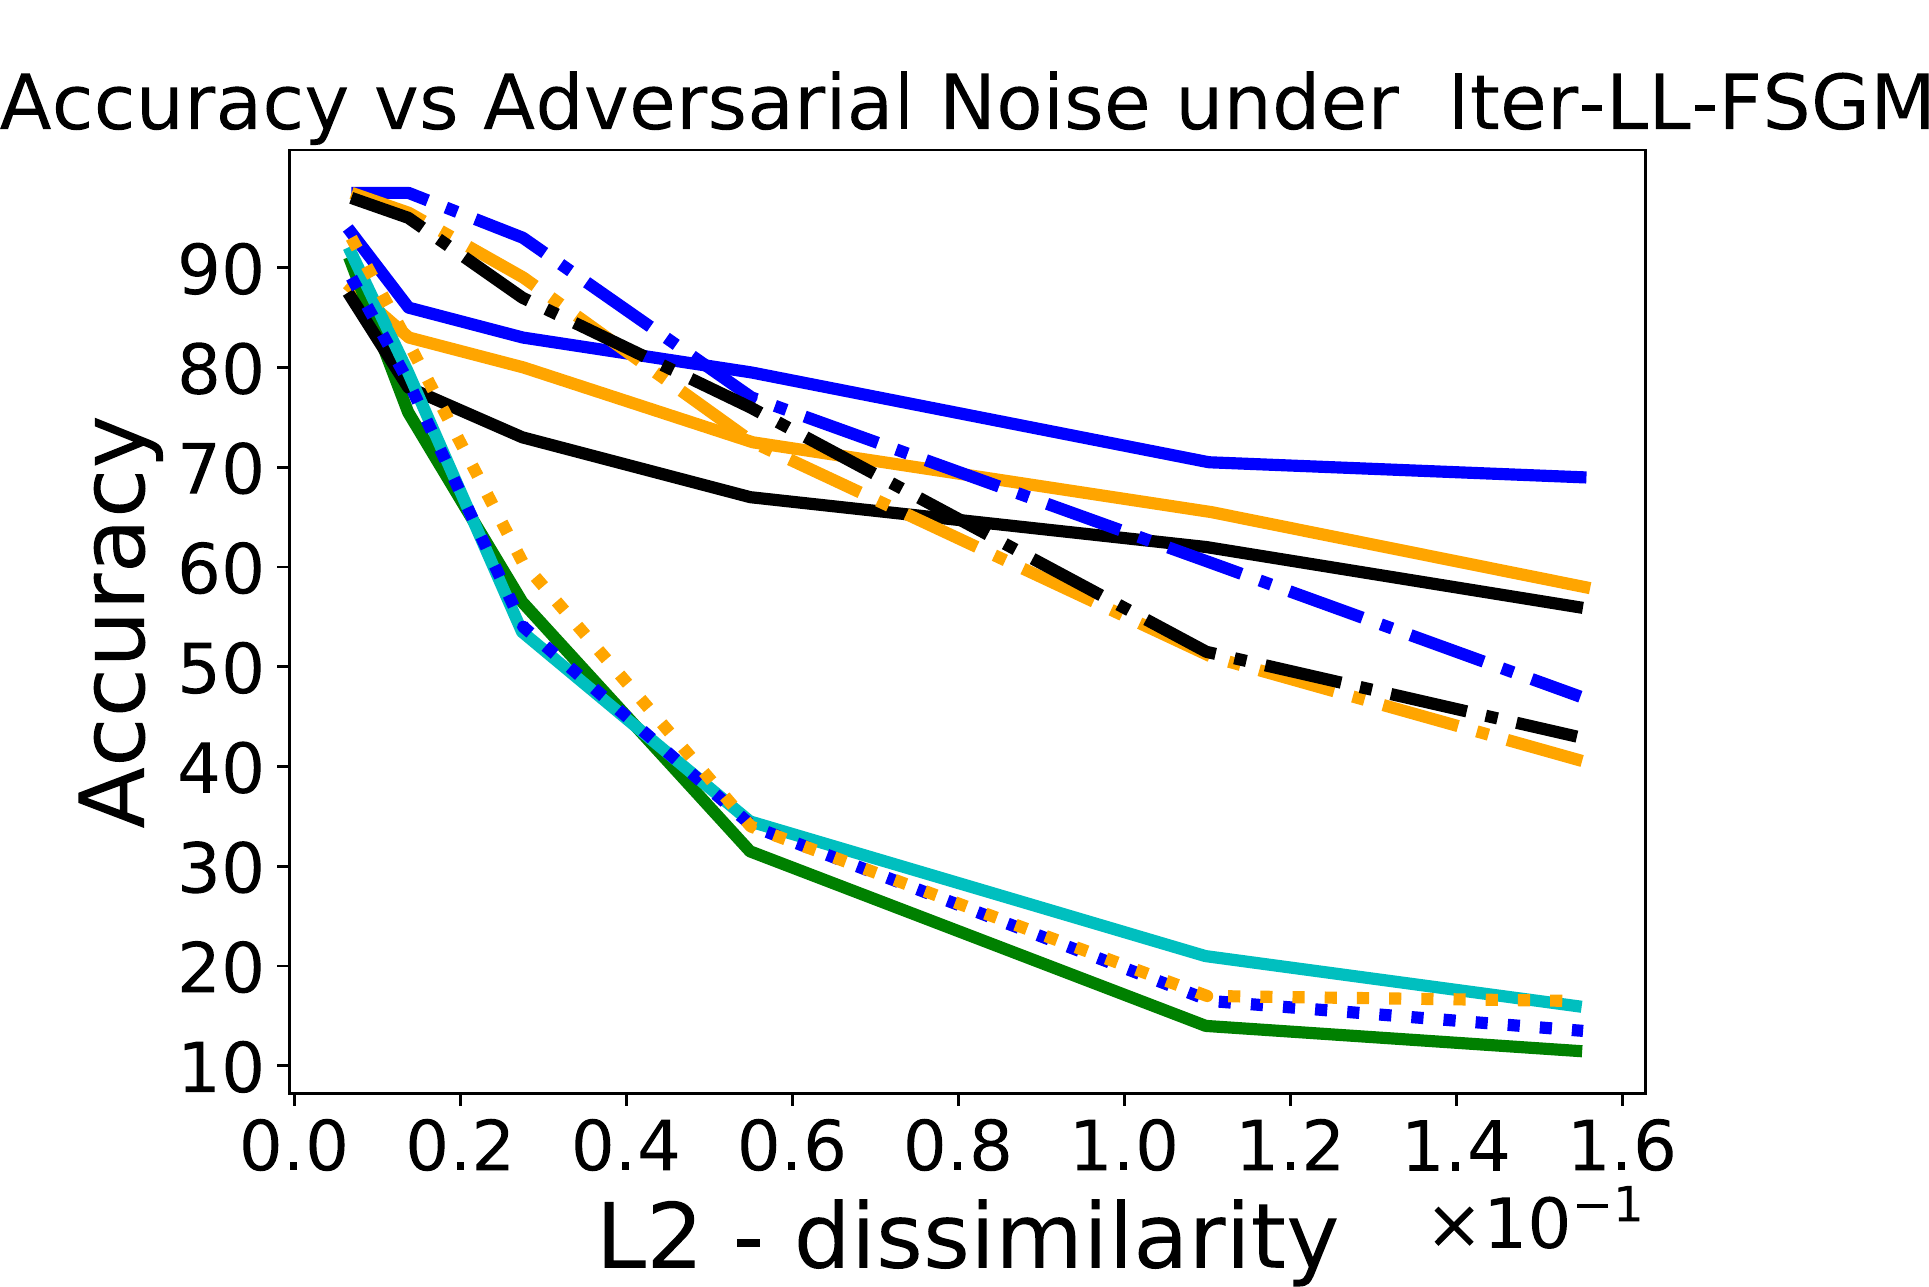}
              \end{subfigure}
              \caption{Adversarial Robustness of LR models}
              \label{fig:adversarial-robust-lr-model}
\end{figure}
\end{center}

\subsection{Layer Cushion}
\label{sec:layer-cushion}

Here we plot the \textit{layer cushion} quantities for various layers
in ResNet. The quantity was  first mentioned in~\citet{arora18b}. We look
at ResNet models from ~\citet{Sanyal2018}, normal ResNet~\citep{HZRS:2016} and randomly
initialized ResNet.

For any layer $i$, the layer cushion is defined as the largest
number $\mu_i$  such that the following holds for all examples
$\vec{x}\in \cS$ where $\cS$ is the training set.

\[ \mu_i\norm{\vec{A}_i}_F\norm{\phi\br{\vec{x}_{i-1}}} \le
  \norm{\vec{A}_i\phi\br{\vec{x}_{i-1}}}\]
$\vec{A}_i$ is the weight matrix of the $i^{\it{th}}$ layer,
$\vec{x}_i$ is the pre-activation of the layer and $\phi$ is the
activation function. As observed i~\citet{arora18b}, higher the value
of $\mu_i$, better is the generalisation ability of the model. 

  \begin{figure}[h!]
    \begin{subfigure}[c]{0.245\linewidth}
    \centering
    \def\svgwidth{0.99\columnwidth}
    \input{./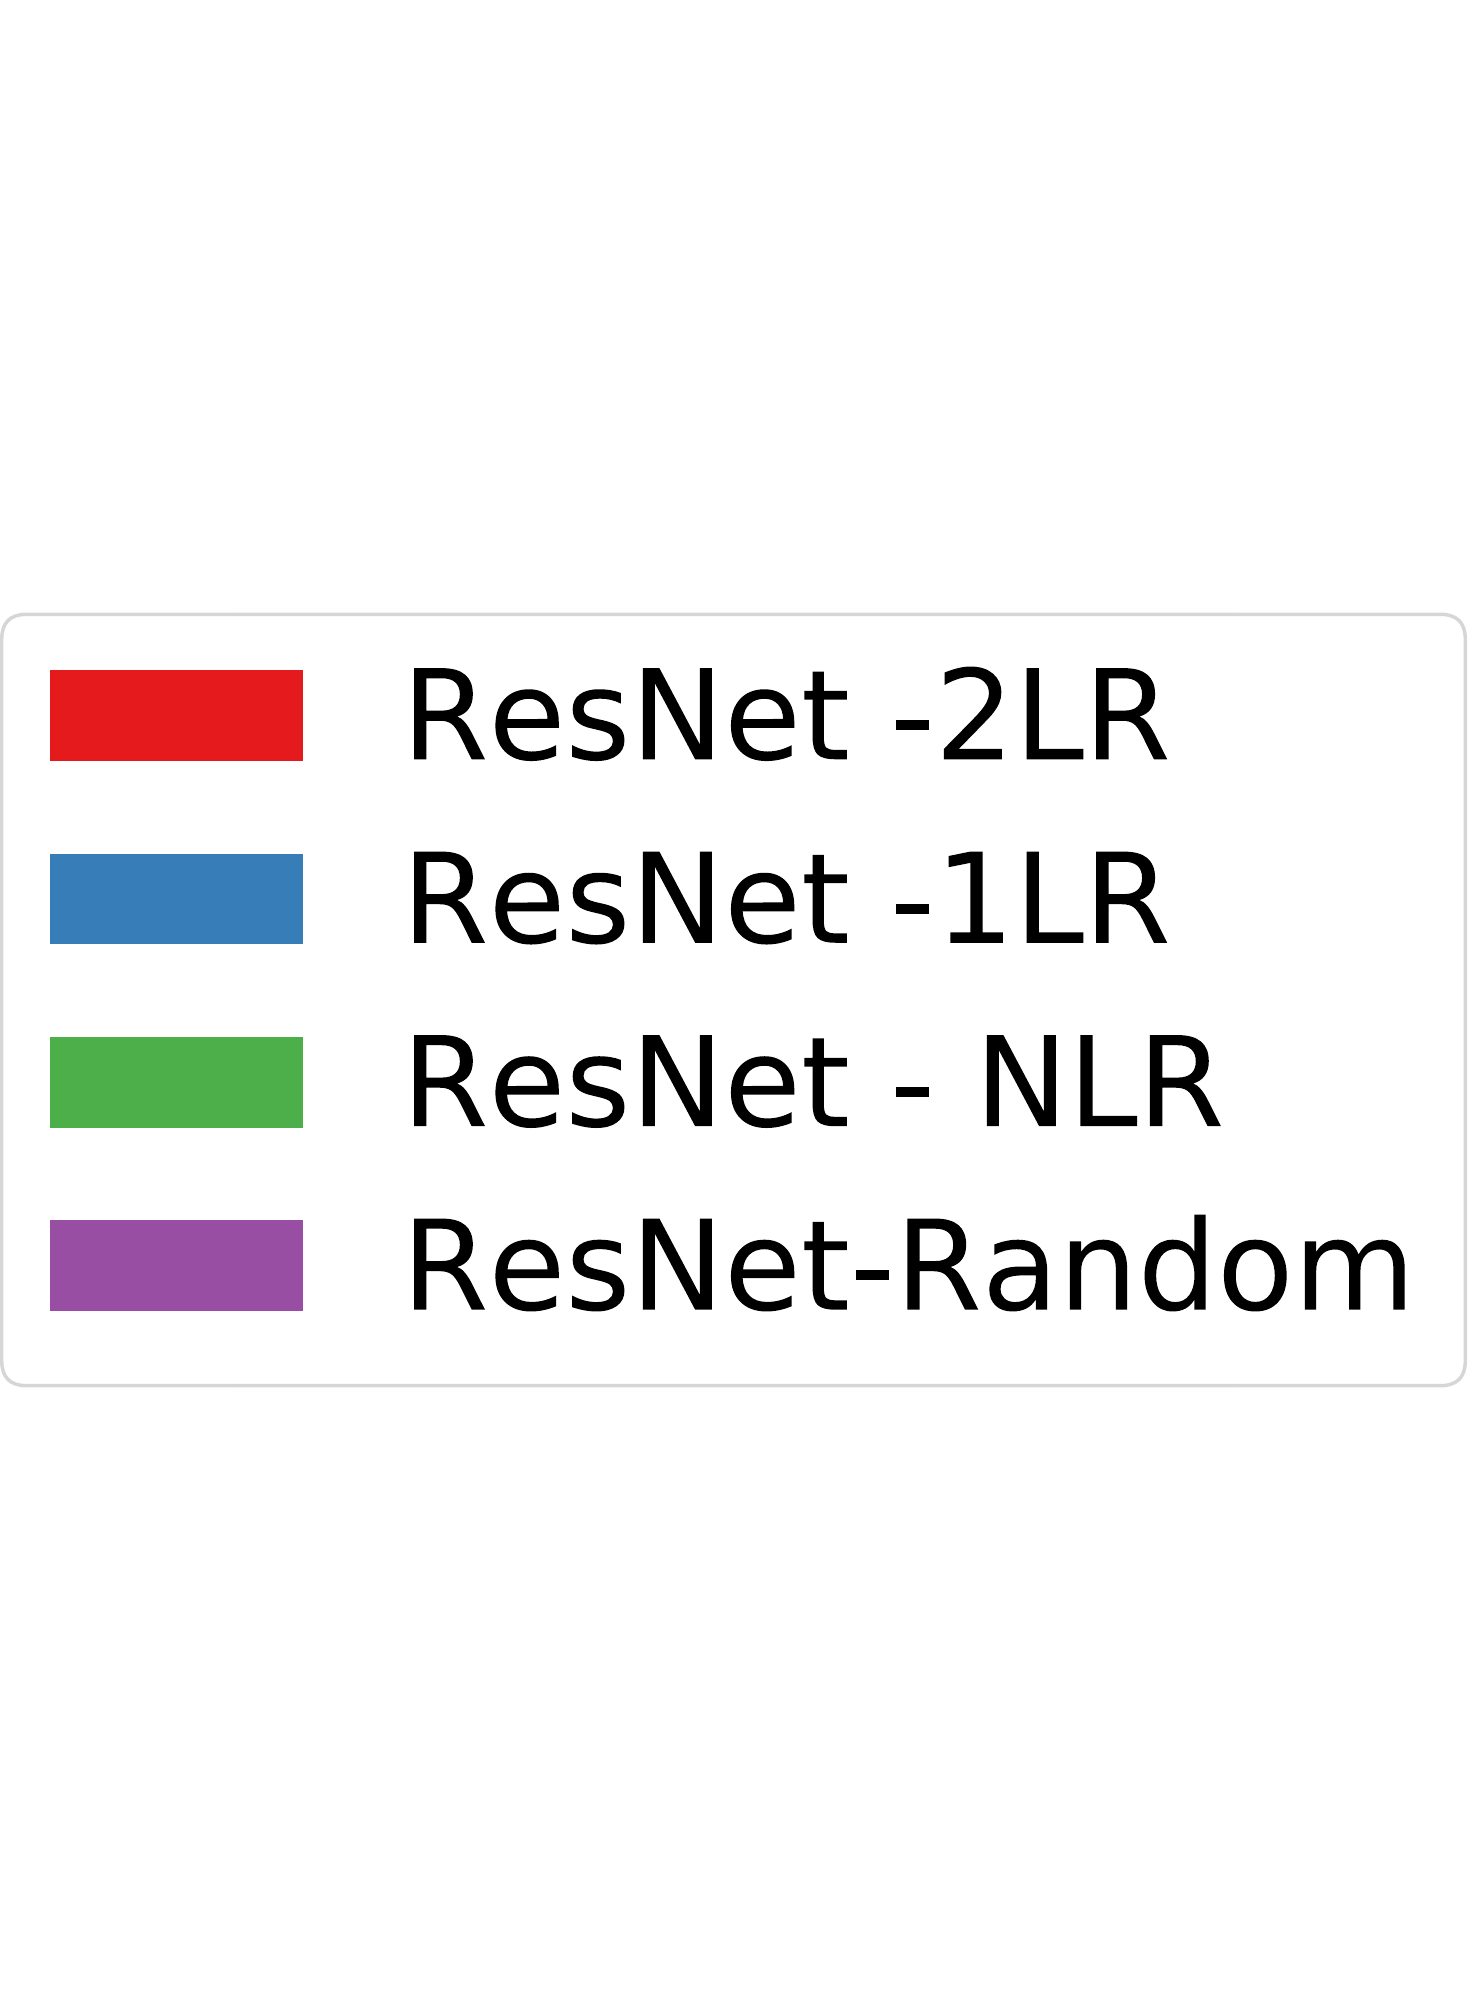_tex}
  \end{subfigure}\hfill
  \begin{subfigure}[c]{0.45\linewidth}
    \centering
    \def\svgwidth{0.99\columnwidth}
    \input{./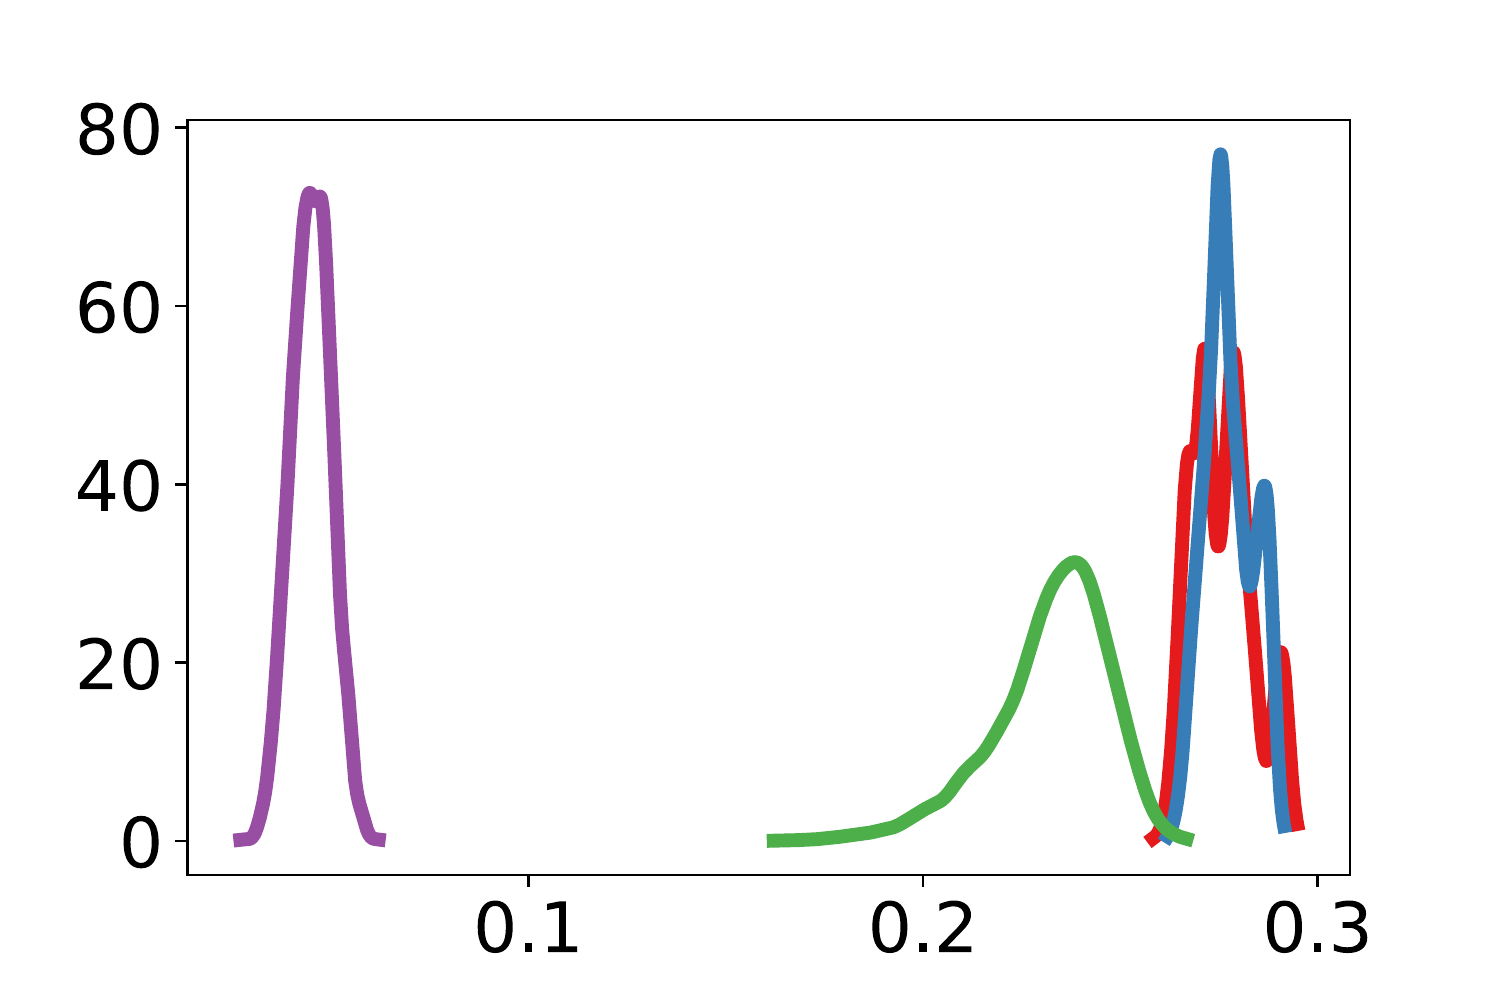_tex}
  \end{subfigure}\caption{The last fully connected layer of Resnet.}
  \end{figure}

 The following correspond to ResNet blocks. Each block has two smaller
 sub-blocks where each sub-block has two convolutional layers. The
 value of layer cushion for these modules of one block are plotted below.

\begin{center}
  \begin{figure}[h!]
  \begin{subfigure}[c]{0.245\linewidth}
    \centering
    \def\svgwidth{0.99\columnwidth}
    \input{./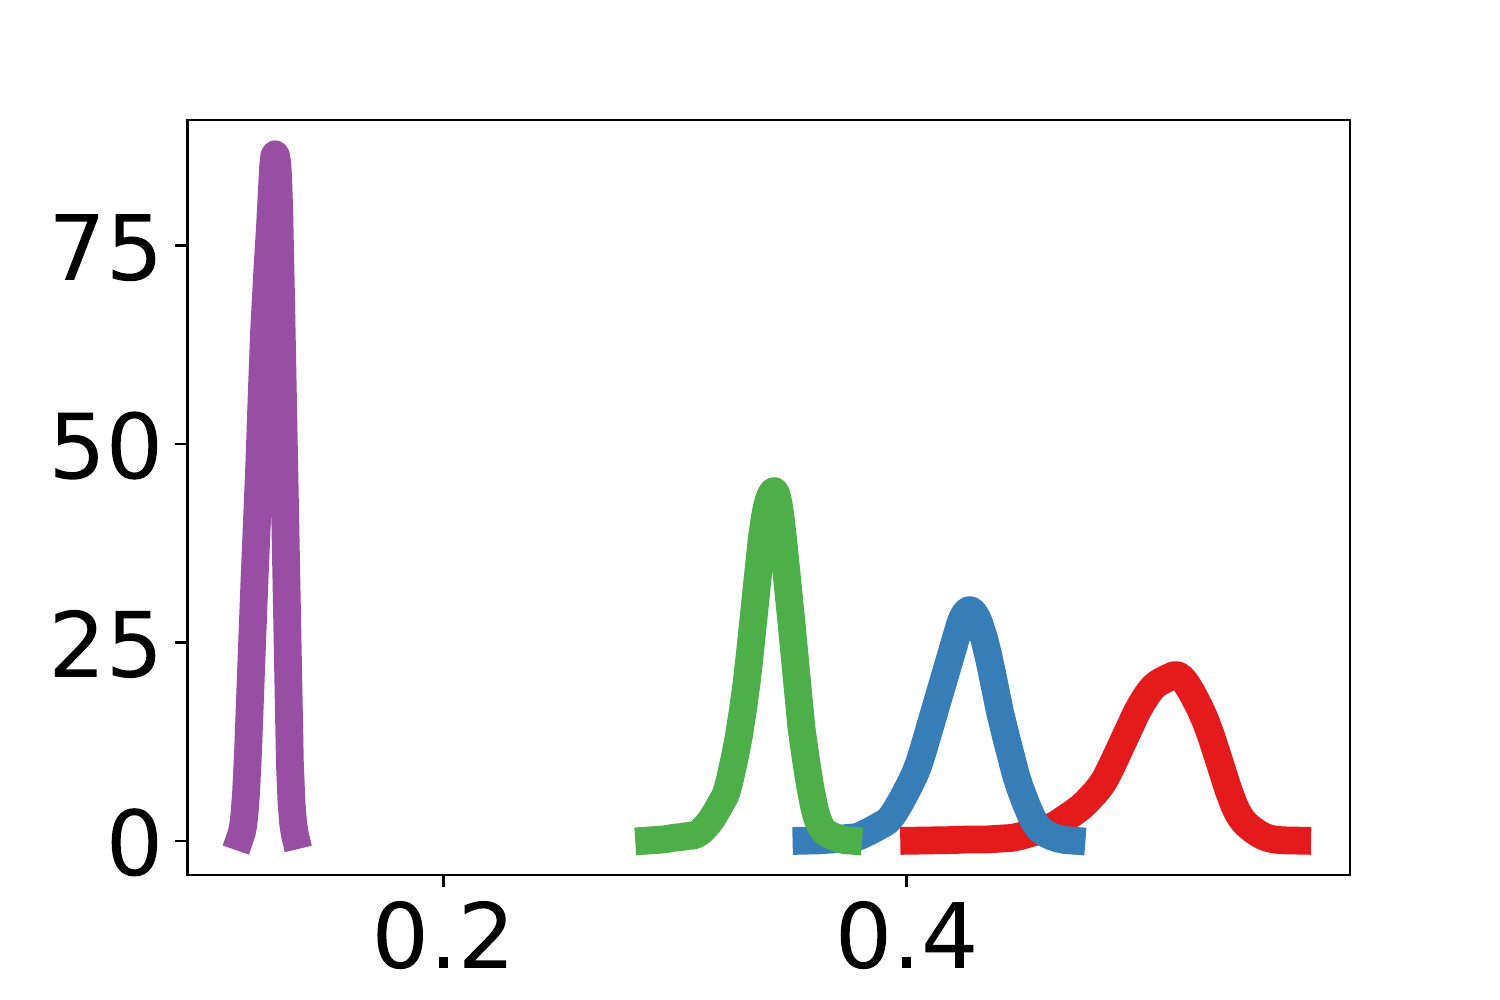_tex}
  \end{subfigure}
  \begin{subfigure}[c]{0.245\linewidth}
    \centering
    \def\svgwidth{0.99\columnwidth}
    \input{./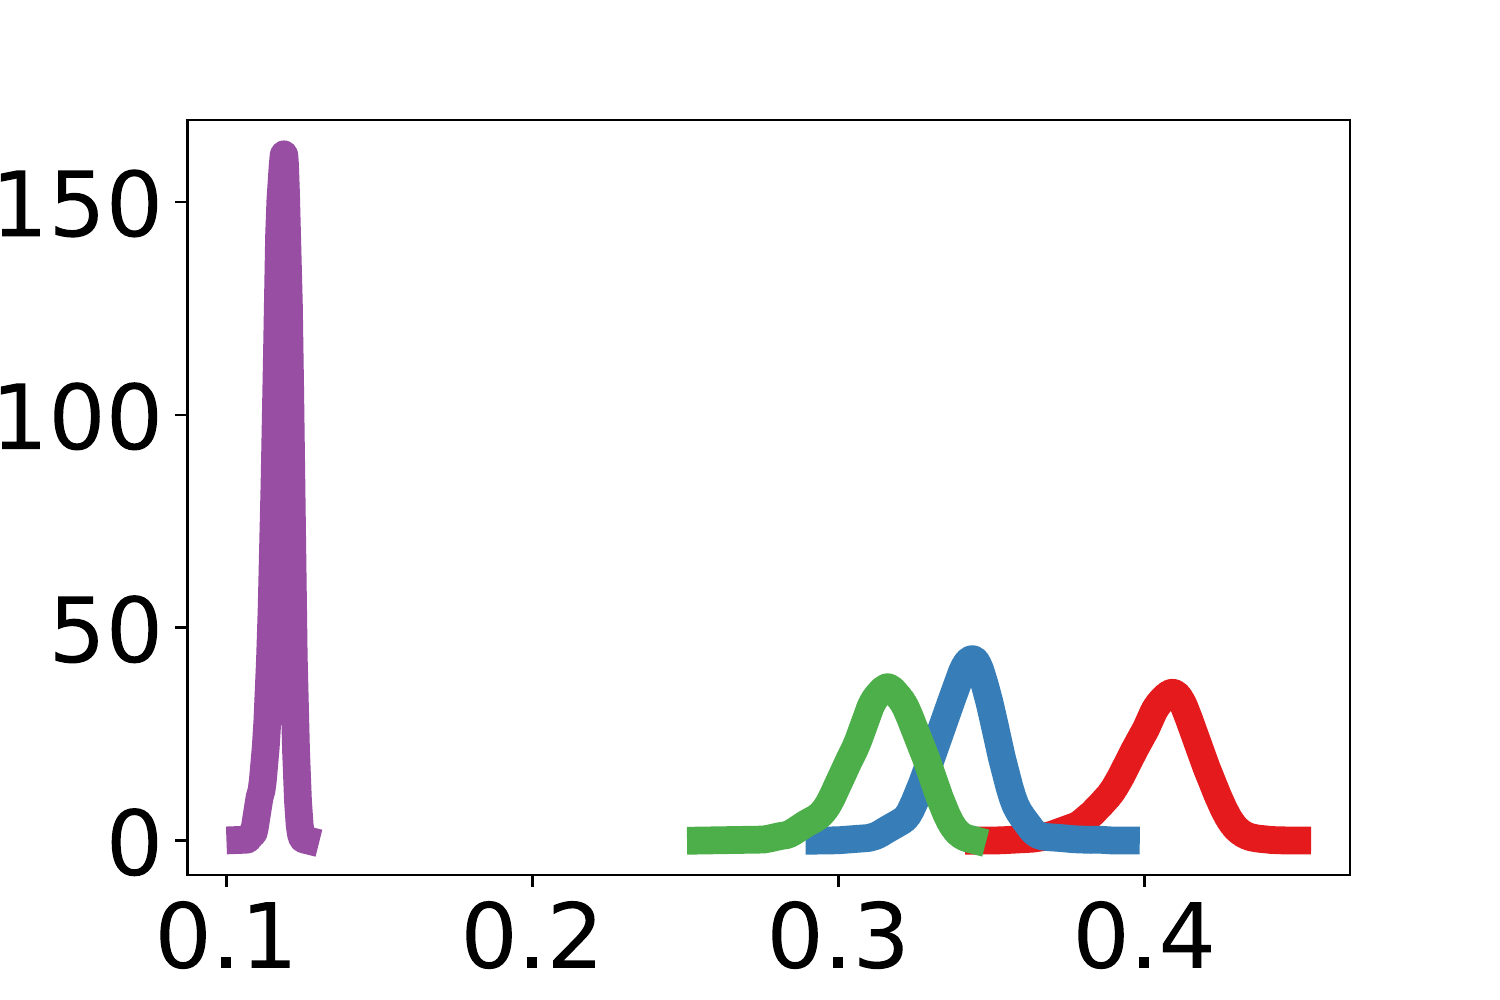_tex}
  \end{subfigure}
  \begin{subfigure}[c]{0.245\linewidth}
    \centering
    \def\svgwidth{0.99\columnwidth}
    \input{./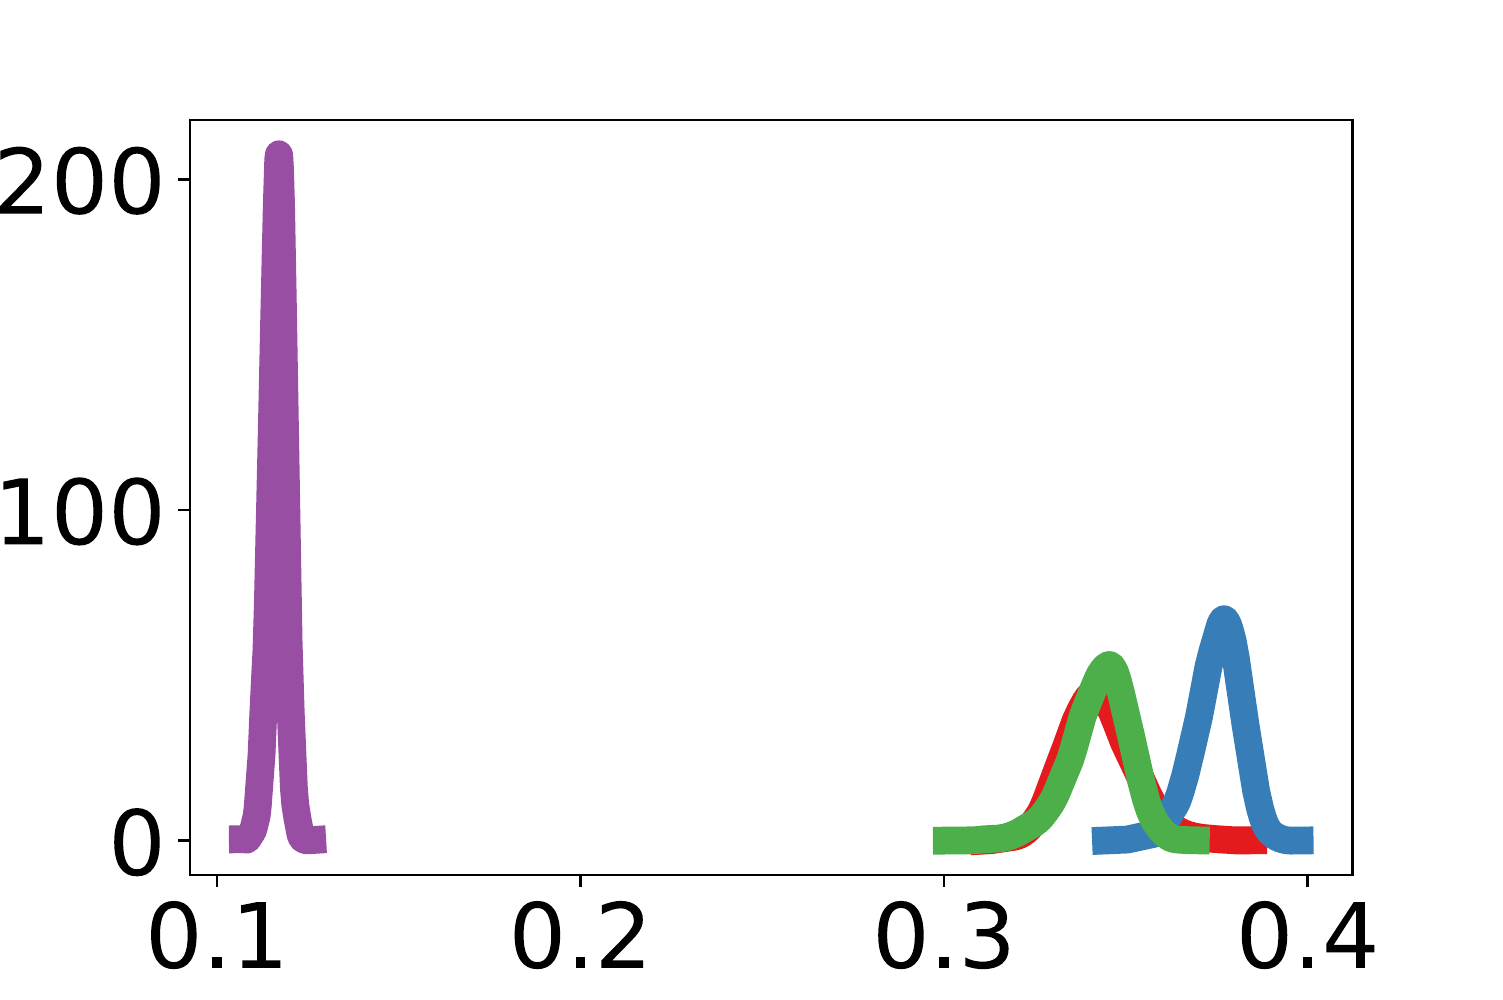_tex}
  \end{subfigure}
  \begin{subfigure}[c]{0.245\linewidth}
    \centering
    \def\svgwidth{0.99\columnwidth}
    \input{./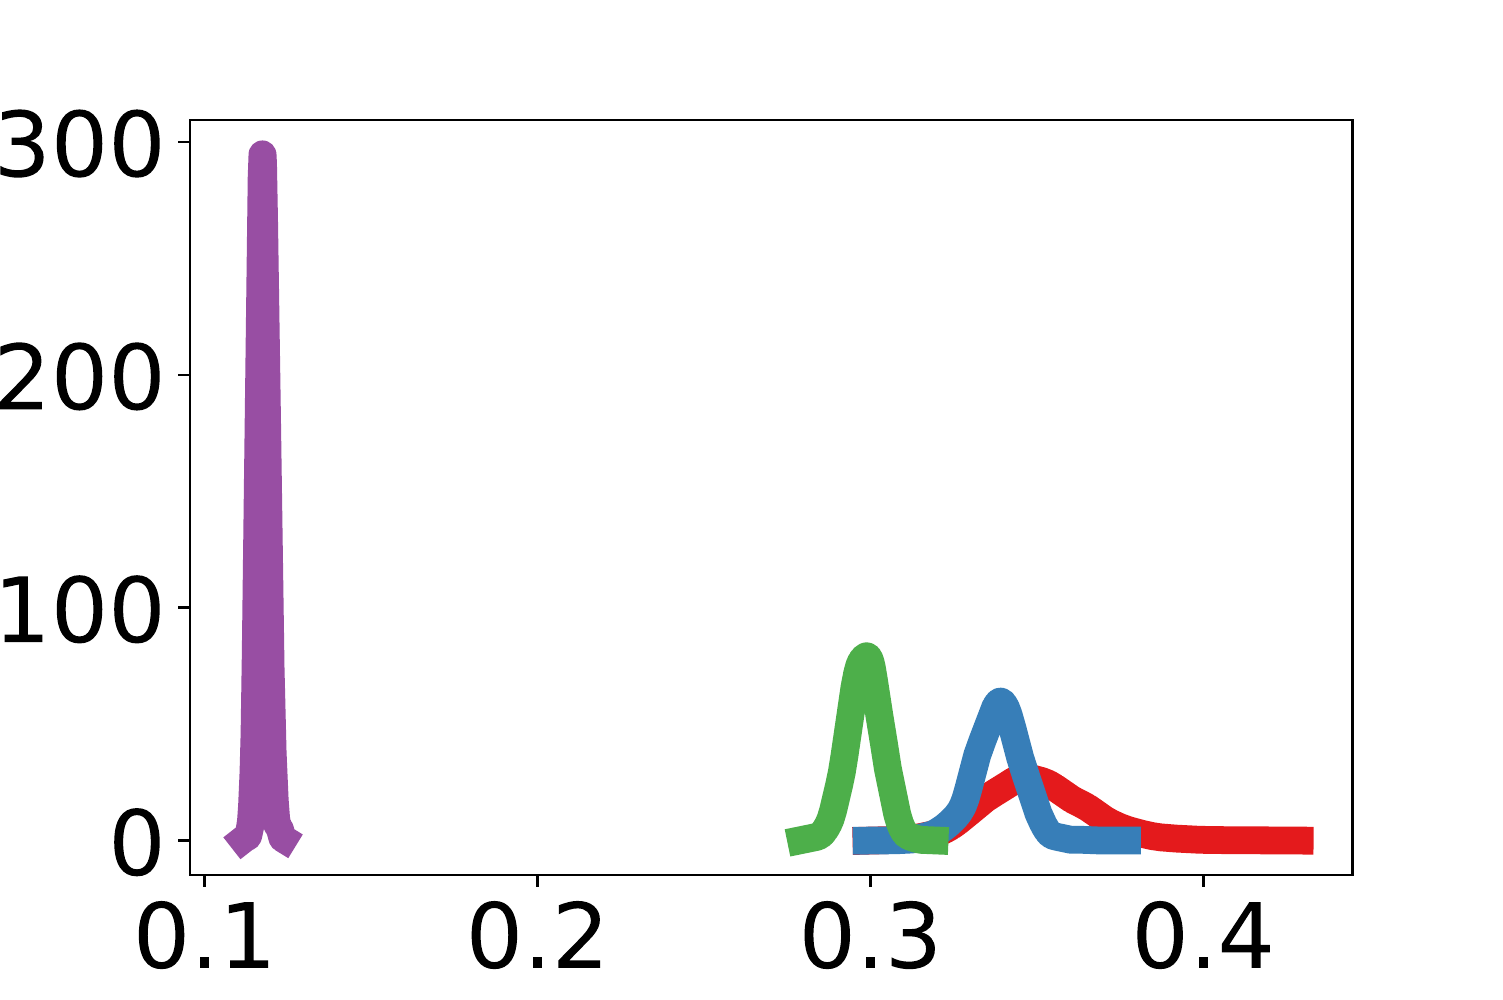_tex}
  \end{subfigure}
  \caption{Layer 1}
  \label{fig:int_lyr_cush}
\end{figure}
\end{center}

\begin{center}
  \begin{figure}[h!]
  \begin{subfigure}[c]{0.245\linewidth}
    \centering
    \def\svgwidth{0.99\columnwidth}
    \input{./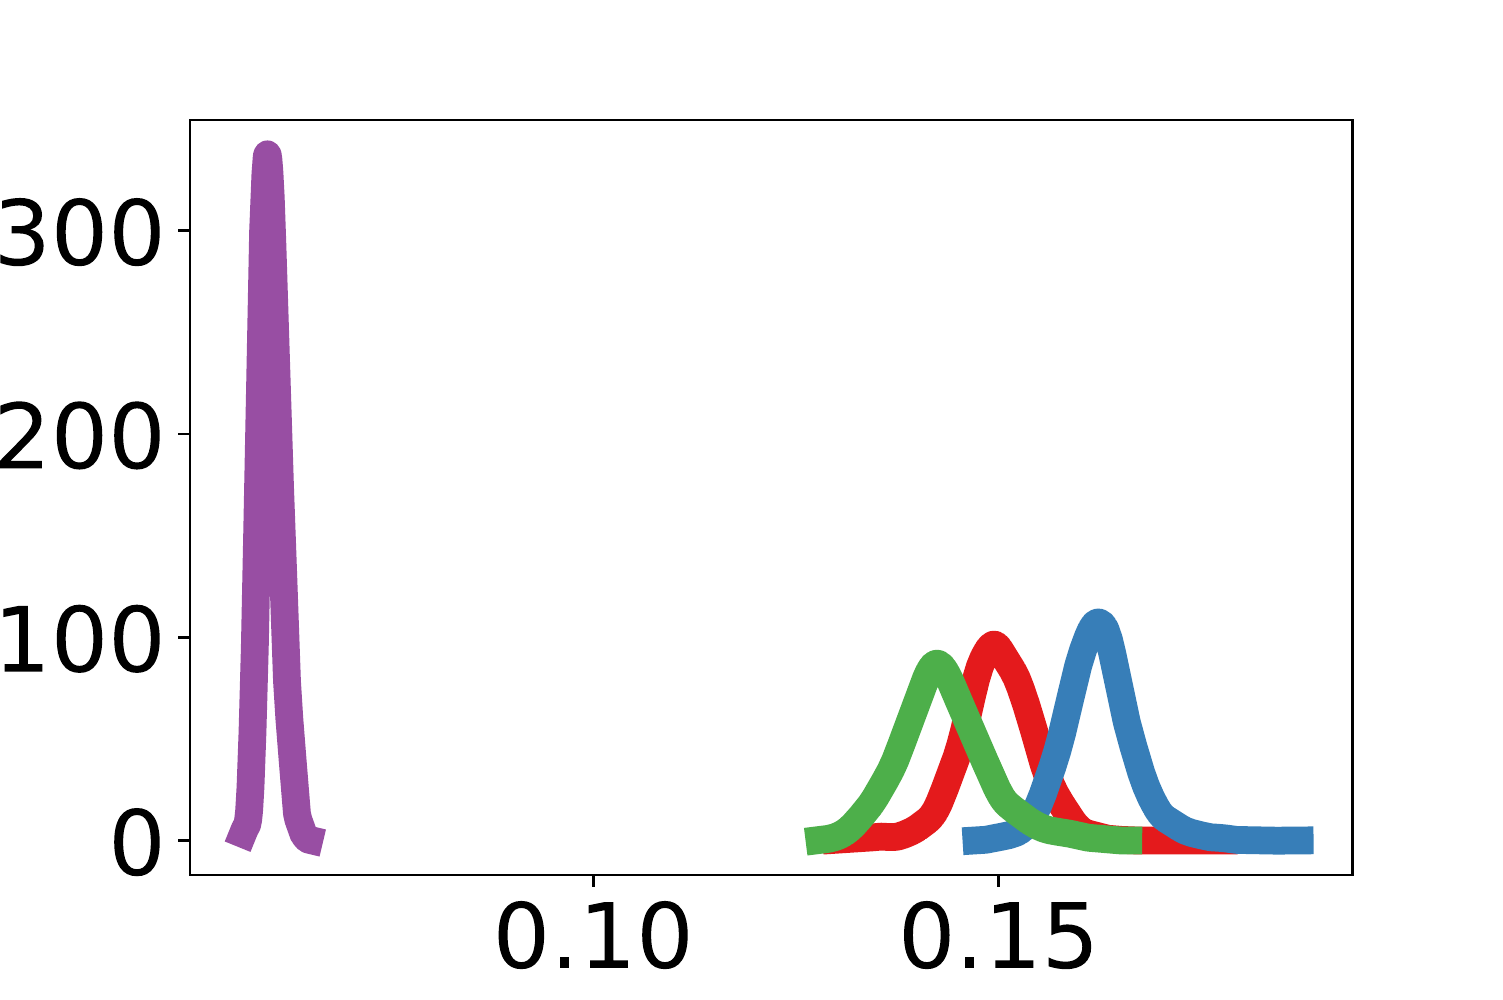_tex}
  \end{subfigure}
  \begin{subfigure}[c]{0.245\linewidth}
    \centering
    \def\svgwidth{0.99\columnwidth}
    \input{./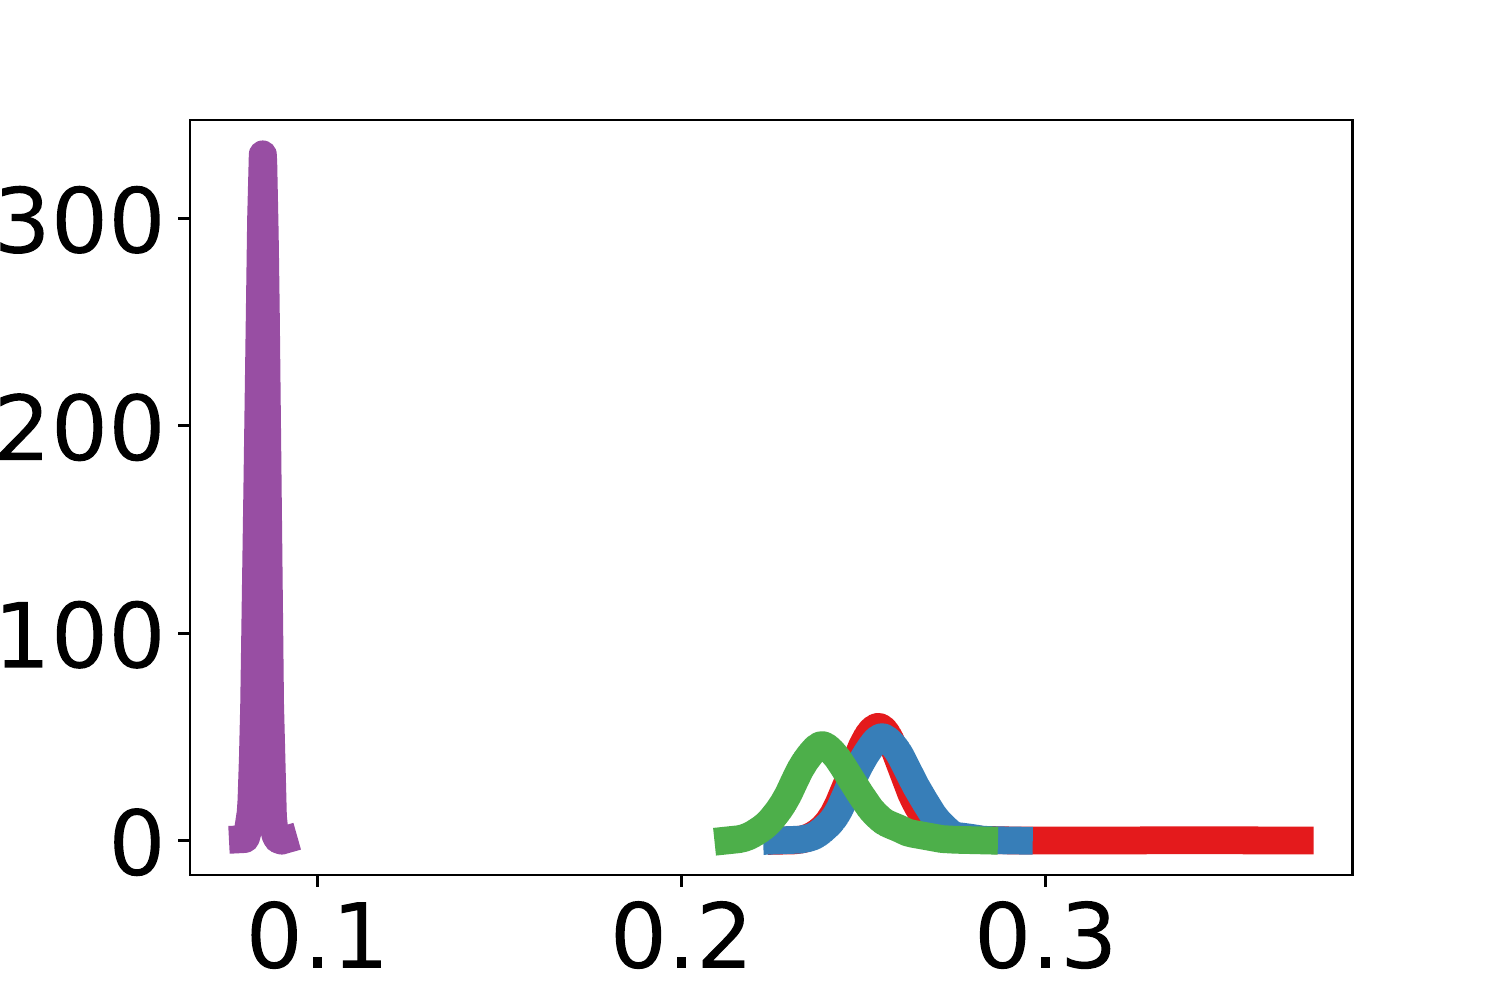_tex}
  \end{subfigure}
  \begin{subfigure}[c]{0.245\linewidth}
    \centering
    \def\svgwidth{0.99\columnwidth}
    \input{./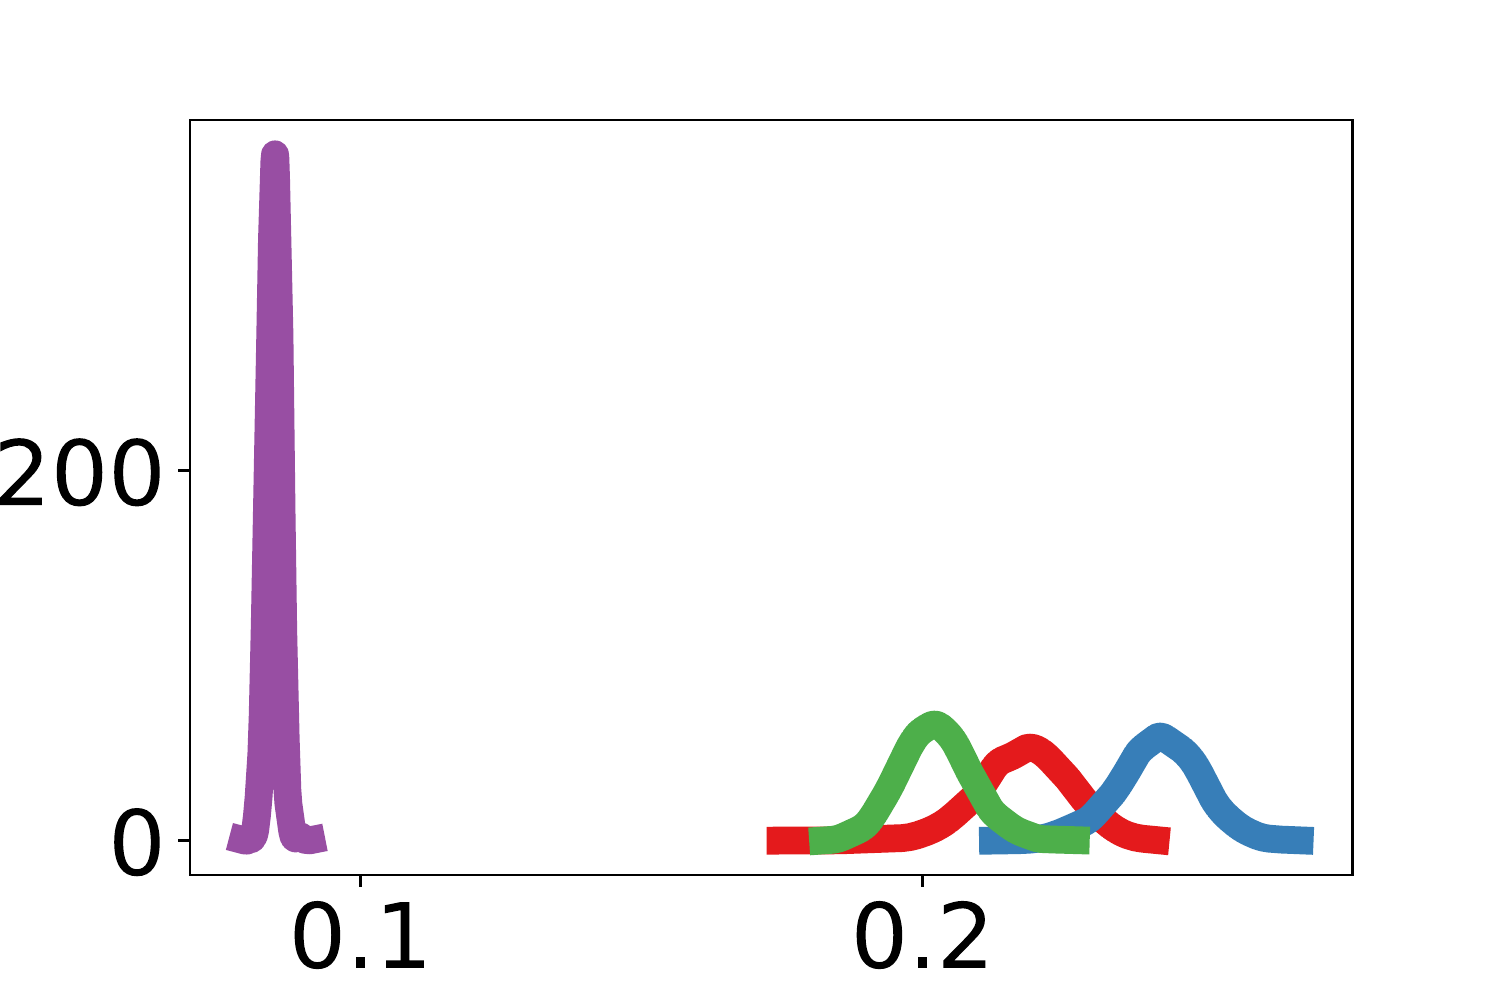_tex}
  \end{subfigure}
  \begin{subfigure}[c]{0.245\linewidth}
    \centering
    \def\svgwidth{0.99\columnwidth}
    \input{./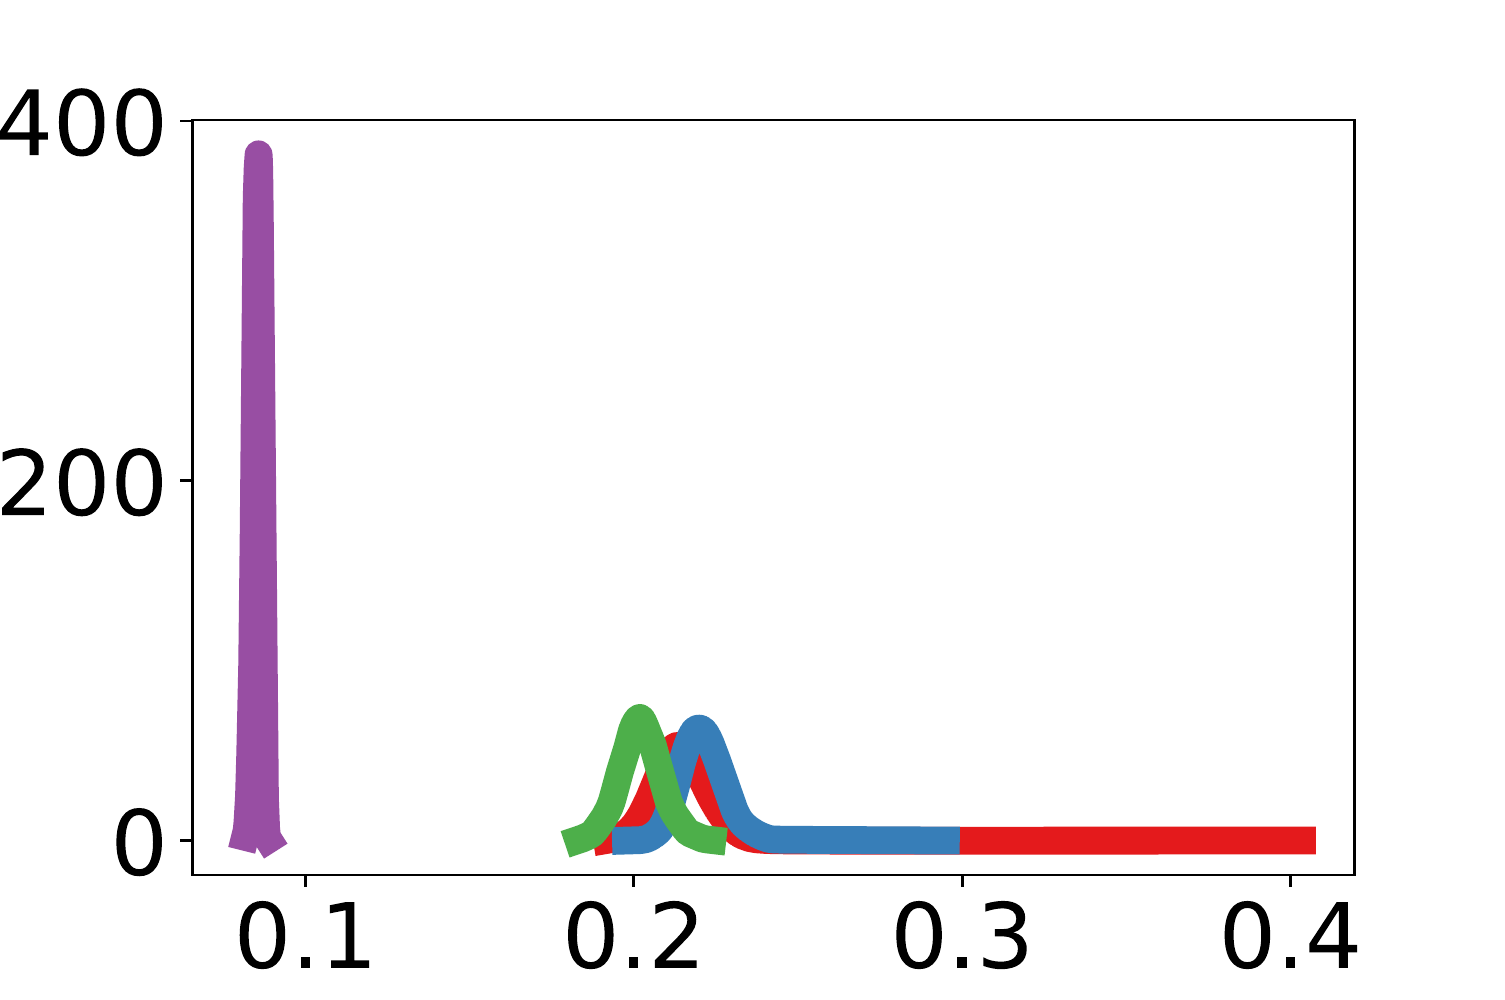_tex}
  \end{subfigure}
  \caption{Layer 2}
  \label{fig:int_lyr2_cush}
\end{figure}
\end{center}

\begin{center}
  \begin{figure}[h!]
  \begin{subfigure}[c]{0.245\linewidth}
    \centering
    \def\svgwidth{0.99\columnwidth}
    \input{./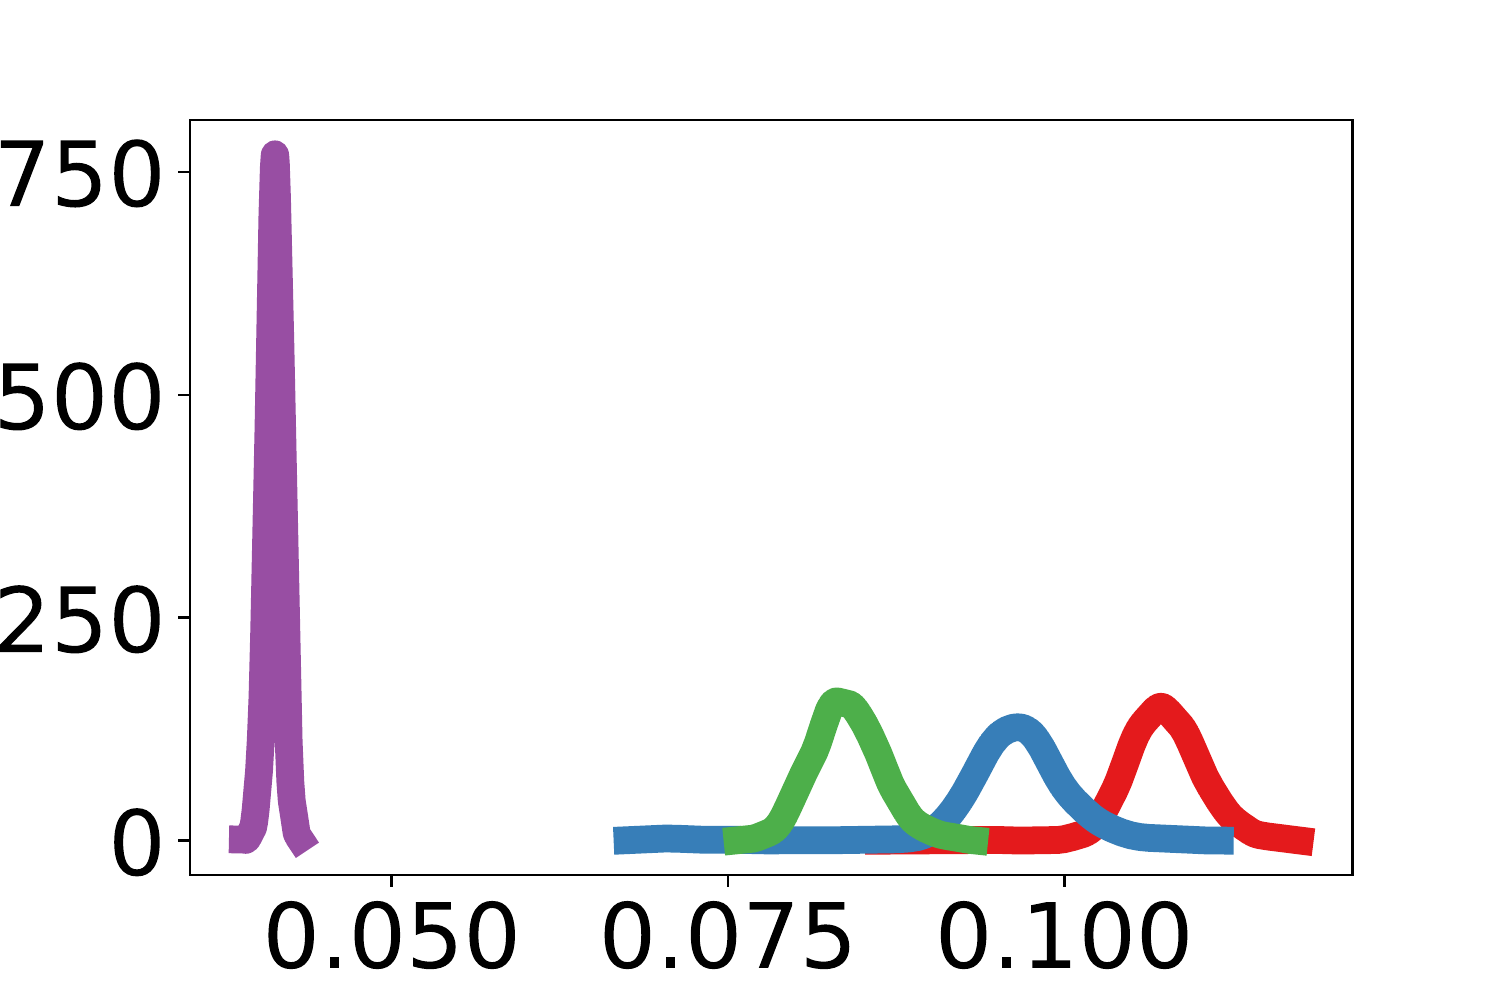_tex}
  \end{subfigure}
  \begin{subfigure}[c]{0.245\linewidth}
    \centering
    \def\svgwidth{0.99\columnwidth}
    \input{./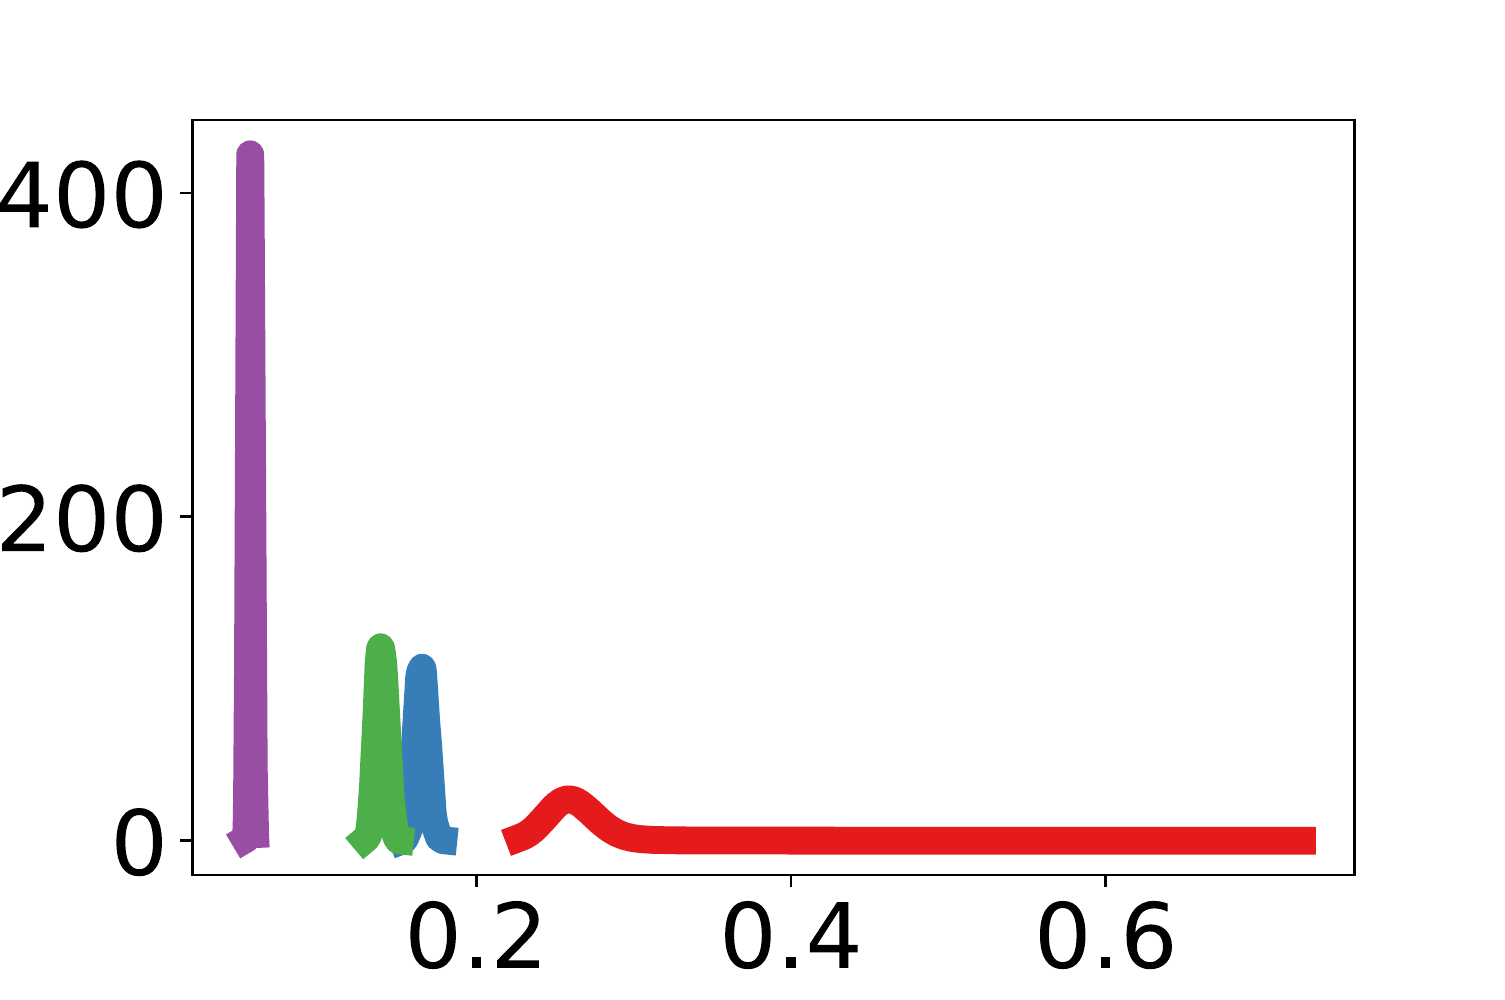_tex}
  \end{subfigure}
  \begin{subfigure}[c]{0.245\linewidth}
    \centering
    \def\svgwidth{0.99\columnwidth}
    \input{./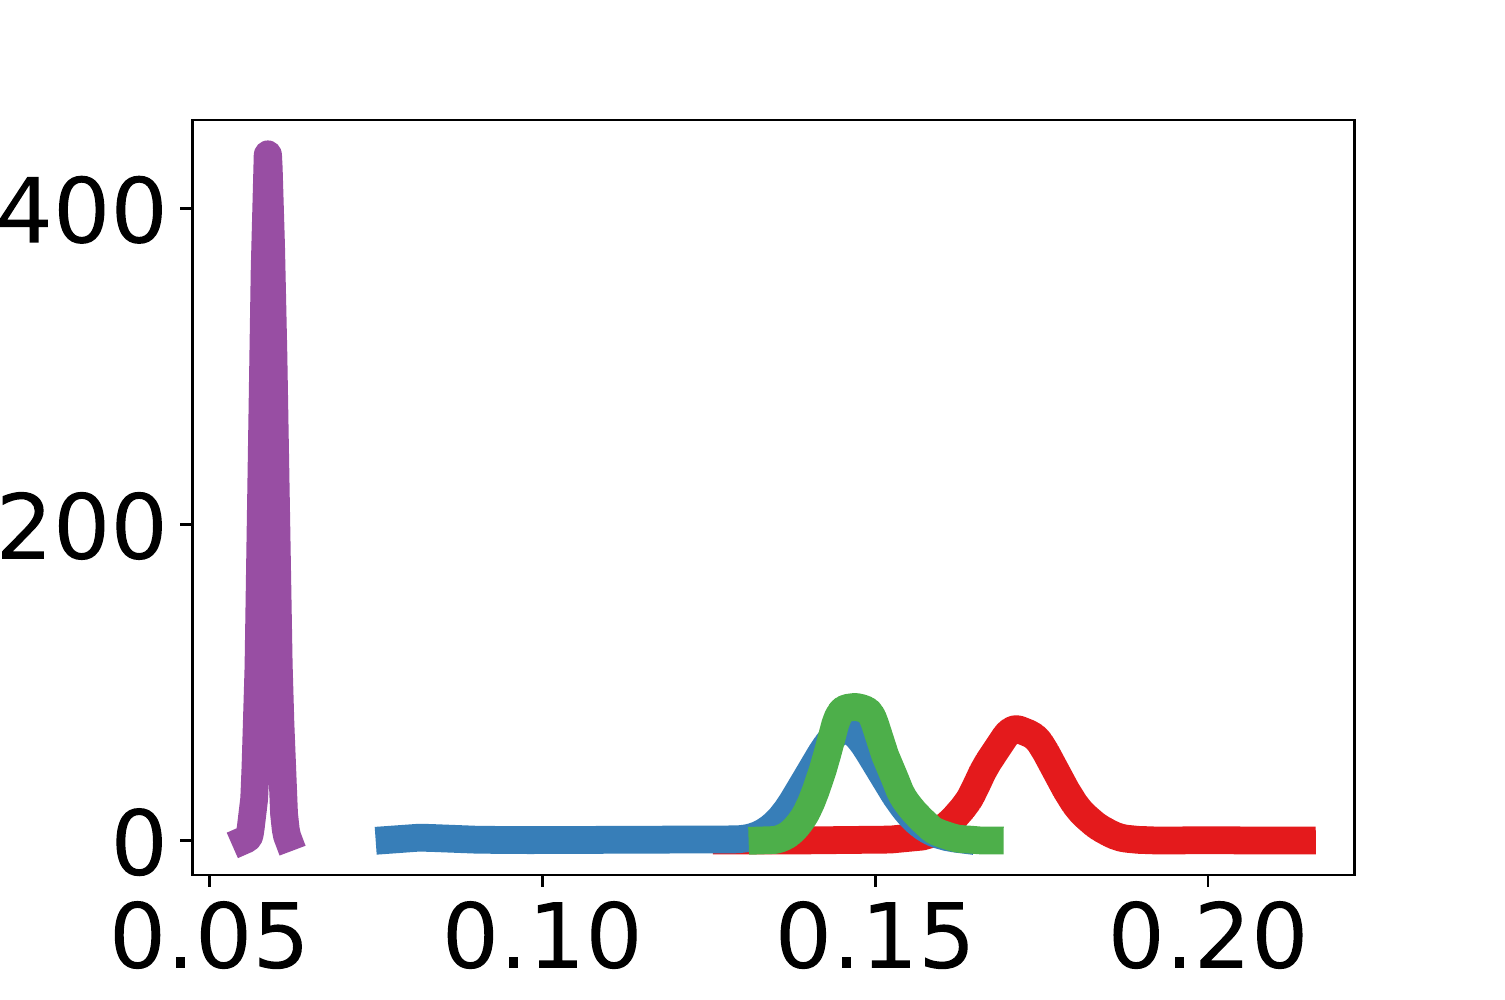_tex}
  \end{subfigure}
  \begin{subfigure}[c]{0.245\linewidth}
    \centering
    \def\svgwidth{0.99\columnwidth}
    \input{./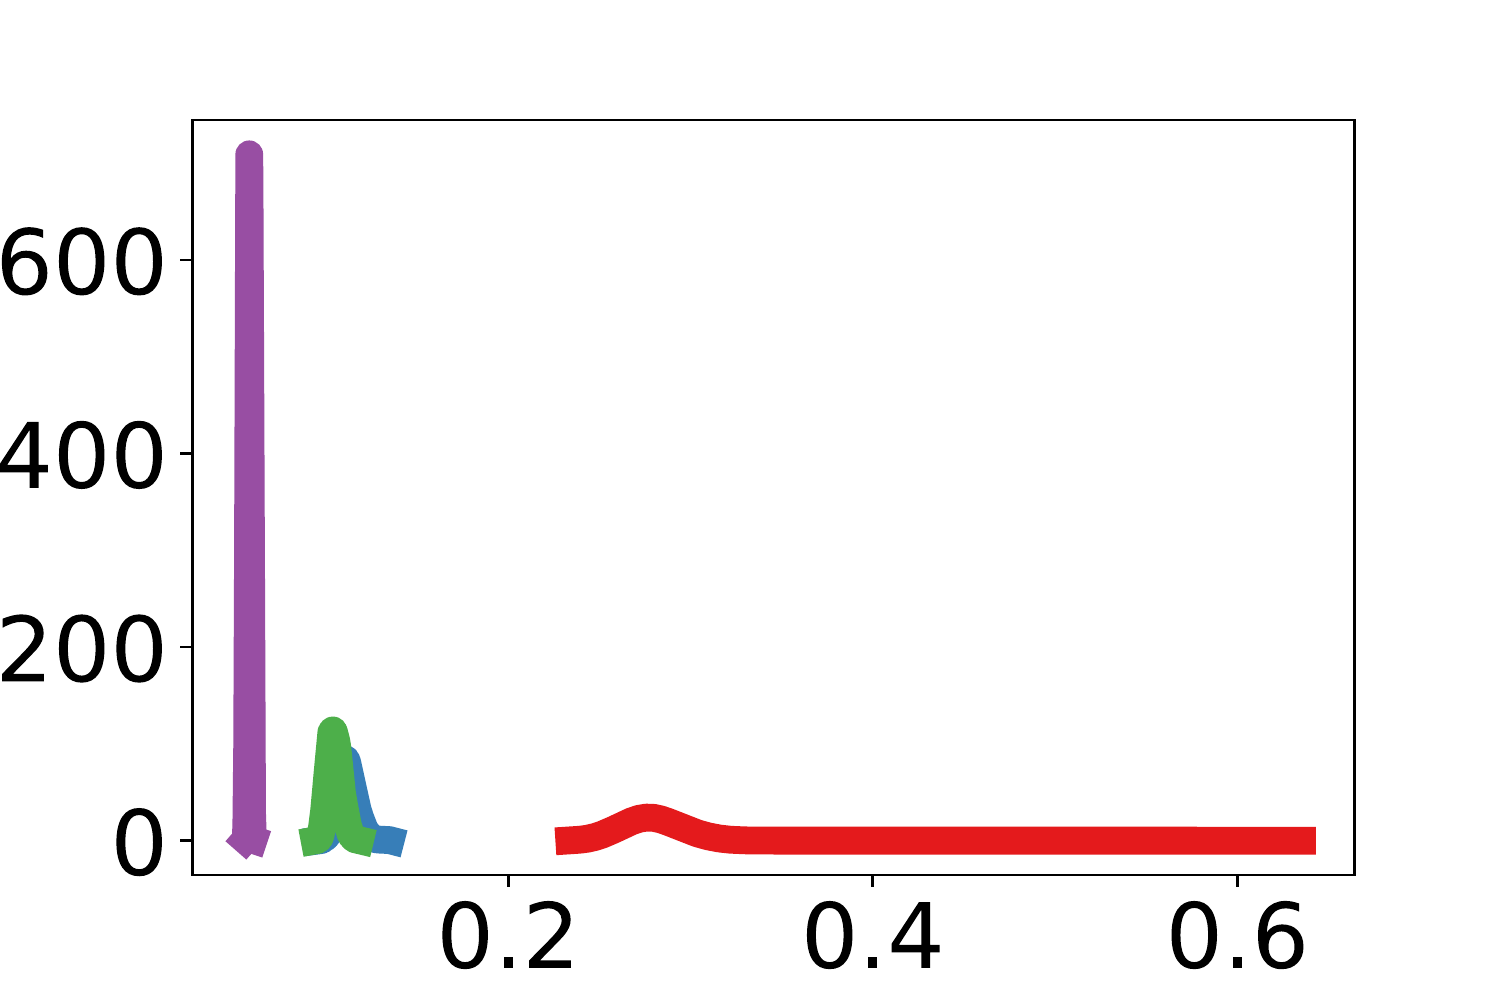_tex}
  \end{subfigure}
  \caption{Layer 3}
  \label{fig:int_lyr3_cush}
\end{figure}
\end{center}
\vspace{-50pt}
  \begin{figure}[h!]
  \begin{subfigure}[c]{0.245\linewidth}
    \centering
    \def\svgwidth{0.99\columnwidth}
    \input{./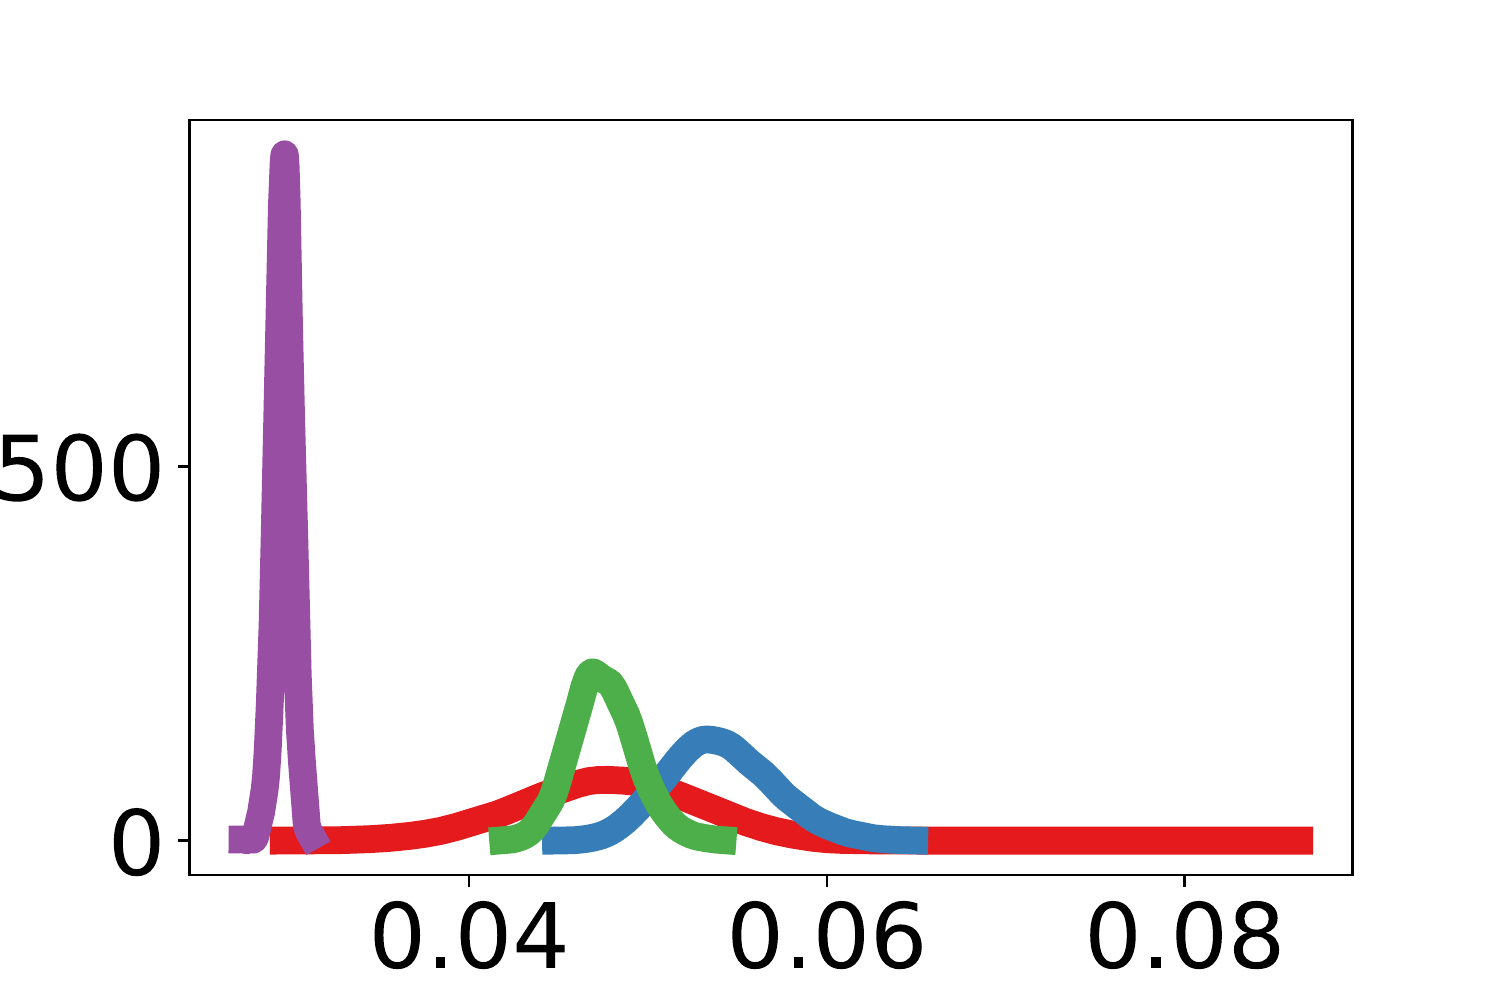_tex}
  \end{subfigure}
  \begin{subfigure}[c]{0.245\linewidth}
    \centering
    \def\svgwidth{0.99\columnwidth}
    \input{./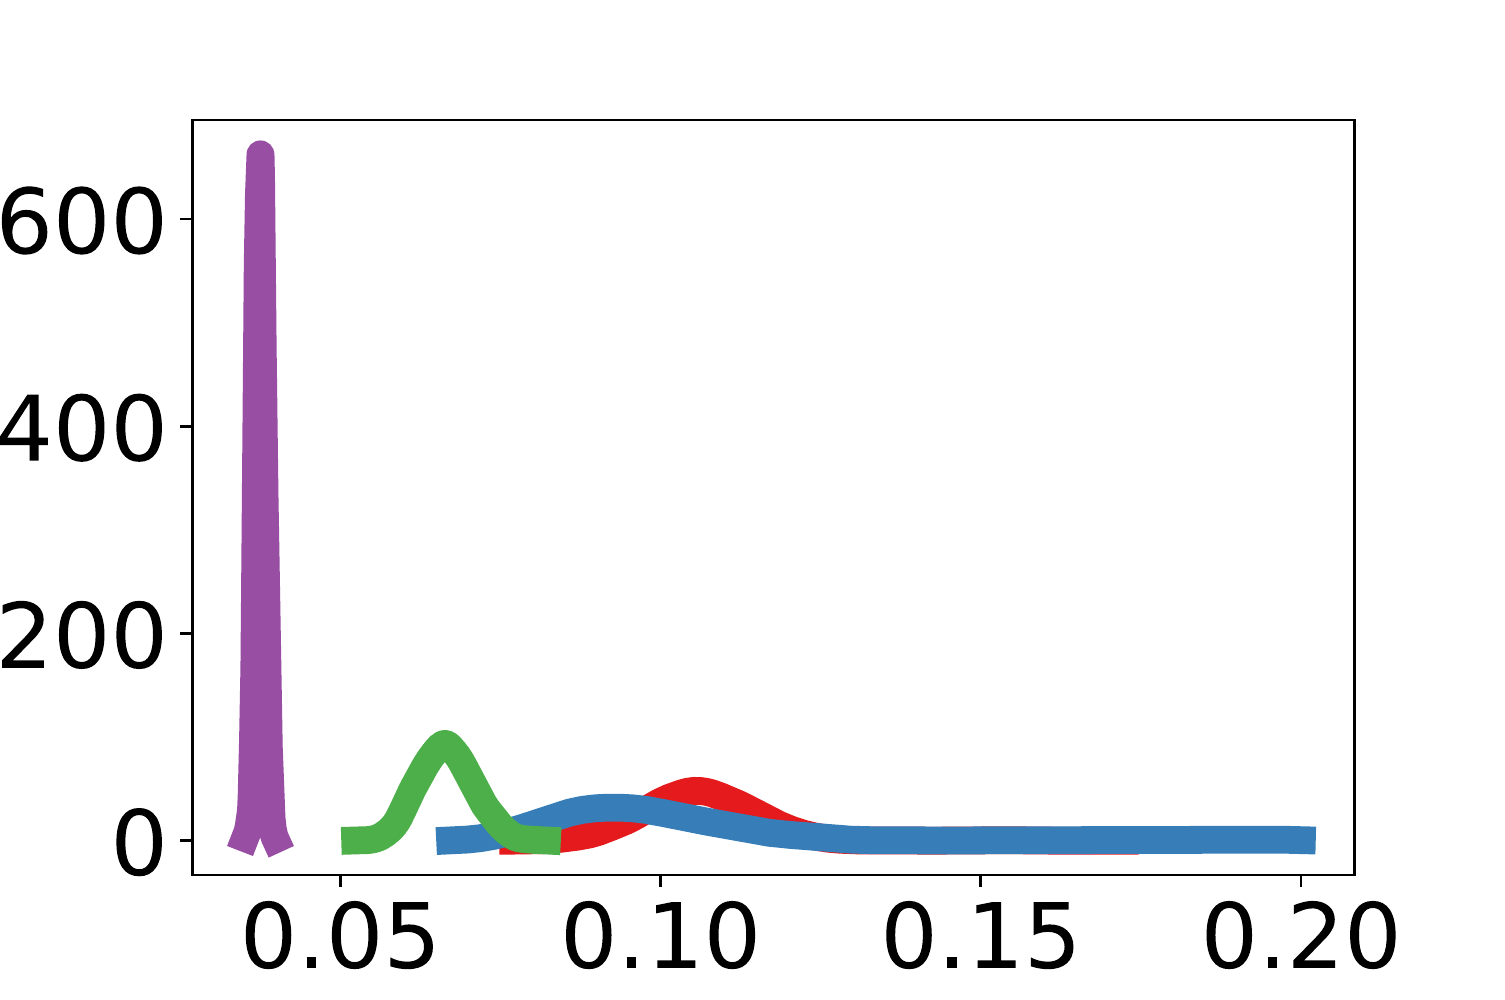_tex}
  \end{subfigure}
  \begin{subfigure}[c]{0.245\linewidth}
    \centering
    \def\svgwidth{0.99\columnwidth}
    \input{./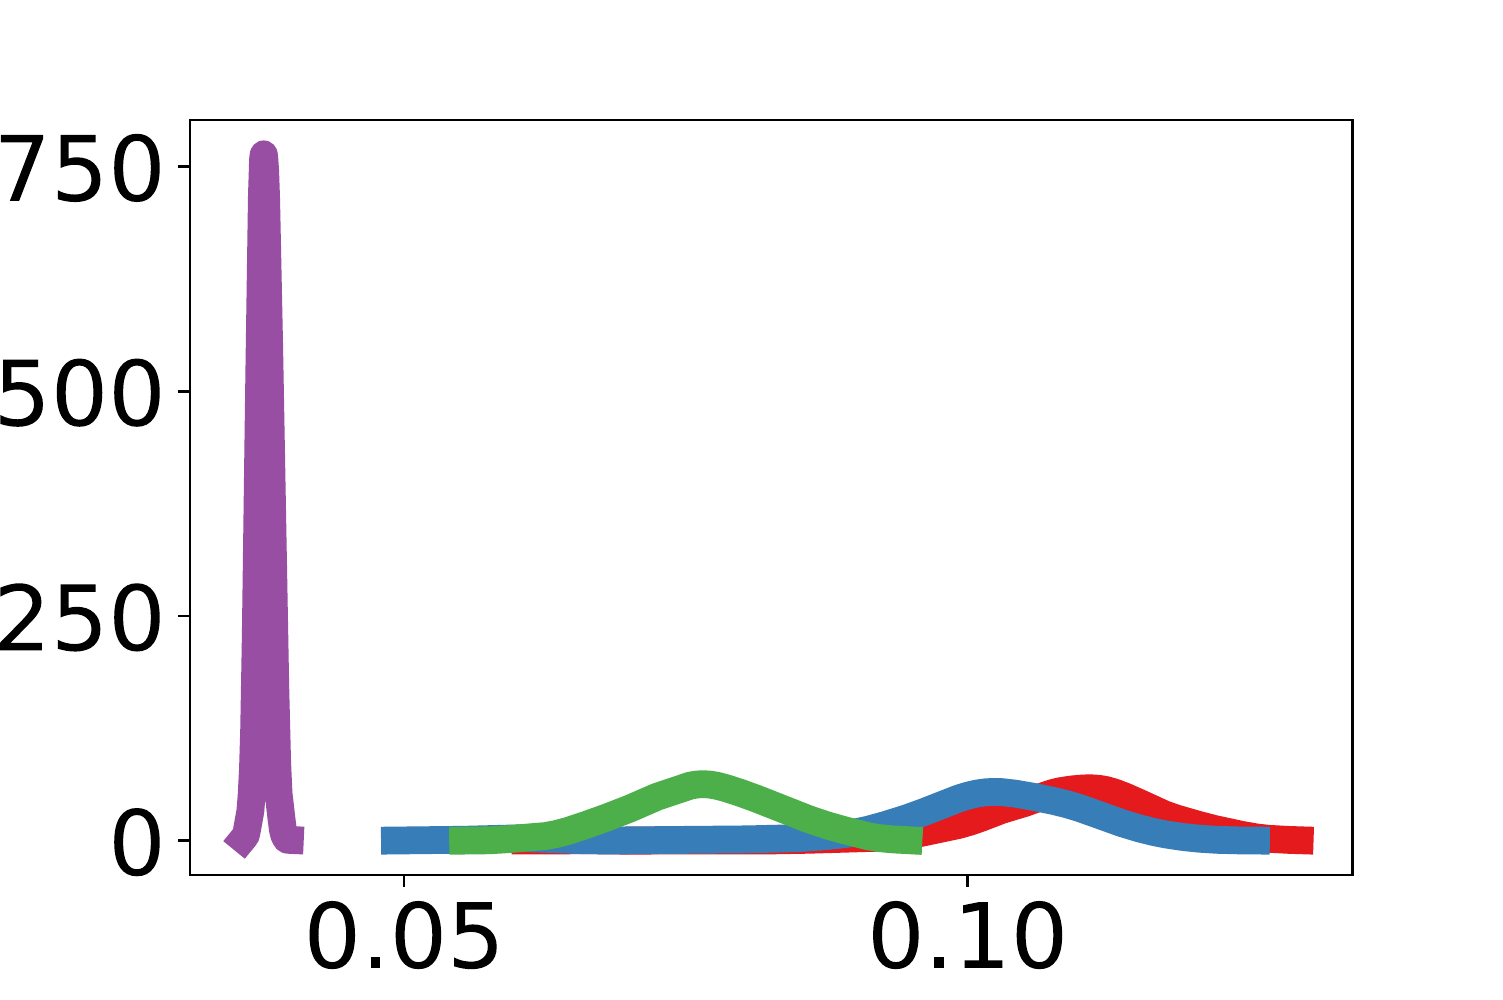_tex}
  \end{subfigure}
  \begin{subfigure}[c]{0.245\linewidth}
    \centering
    \def\svgwidth{0.99\columnwidth}
    \input{./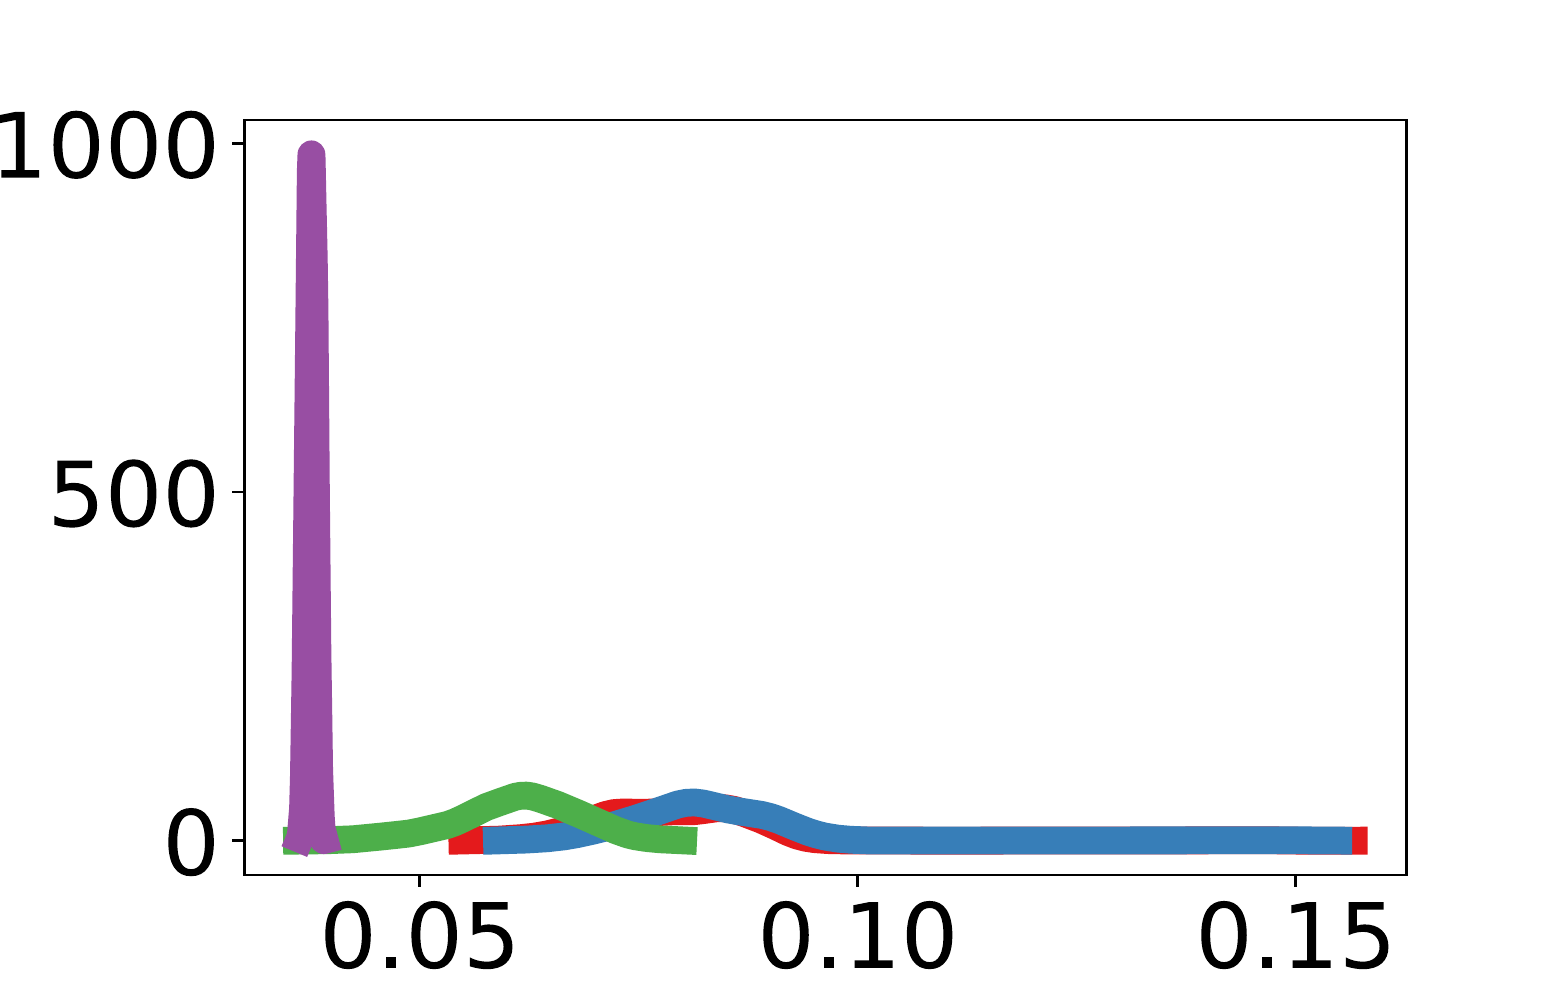_tex}
  \end{subfigure}
  \caption{Layer 4}
  \label{fig:int_lyr4_cush}
\end{figure}

\subsection{Data dependent Spectral Norm}
\label{sec:data-depend-spectr}

Here we plot the data dependent form of spectral norm for various layers
in ResNet. This is the measure used in the experiments in~\citet{bartlett2017spectrally}. We look
at ResNet models from ~\citet{Sanyal2018}, normal ResNet and randomly
initialized ResNet.

For any layer $i$, the spectral norm defines how much the output of a single layer  blows up in $\ell_2$ norm given an input that - unrolled into a single vector - has $\ell_2$ norm $1$. The following plot shows the average value of the magnification of the $\ell_2$ norm of the input defined as \[ \dfrac{1}{n} \dfrac{\ip{\norm{\vec{A}_i}}{\vec{x}_i}}{\norm{\vec{x}_i}} \]

  \begin{figure}[h!]
    \begin{subfigure}[c]{0.245\linewidth}
    \centering
    \def\svgwidth{0.99\columnwidth}
    \input{./figs/legend.pdf_tex}
  \end{subfigure}\hfill
  \begin{subfigure}[c]{0.45\linewidth}
    \centering
    \def\svgwidth{0.99\columnwidth}
    \input{./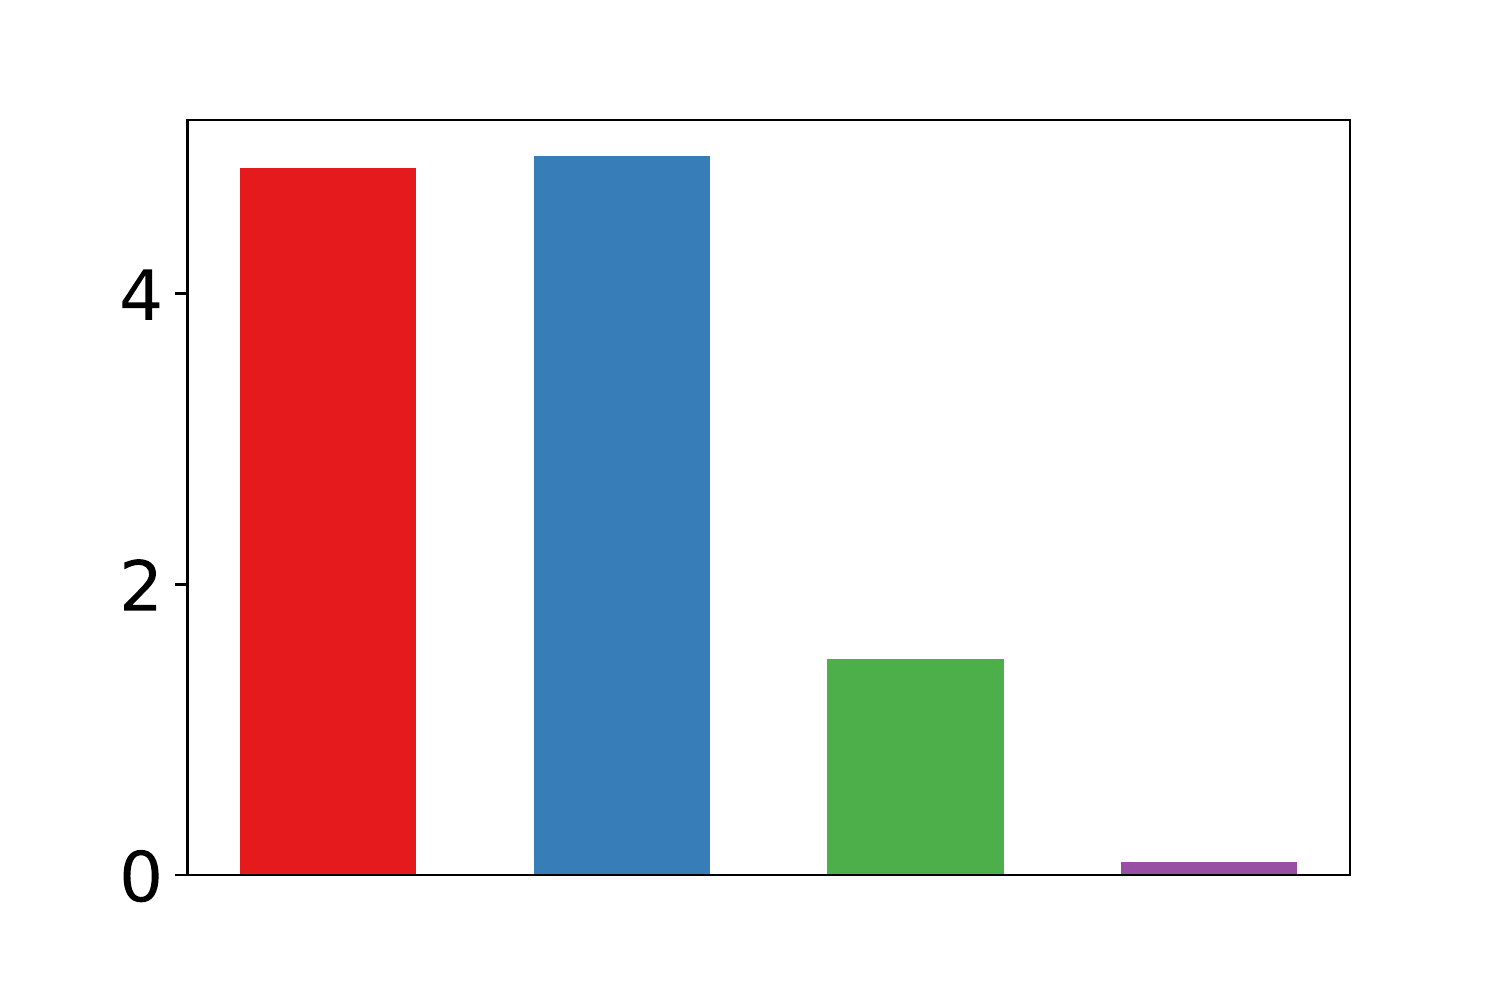_tex}
  \end{subfigure}\caption{The last fully connected layer of Resnet.}
  \end{figure}

 The following correspond to ResNet blocks. Each block has two smaller
 sub-blocks where each sub-block has two convolutional layers. The
 value of layer cushion for these modules of one block are plotted below.

\begin{center}
  \begin{figure}[h!]
  \begin{subfigure}[c]{0.245\linewidth}
    \centering
    \def\svgwidth{0.99\columnwidth}
    \input{./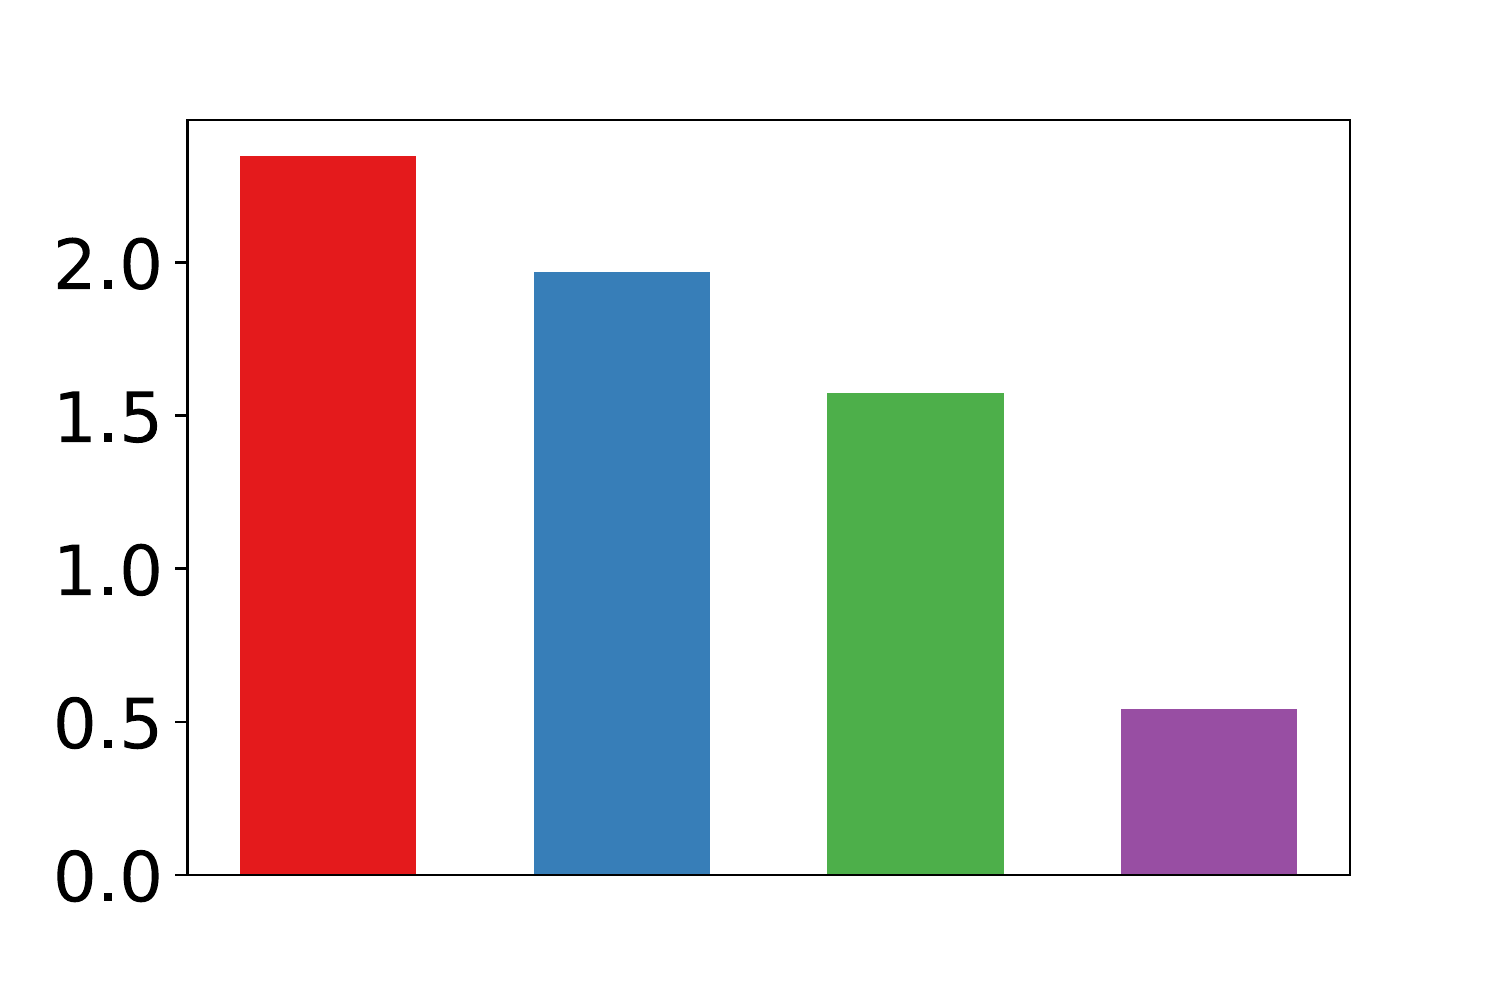_tex}
  \end{subfigure}
  \begin{subfigure}[c]{0.245\linewidth}
    \centering
    \def\svgwidth{0.99\columnwidth}
    \input{./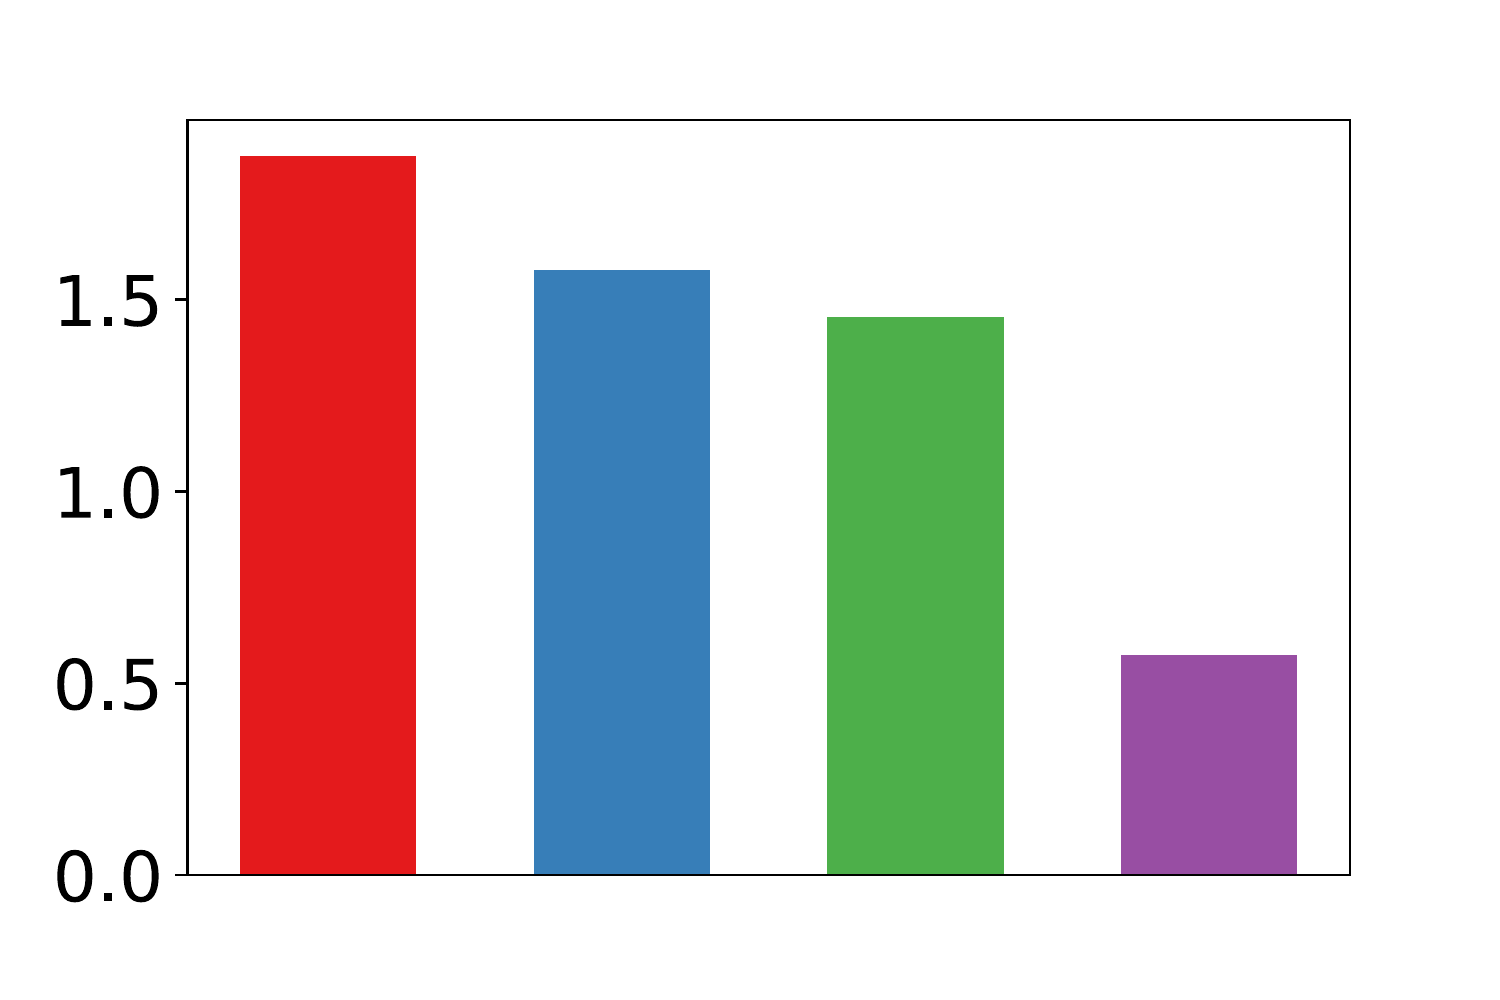_tex}
  \end{subfigure}
  \begin{subfigure}[c]{0.245\linewidth}
    \centering
    \def\svgwidth{0.99\columnwidth}
    \input{./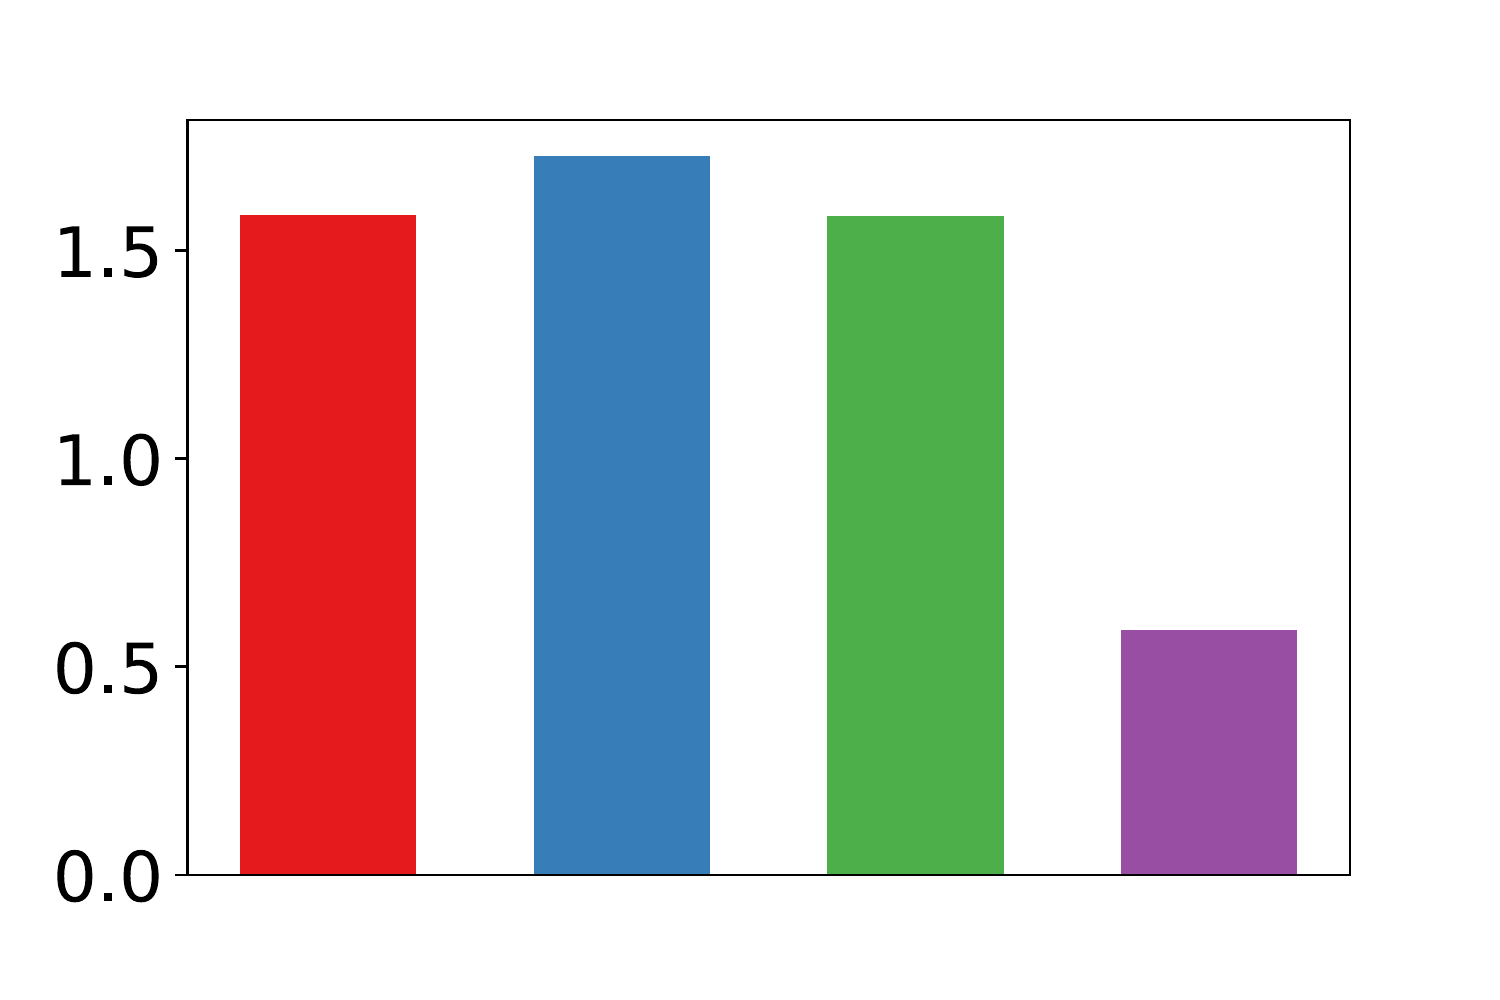_tex}
  \end{subfigure}
  \begin{subfigure}[c]{0.245\linewidth}
    \centering
    \def\svgwidth{0.99\columnwidth}
    \input{./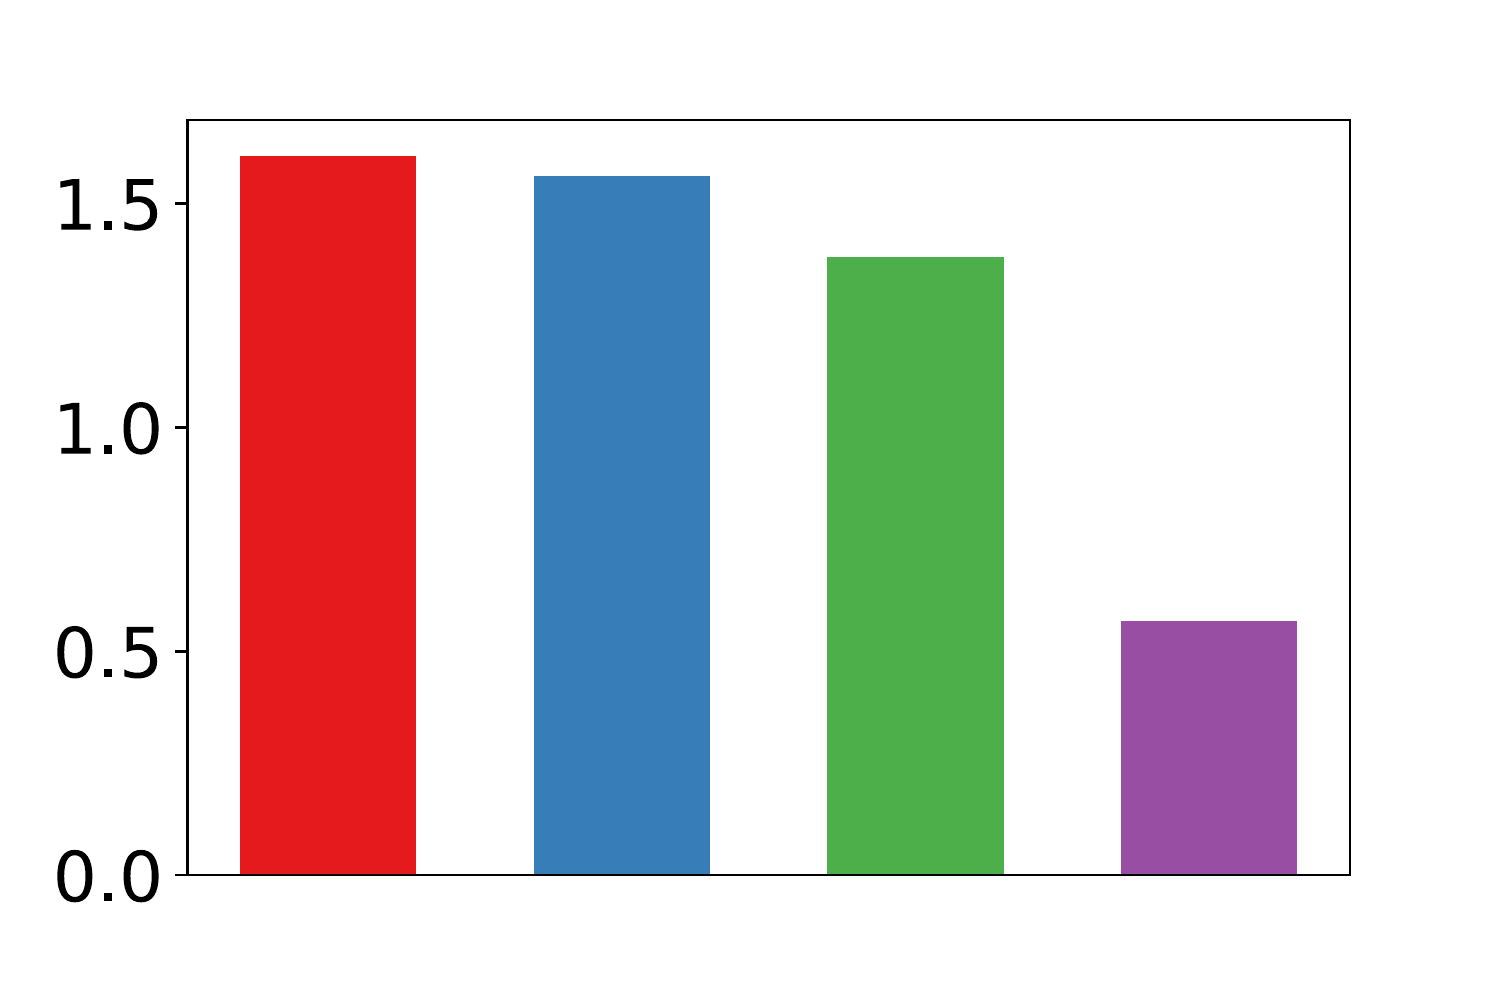_tex}
  \end{subfigure}
  \caption{Layer 1}
  \label{fig:int_spec_lyr_cush}
\end{figure}
\end{center}

\begin{center}
  \begin{figure}[h!]
  \begin{subfigure}[c]{0.245\linewidth}
    \centering
    \def\svgwidth{0.99\columnwidth}
    \input{./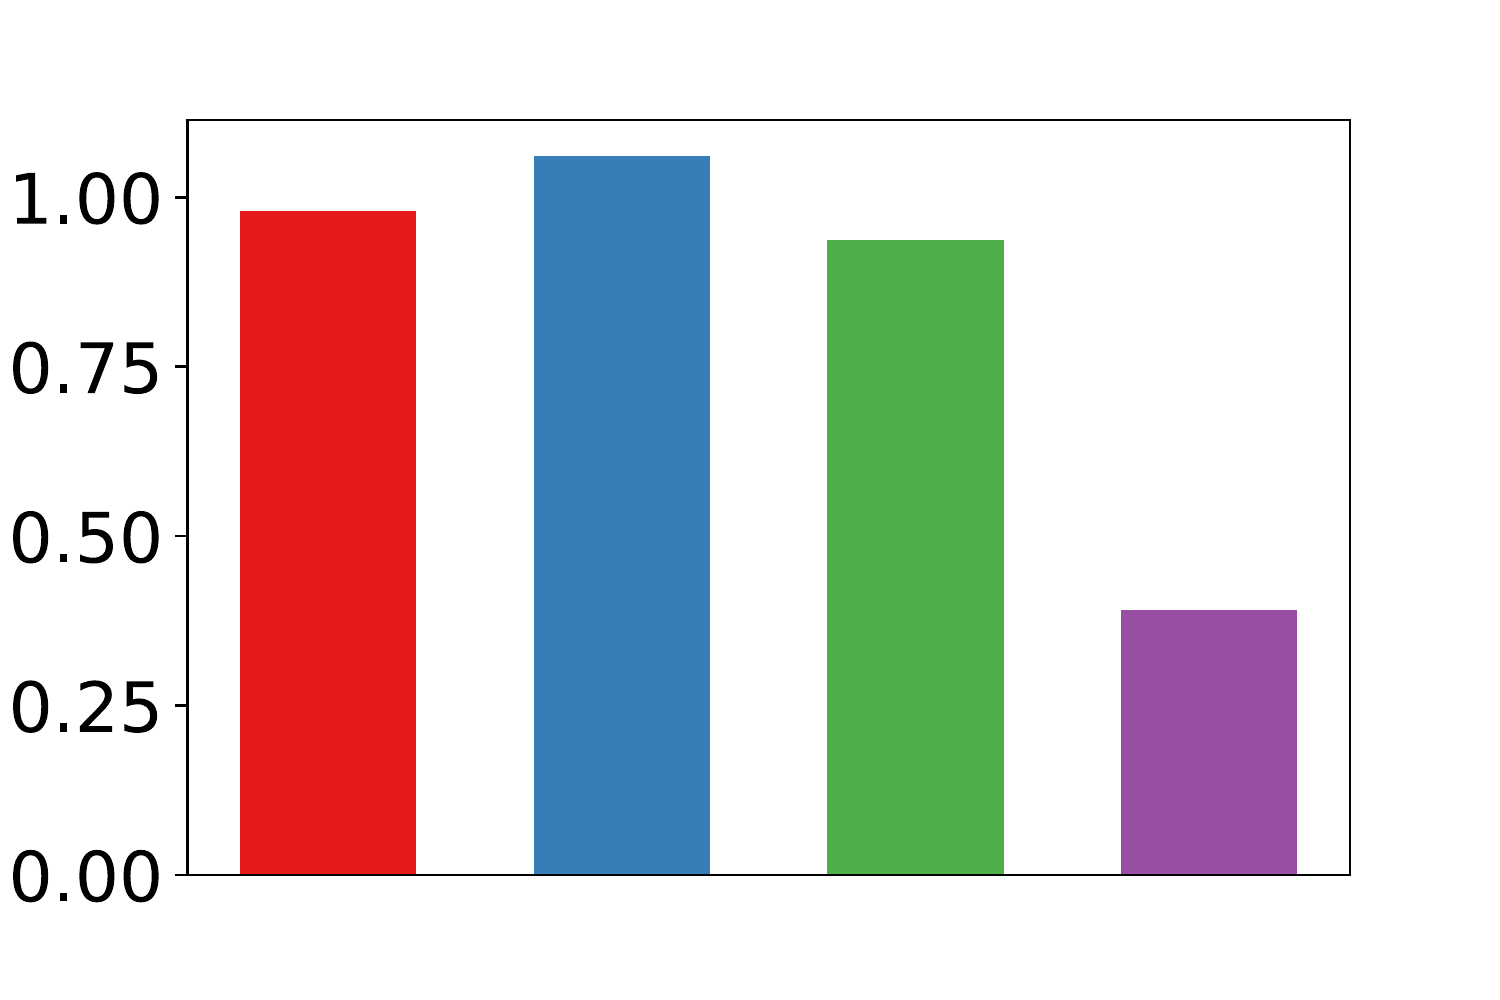_tex}
  \end{subfigure}
  \begin{subfigure}[c]{0.245\linewidth}
    \centering
    \def\svgwidth{0.99\columnwidth}
    \input{./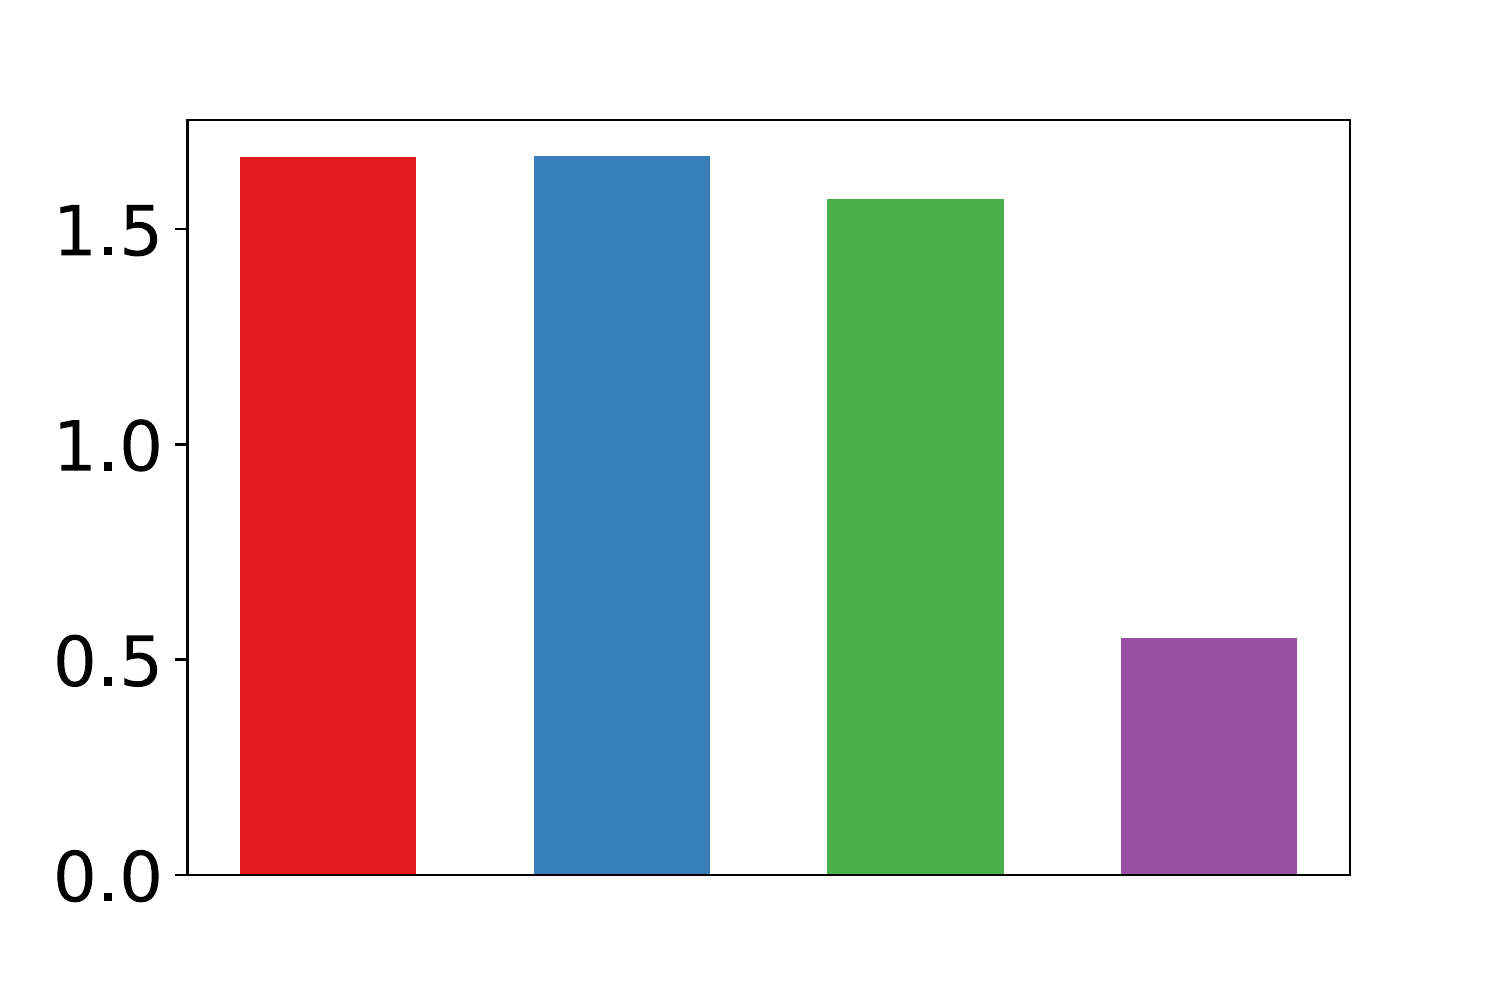_tex}
  \end{subfigure}
  \begin{subfigure}[c]{0.245\linewidth}
    \centering
    \def\svgwidth{0.99\columnwidth}
    \input{./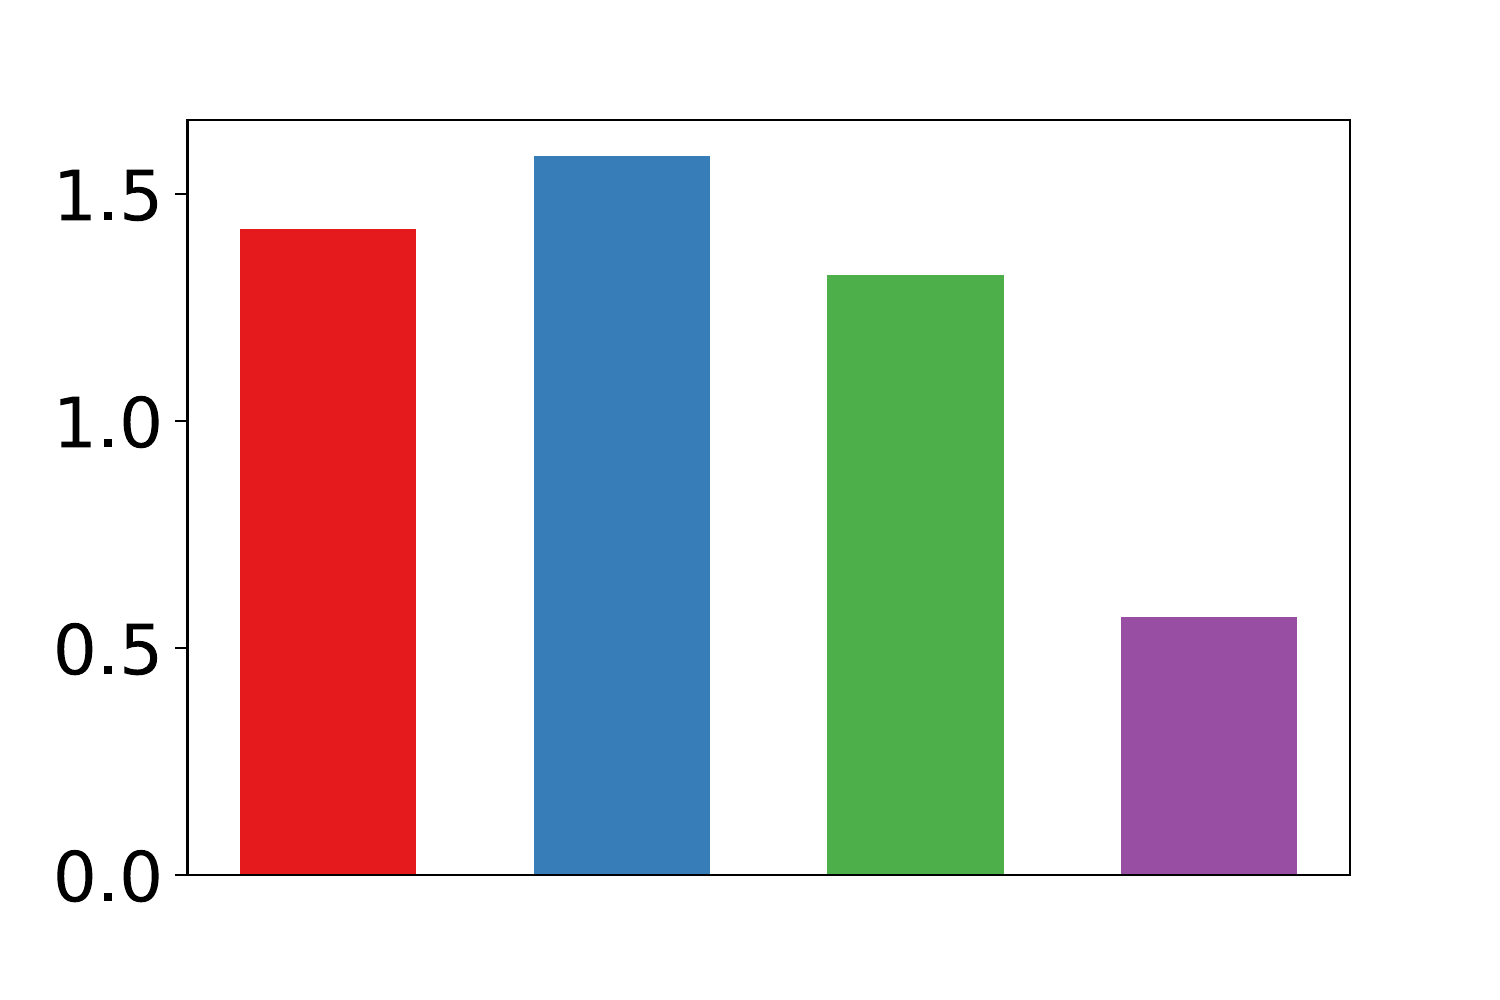_tex}
  \end{subfigure}
  \begin{subfigure}[c]{0.245\linewidth}
    \centering
    \def\svgwidth{0.99\columnwidth}
    \input{./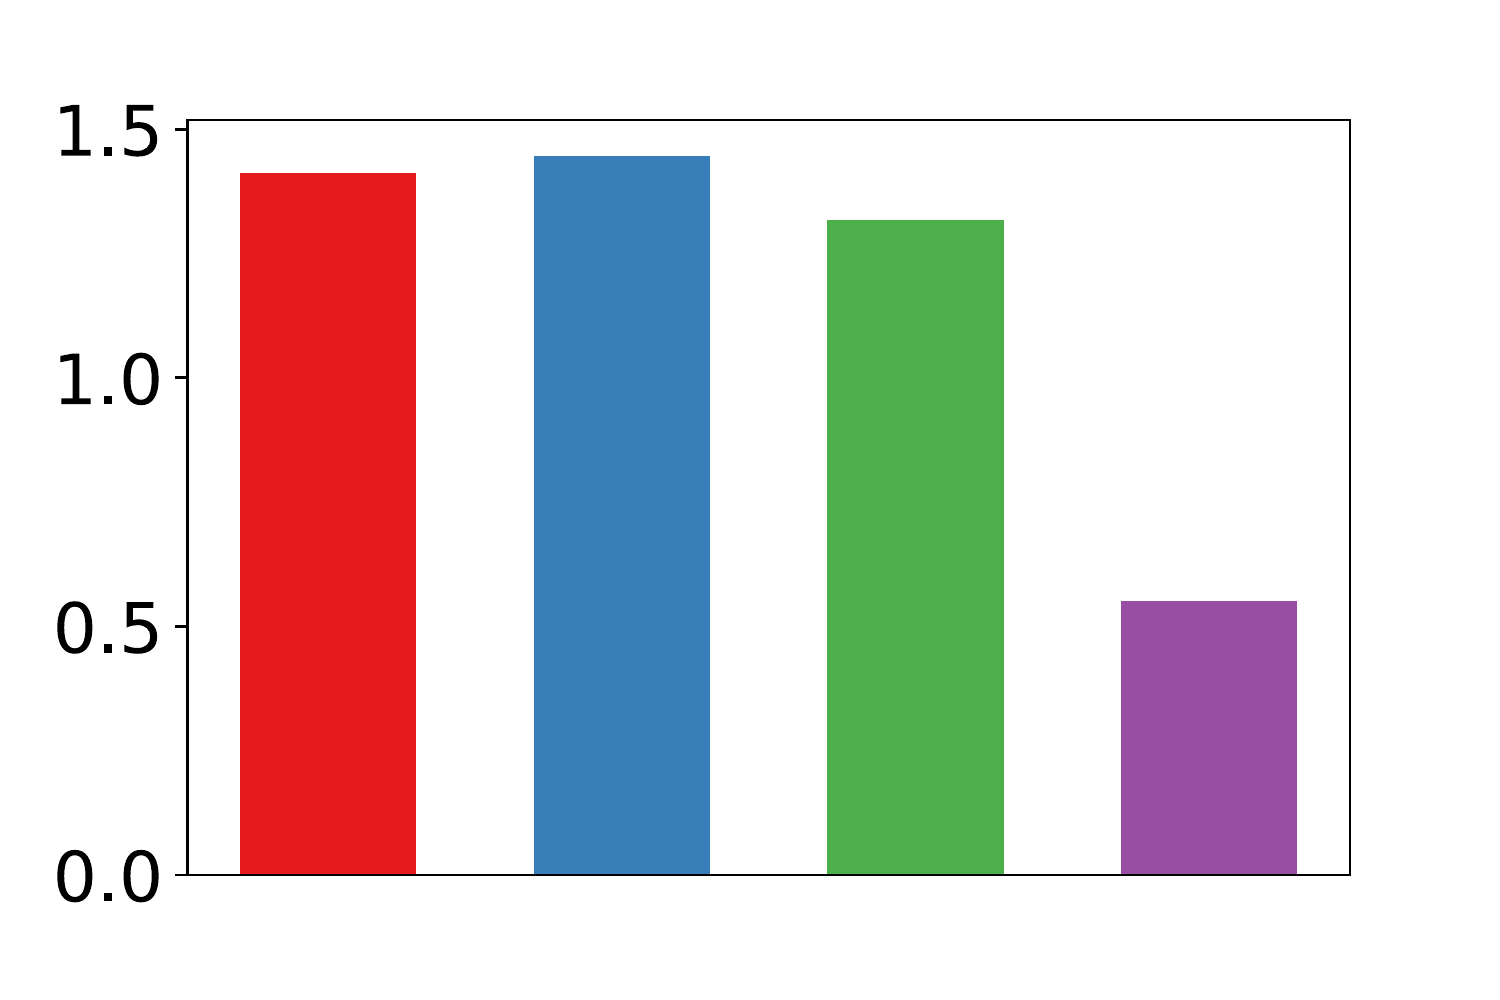_tex}
  \end{subfigure}
  \caption{Layer 2}
  \label{fig:int_spec_lyr2_cush}
\end{figure}
\end{center}

\begin{center}
  \begin{figure}[h!]
  \begin{subfigure}[c]{0.245\linewidth}
    \centering
    \def\svgwidth{0.99\columnwidth}
    \input{./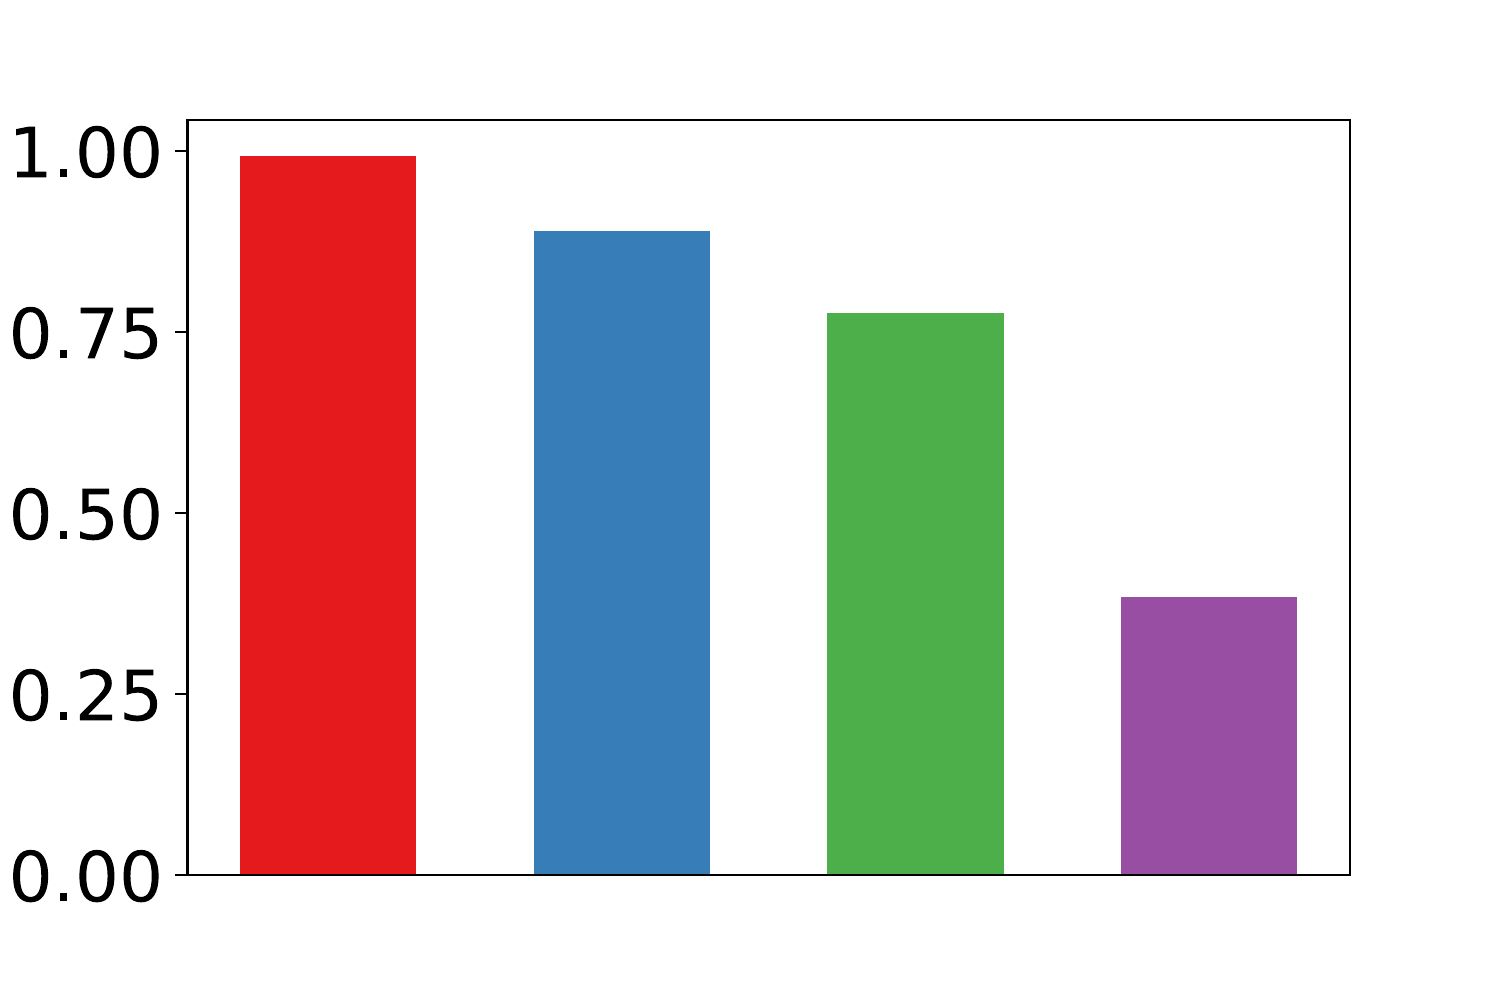_tex}
  \end{subfigure}
  \begin{subfigure}[c]{0.245\linewidth}
    \centering
    \def\svgwidth{0.99\columnwidth}
    \input{./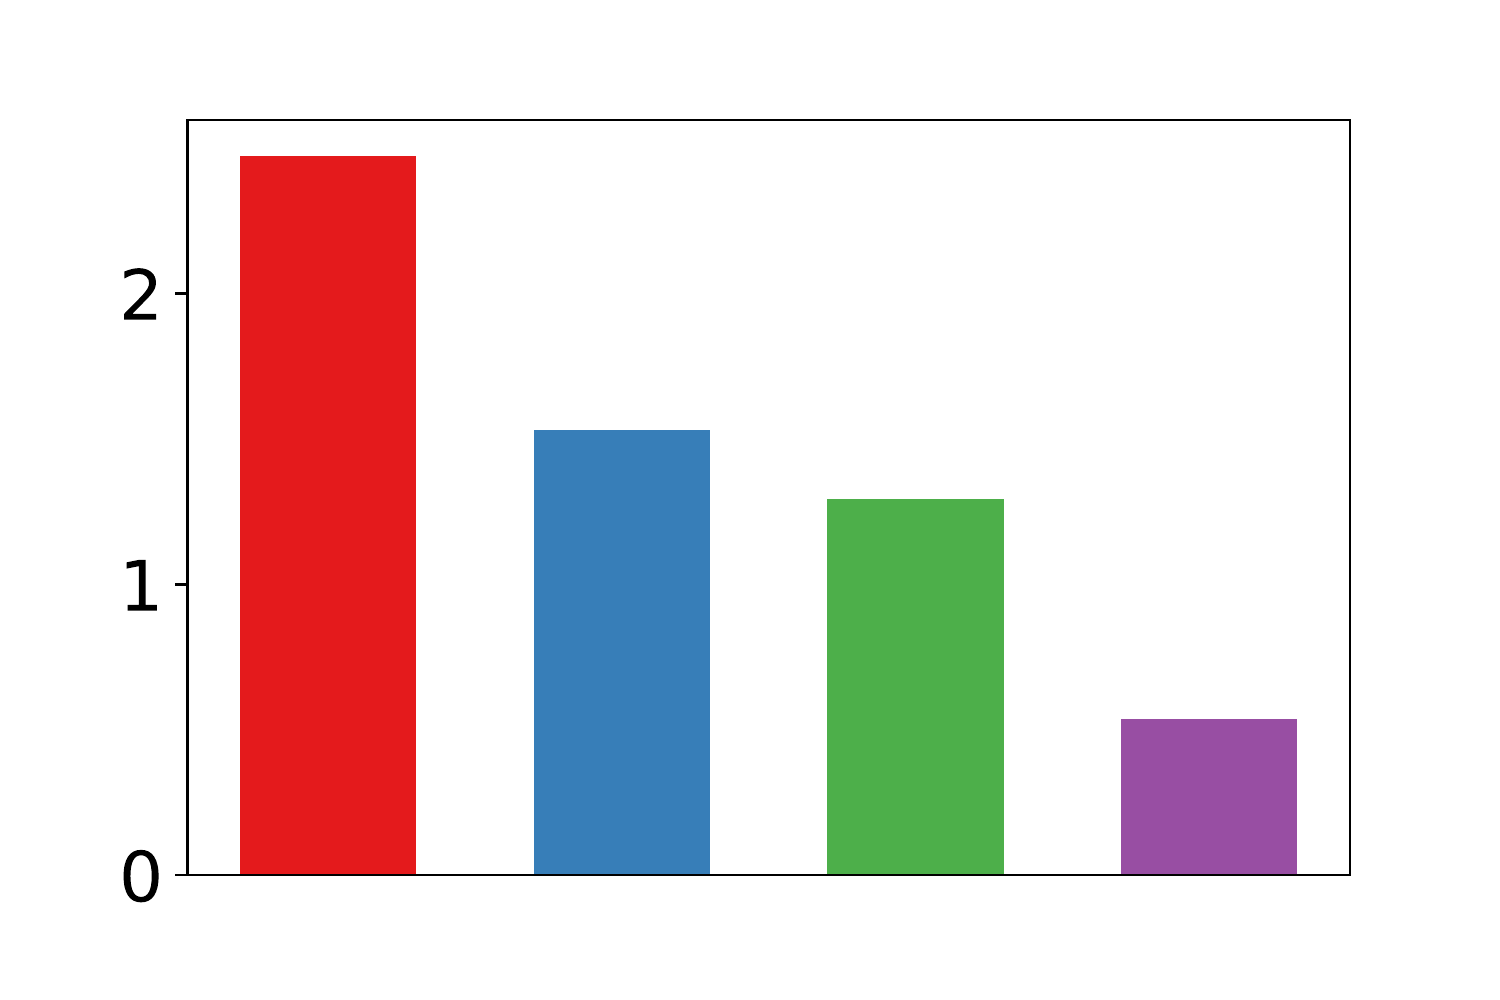_tex}
  \end{subfigure}
  \begin{subfigure}[c]{0.245\linewidth}
    \centering
    \def\svgwidth{0.99\columnwidth}
    \input{./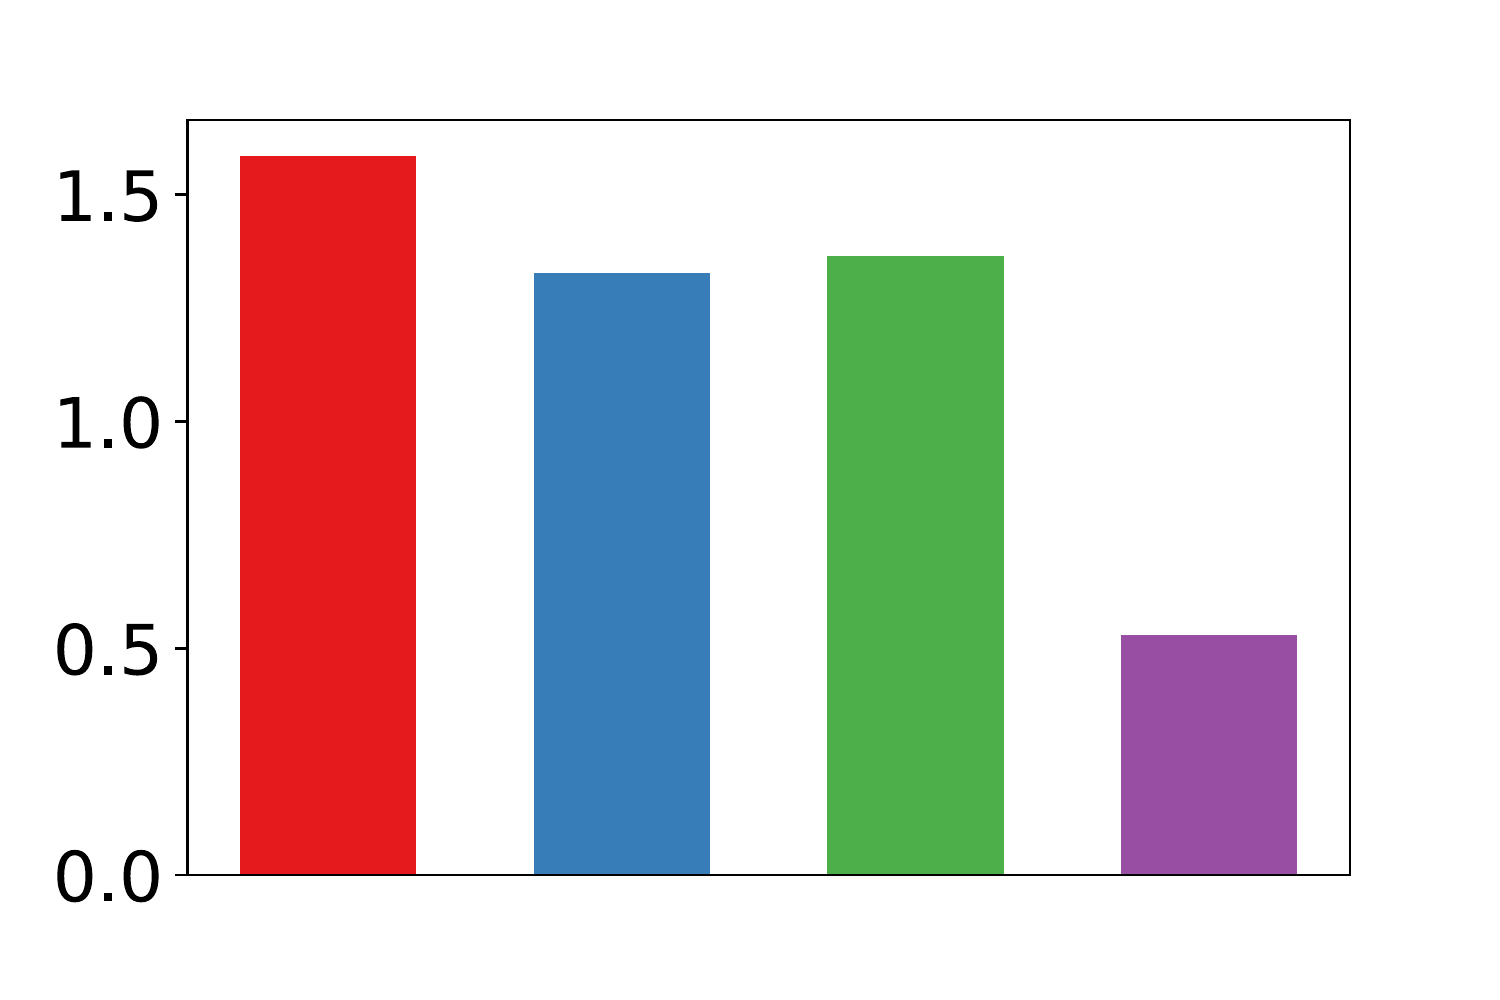_tex}
  \end{subfigure}
  \begin{subfigure}[c]{0.245\linewidth}
    \centering
    \def\svgwidth{0.99\columnwidth}
    \input{./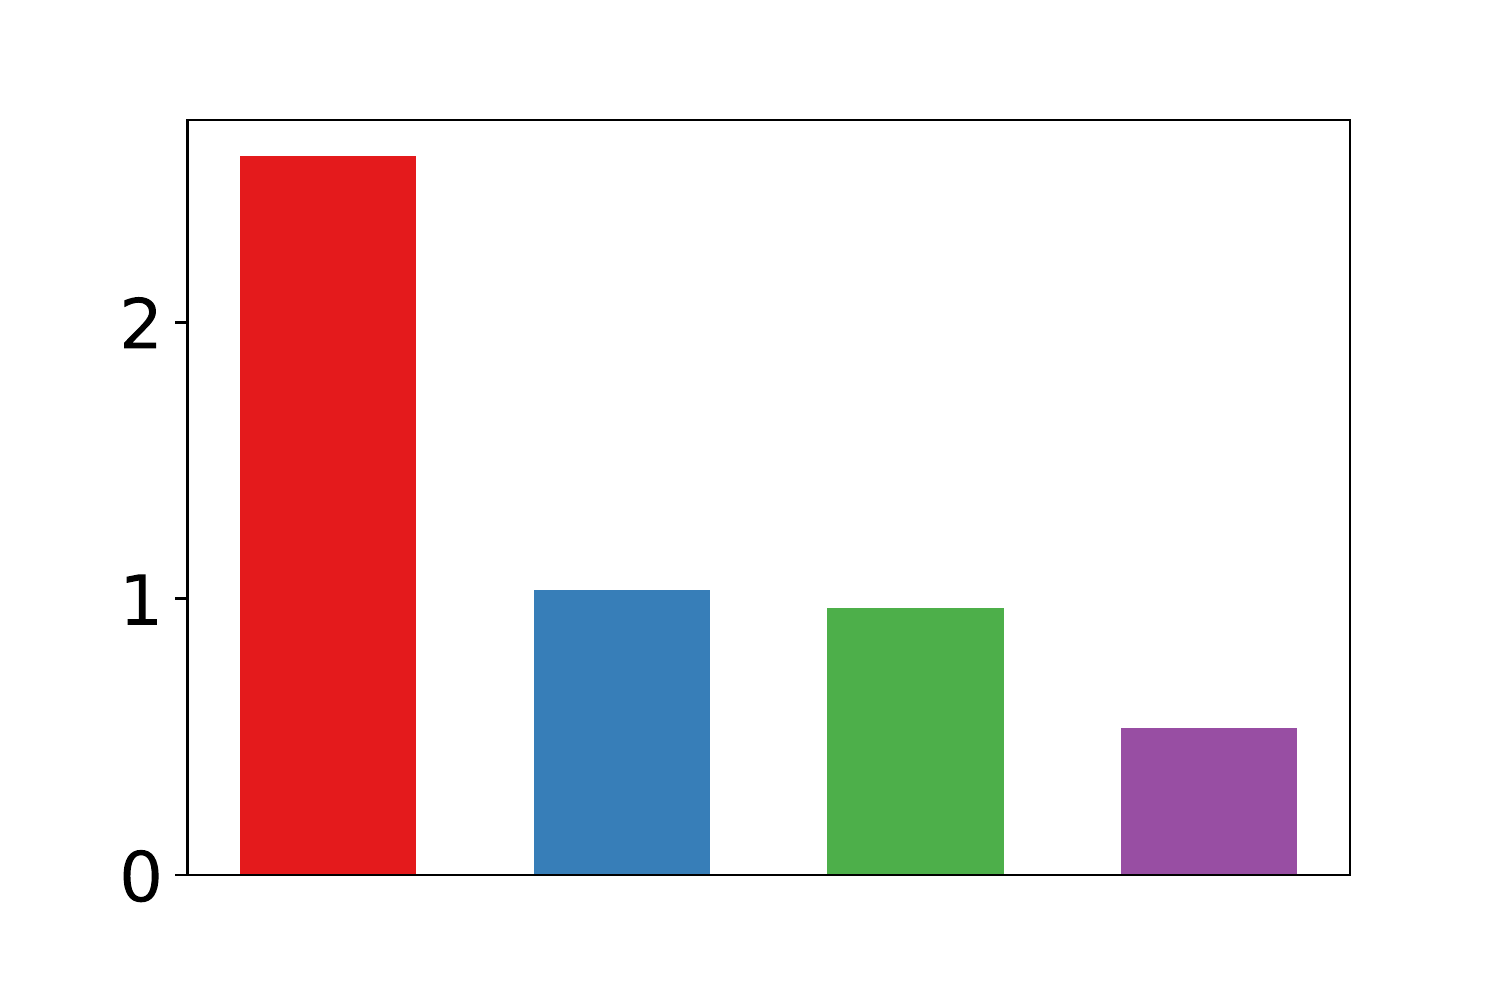_tex}
  \end{subfigure}
  \caption{Layer 3}
  \label{fig:int_spec_lyr3_cush}
\end{figure}
\end{center}
\vspace{-50pt}
  \begin{figure}[h!]
  \begin{subfigure}[c]{0.245\linewidth}
    \centering
    \def\svgwidth{0.99\columnwidth}
    \input{./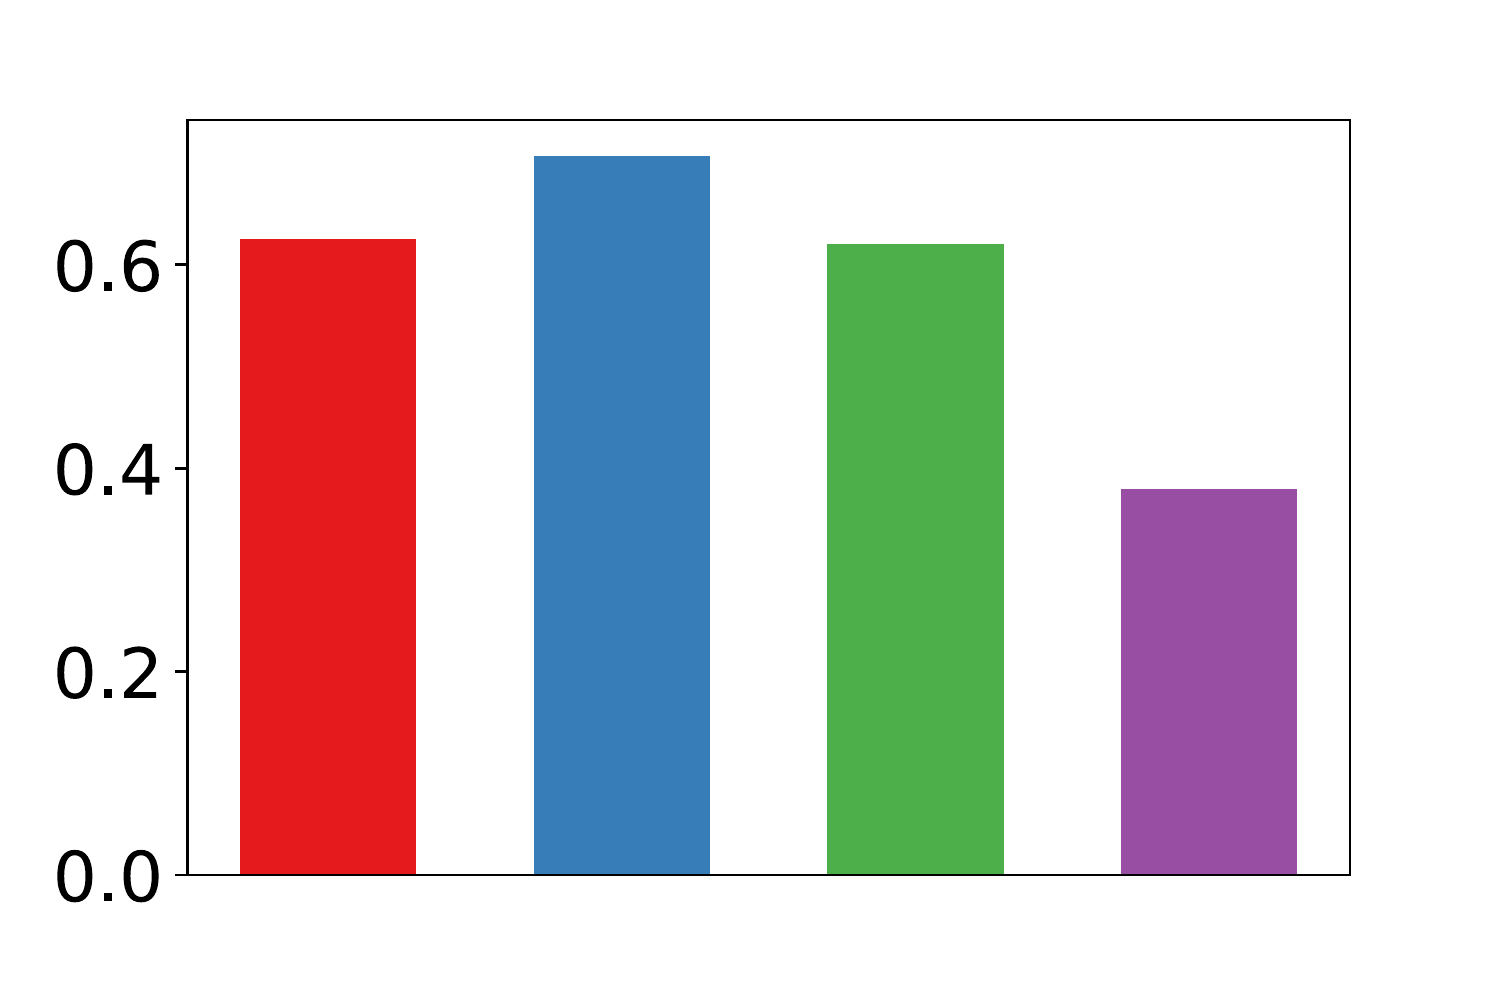_tex}
  \end{subfigure}
  \begin{subfigure}[c]{0.245\linewidth}
    \centering
    \def\svgwidth{0.99\columnwidth}
    \input{./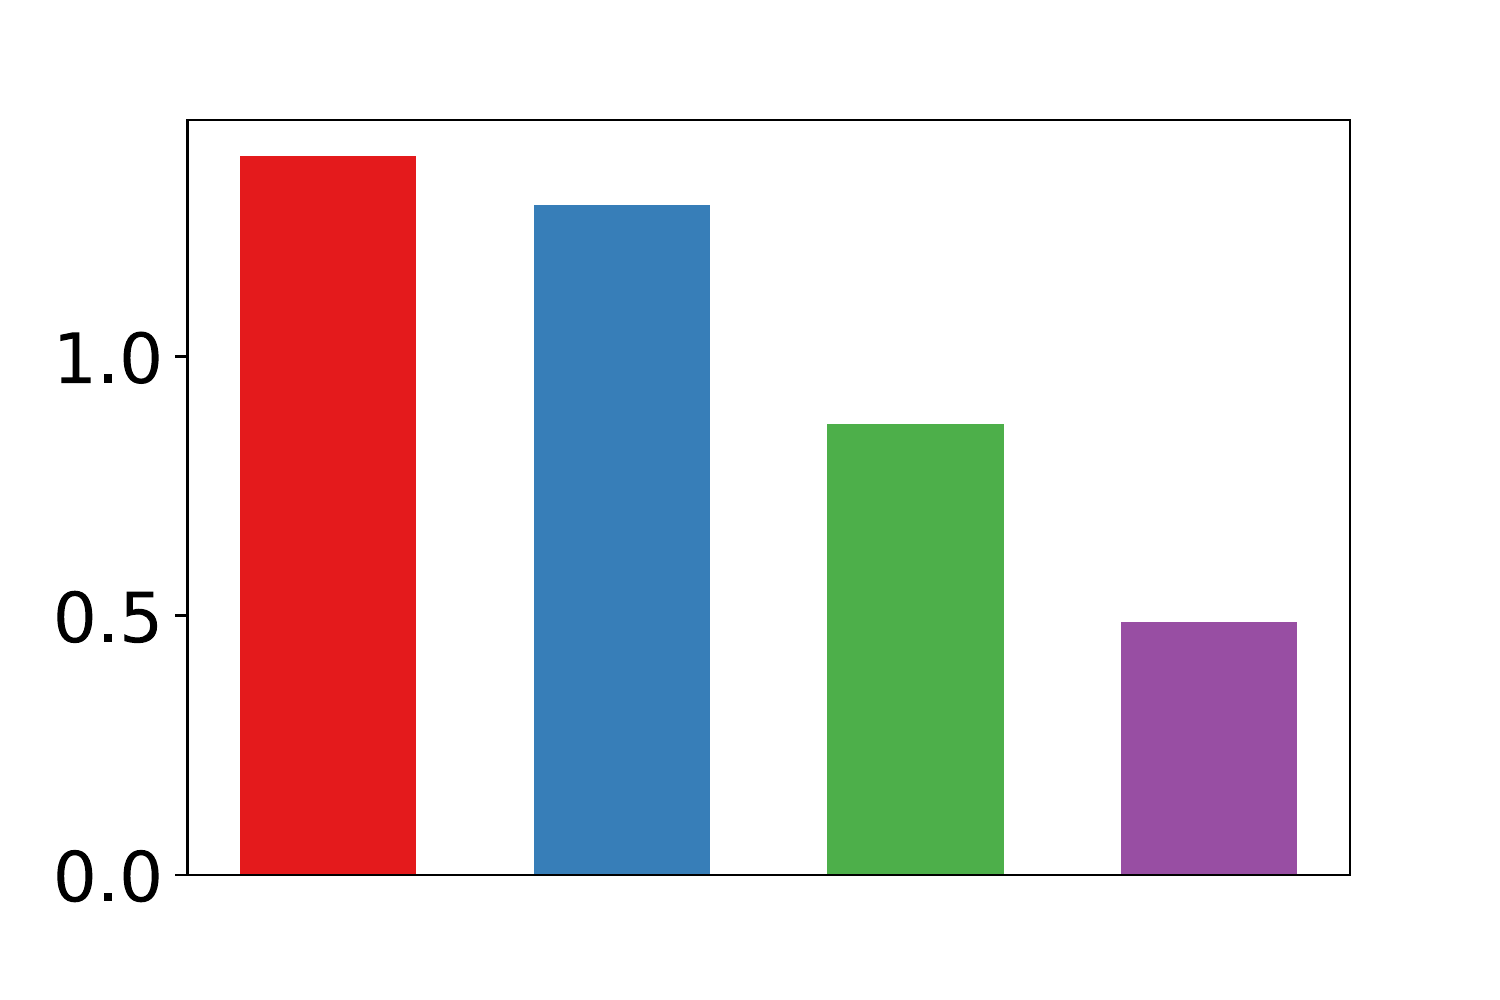_tex}
  \end{subfigure}
  \begin{subfigure}[c]{0.245\linewidth}
    \centering
    \def\svgwidth{0.99\columnwidth}
    \input{./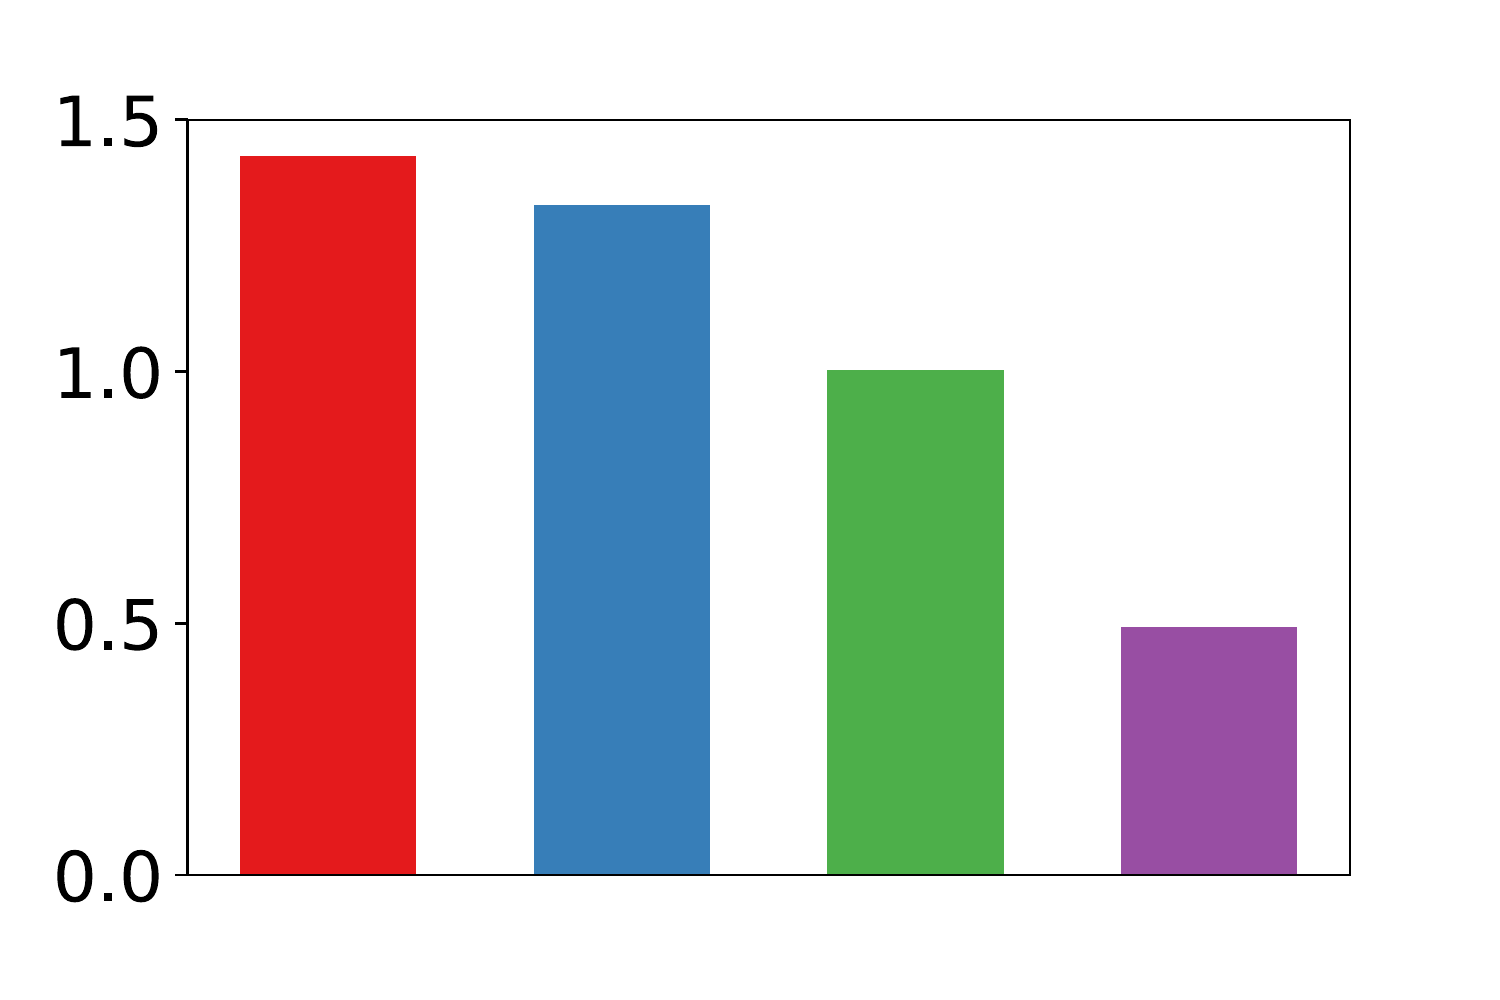_tex}
  \end{subfigure}
  \begin{subfigure}[c]{0.245\linewidth}
    \centering
    \def\svgwidth{0.99\columnwidth}
    \input{./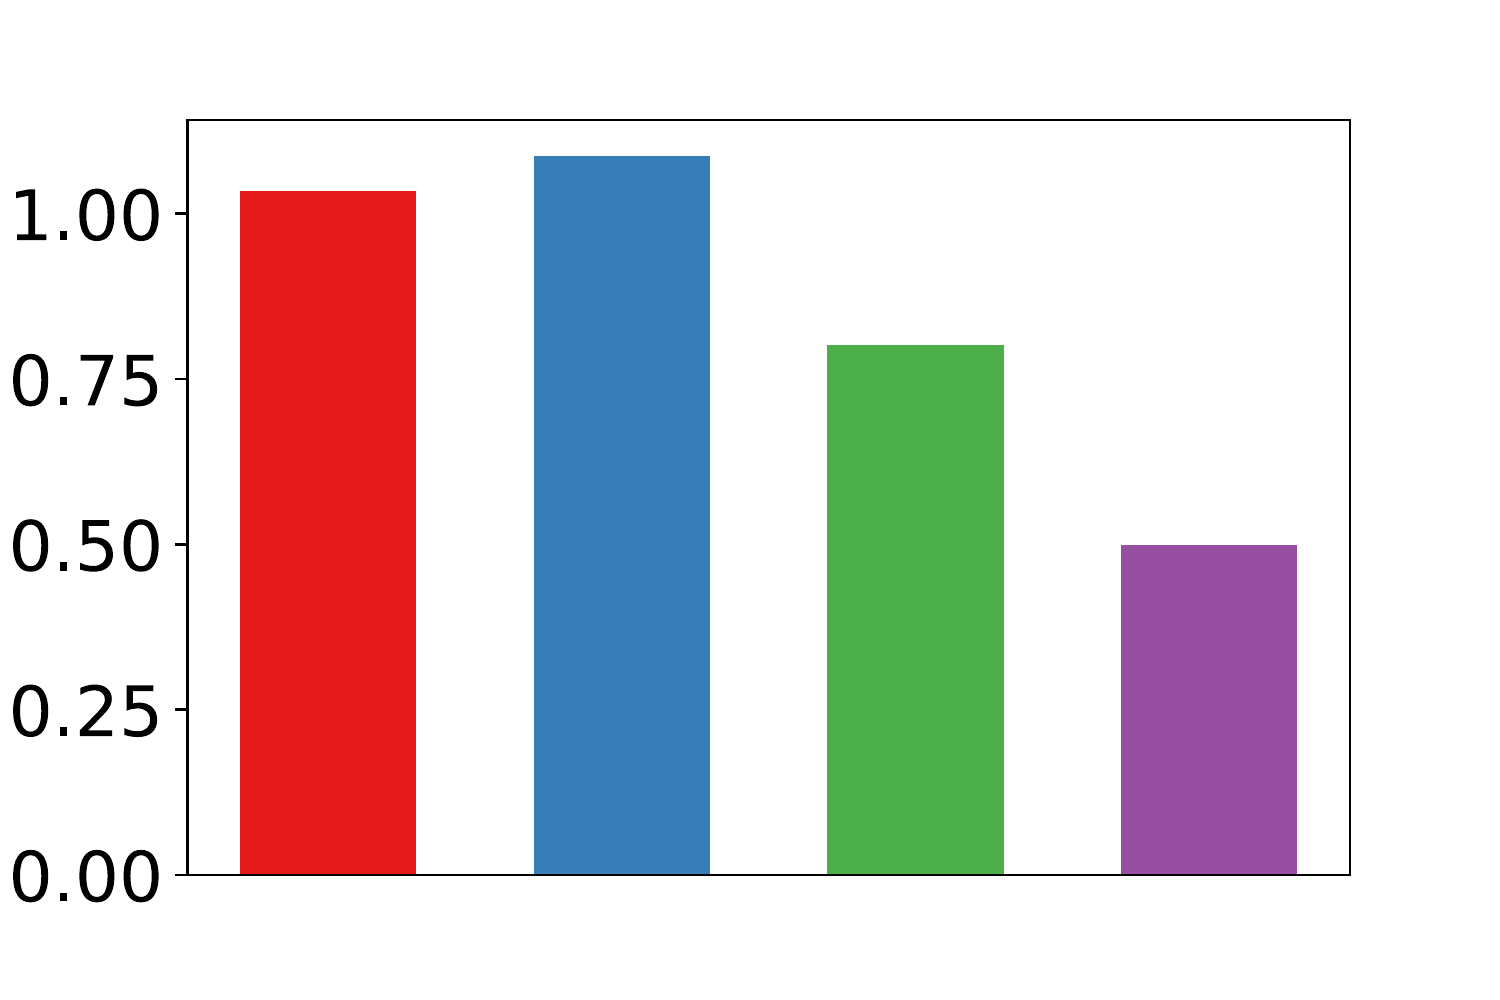_tex}
  \end{subfigure}
  \caption{Layer 4}
  \label{fig:int_spec_lyr4_cush}
\end{figure}

\subsection{Data dependent Stable Rank}
\label{sec:data-depend-spectr}

Here we plot the data dependent form of stable rank for various layers
in ResNet. This is the measure used in the experiments in~\citet{bartlett2017spectrally}. We look
at ResNet models from ~\citet{Sanyal2018}, normal ResNet and randomly
initialized ResNet.

  \begin{figure}[h!]
    \begin{subfigure}[c]{0.245\linewidth}
    \centering
    \def\svgwidth{0.99\columnwidth}
    \input{./figs/legend.pdf_tex}
  \end{subfigure}\hfill
  \begin{subfigure}[c]{0.45\linewidth}
    \centering
    \def\svgwidth{0.99\columnwidth}
    \input{./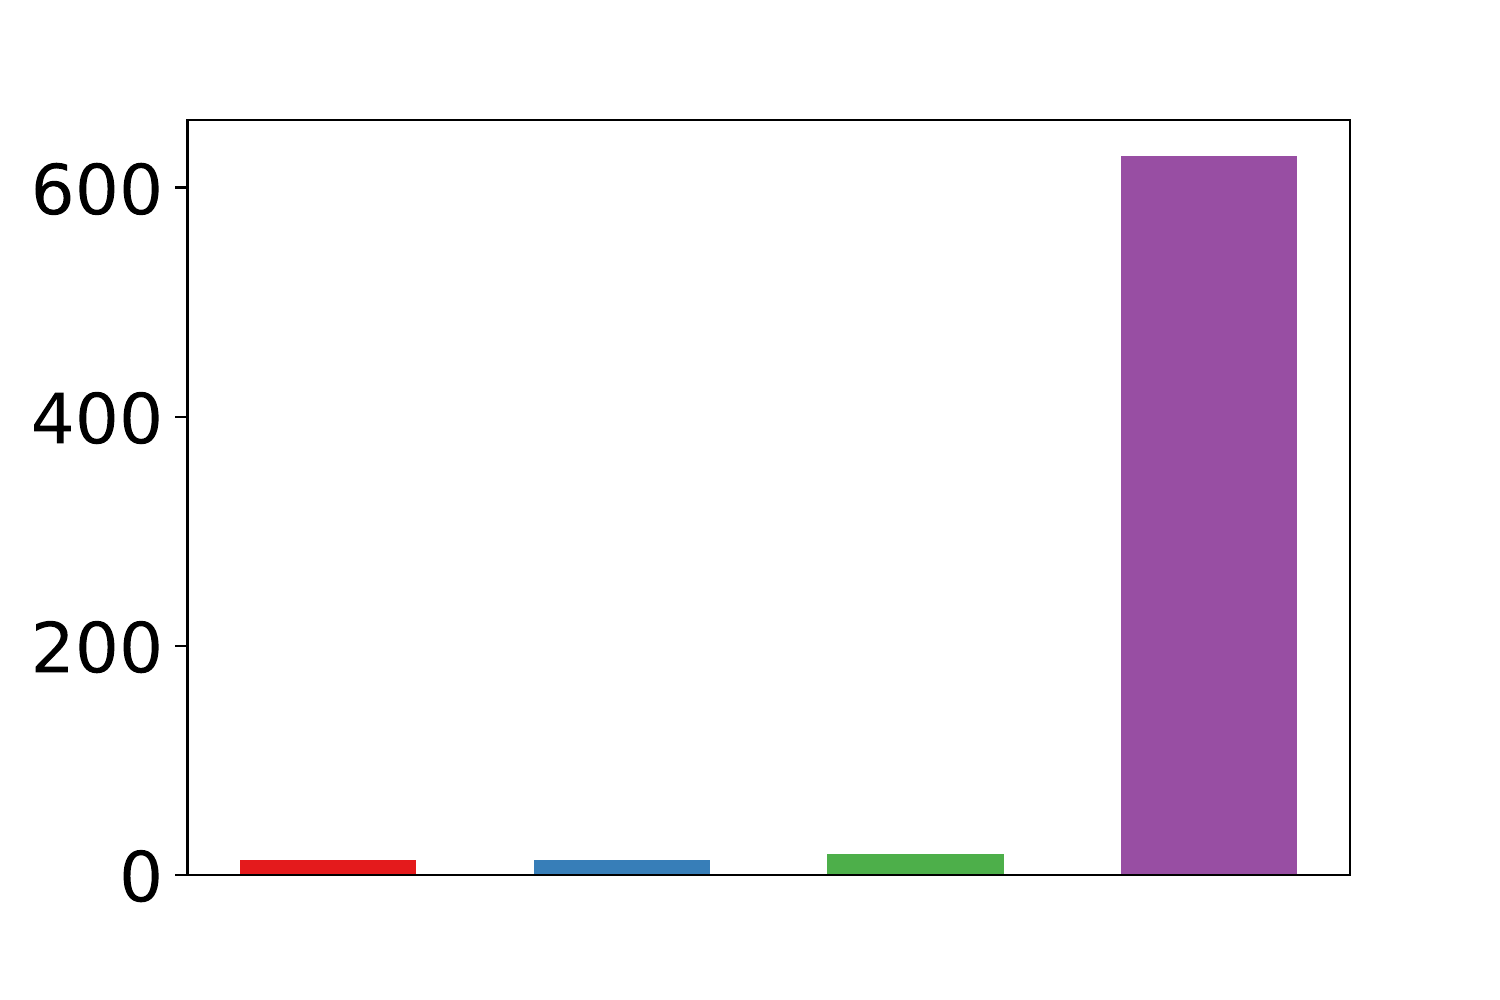_tex}
  \end{subfigure}\caption{The last fully connected layer of Resnet.}
  \end{figure}

 The following correspond to ResNet blocks. Each block has two smaller
 sub-blocks where each sub-block has two convolutional layers. The
 value of layer cushion for these modules of one block are plotted below.

\begin{center}
  \begin{figure}[h!]
  \begin{subfigure}[c]{0.245\linewidth}
    \centering
    \def\svgwidth{0.99\columnwidth}
    \input{./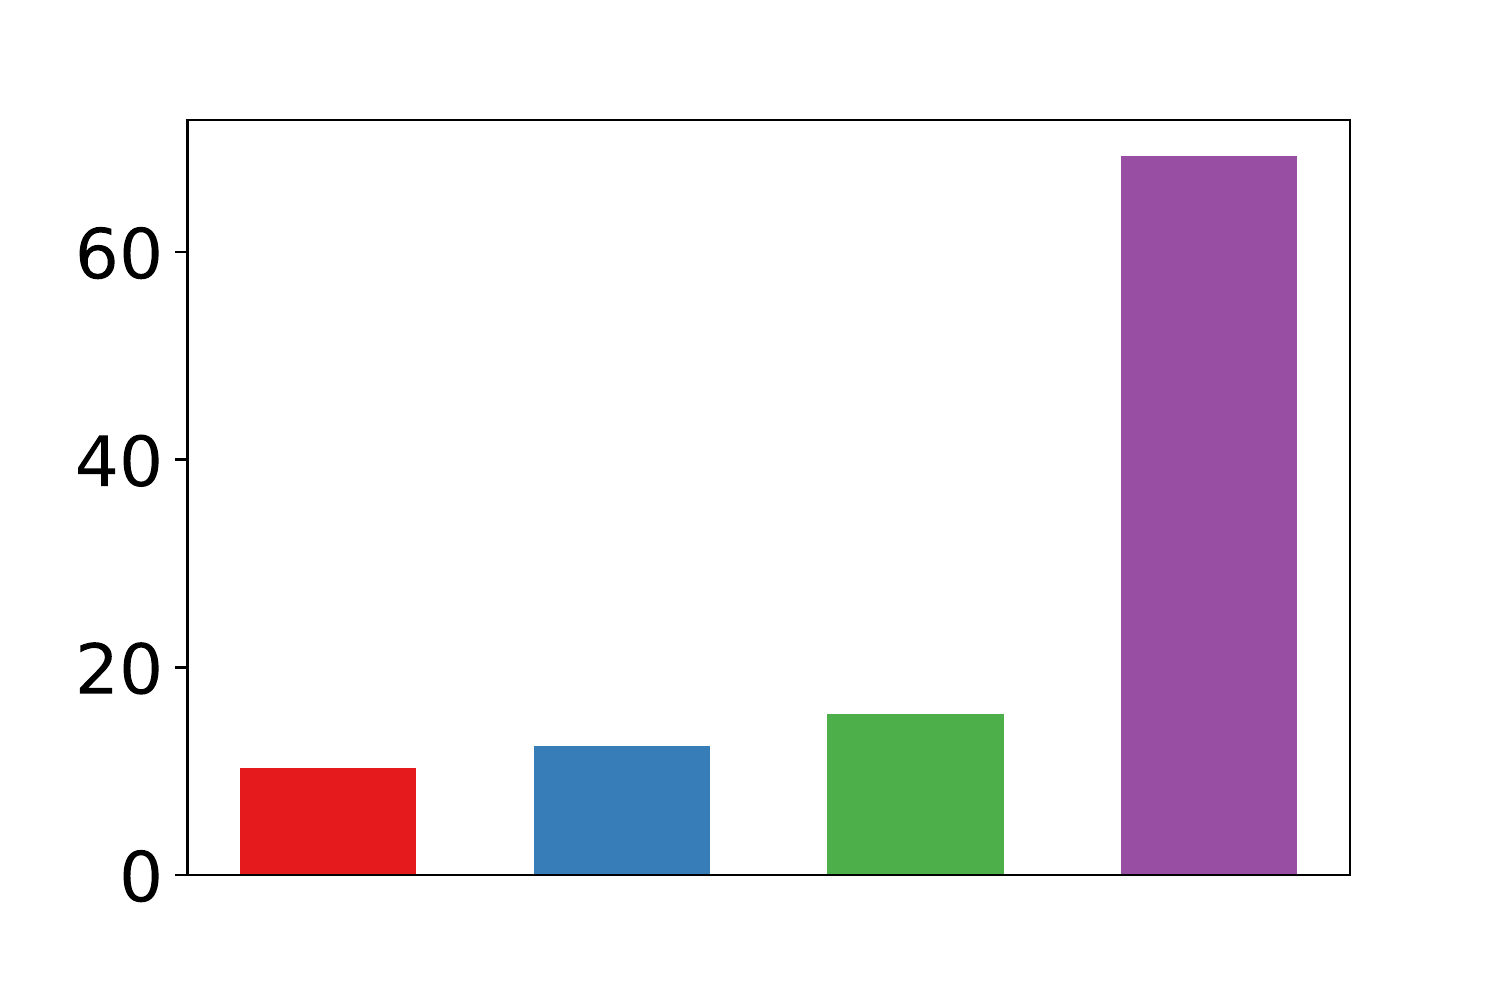_tex}
  \end{subfigure}
  \begin{subfigure}[c]{0.245\linewidth}
    \centering
    \def\svgwidth{0.99\columnwidth}
    \input{./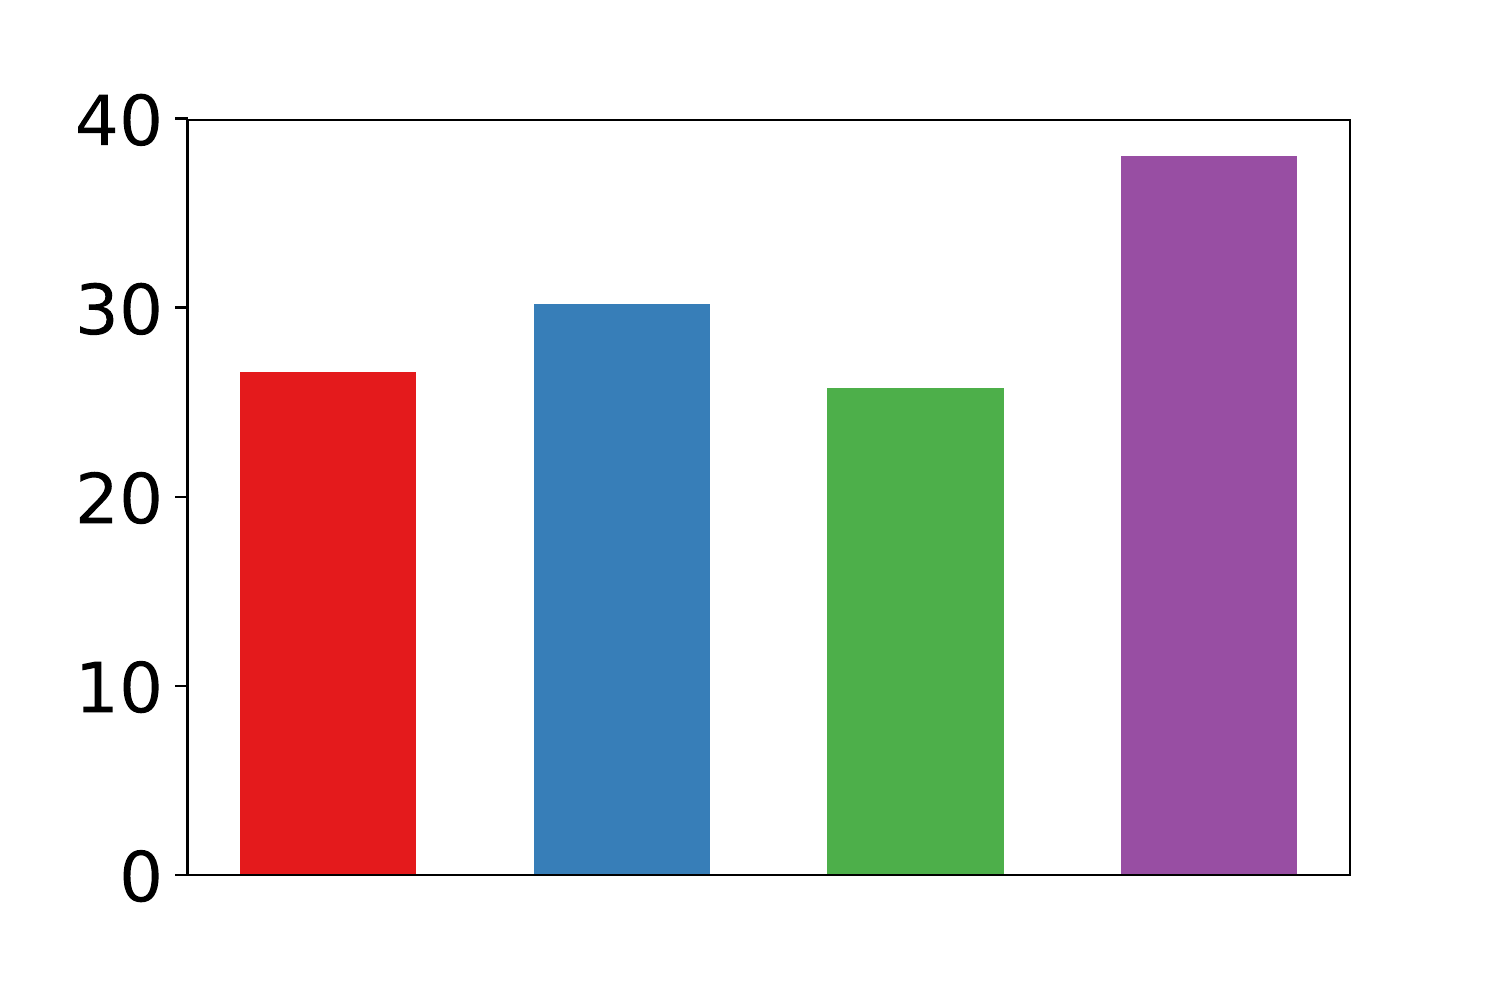_tex}
  \end{subfigure}
  \begin{subfigure}[c]{0.245\linewidth}
    \centering
    \def\svgwidth{0.99\columnwidth}
    \input{./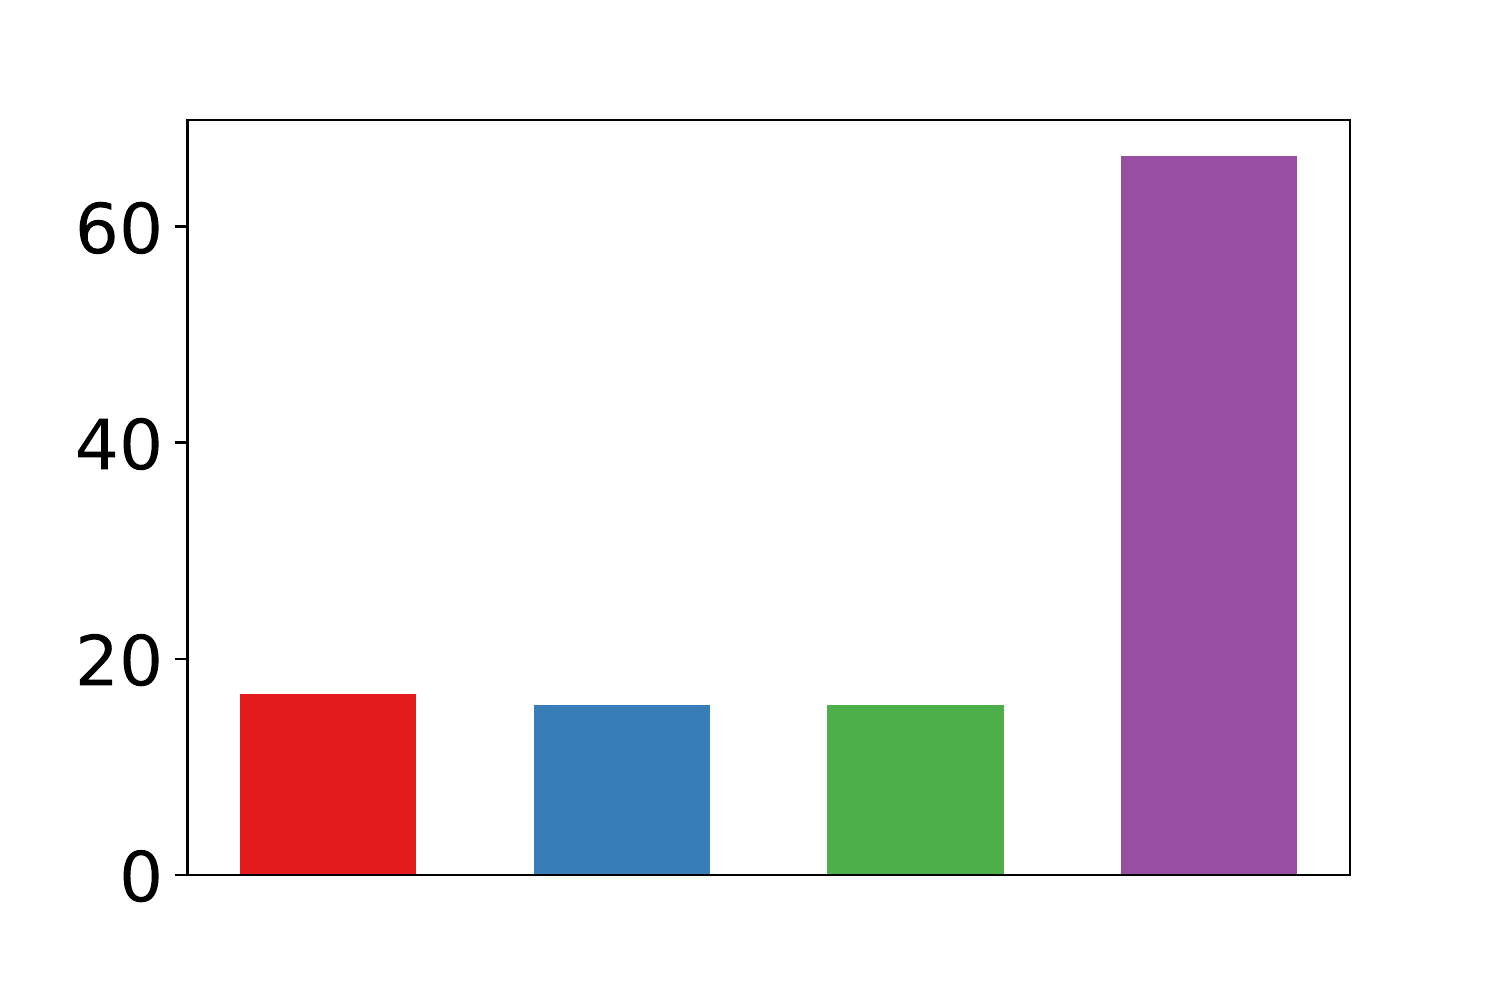_tex}
  \end{subfigure}
  \begin{subfigure}[c]{0.245\linewidth}
    \centering
    \def\svgwidth{0.99\columnwidth}
    \input{./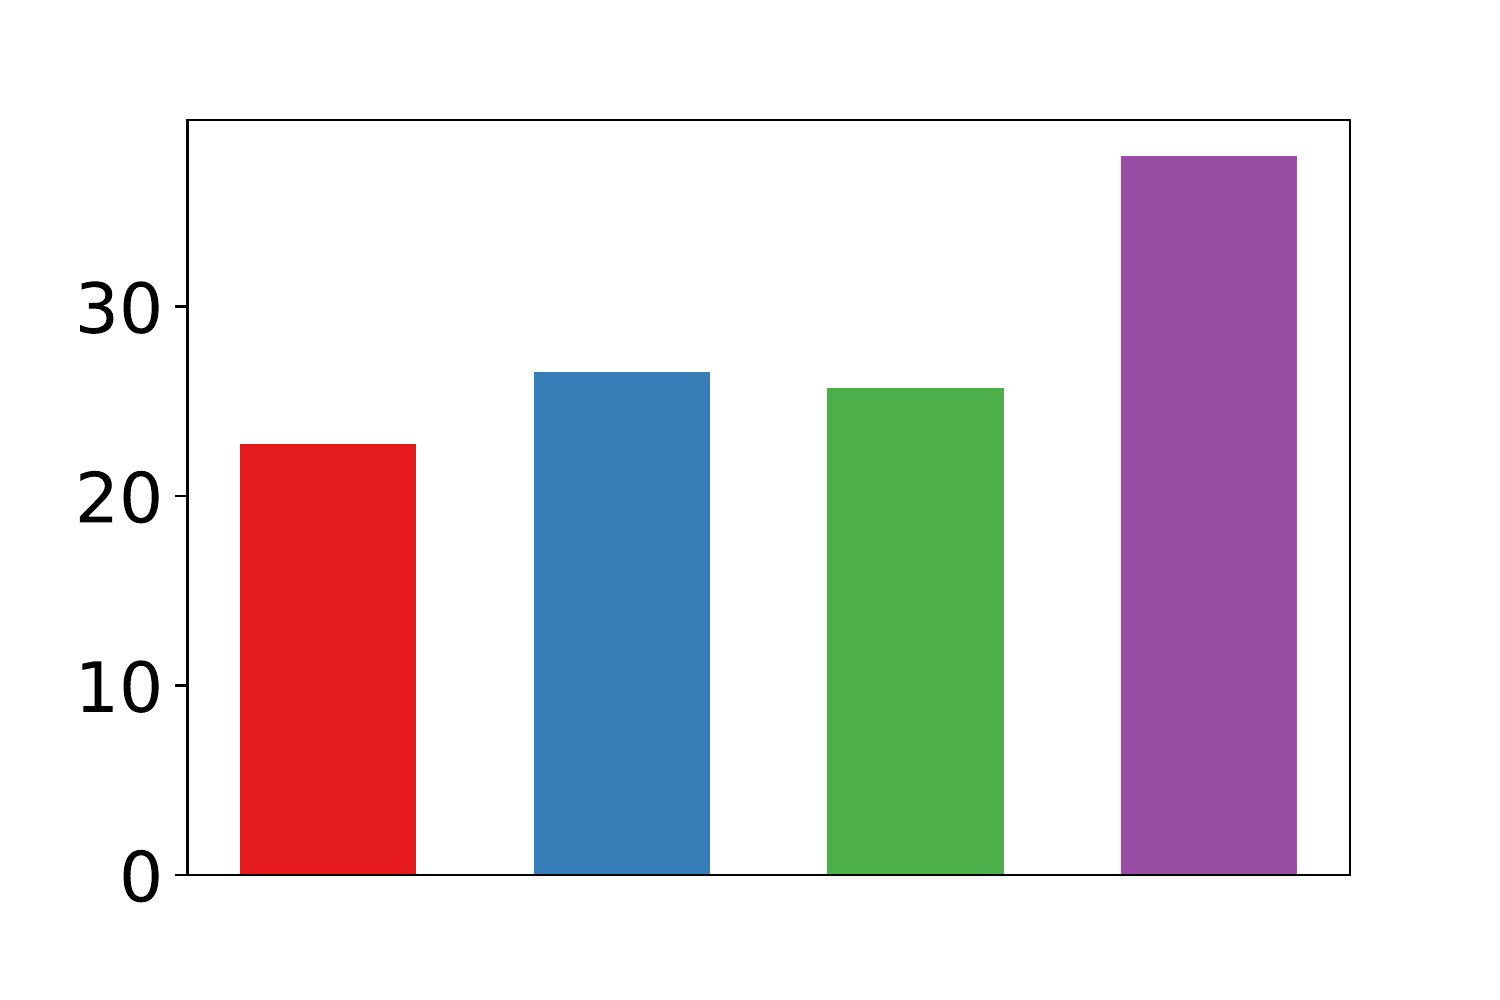_tex}
  \end{subfigure}
  \caption{Layer 1}
  \label{fig:int_stable_lyr_cush}
\end{figure}
\end{center}

\begin{center}
  \begin{figure}[h!]
  \begin{subfigure}[c]{0.245\linewidth}
    \centering
    \def\svgwidth{0.99\columnwidth}
    \input{./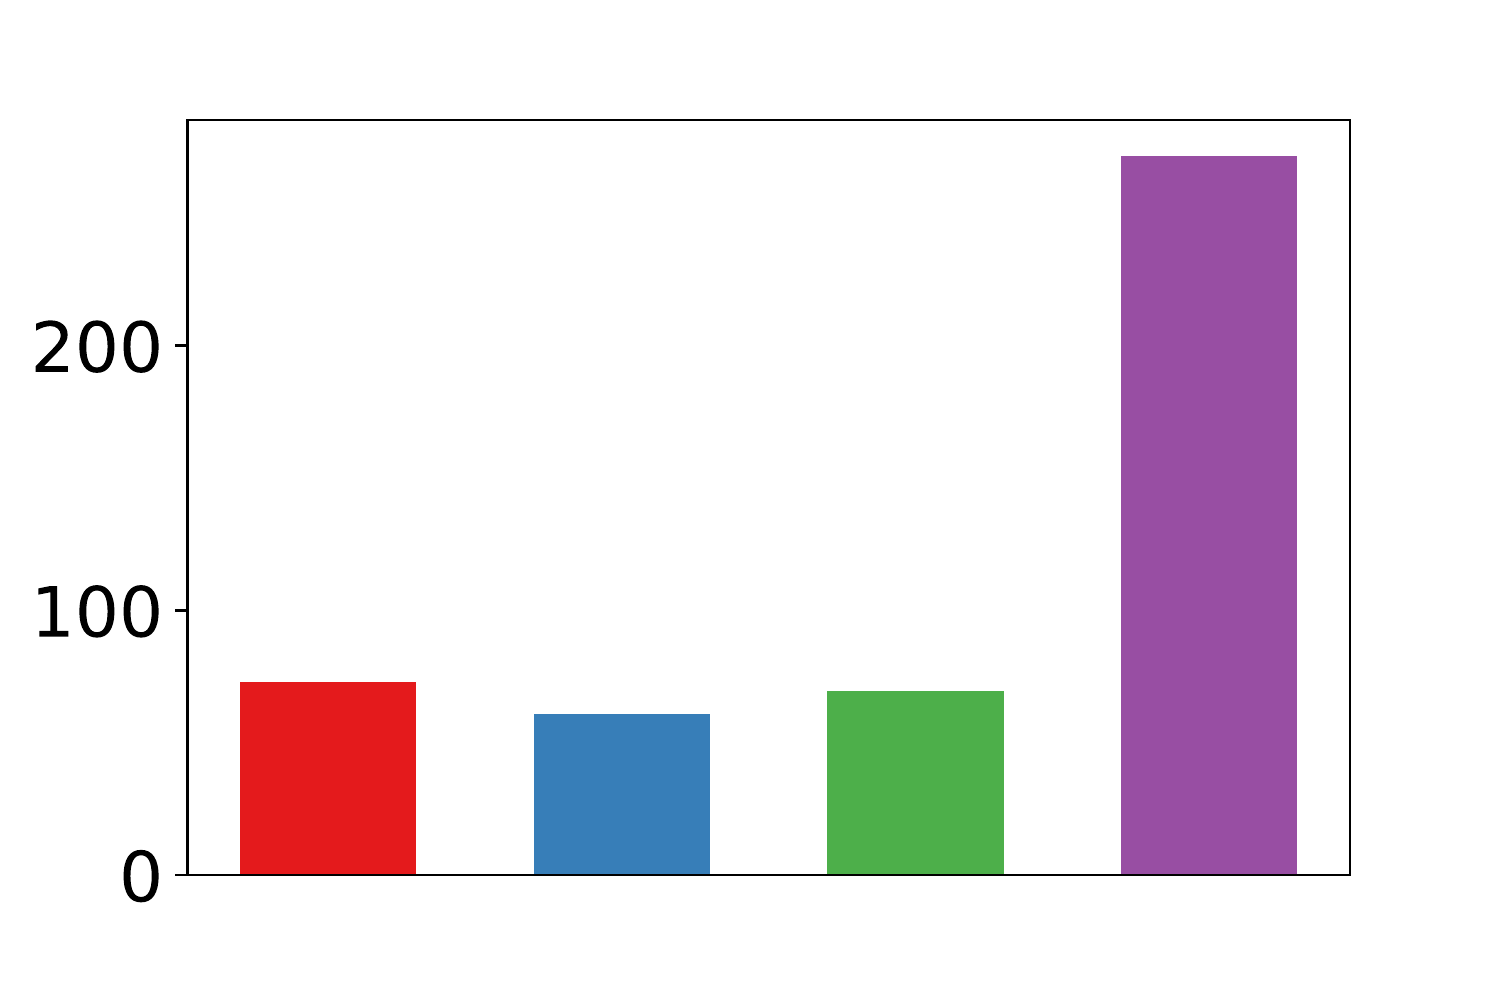_tex}
  \end{subfigure}
  \begin{subfigure}[c]{0.245\linewidth}
    \centering
    \def\svgwidth{0.99\columnwidth}
    \input{./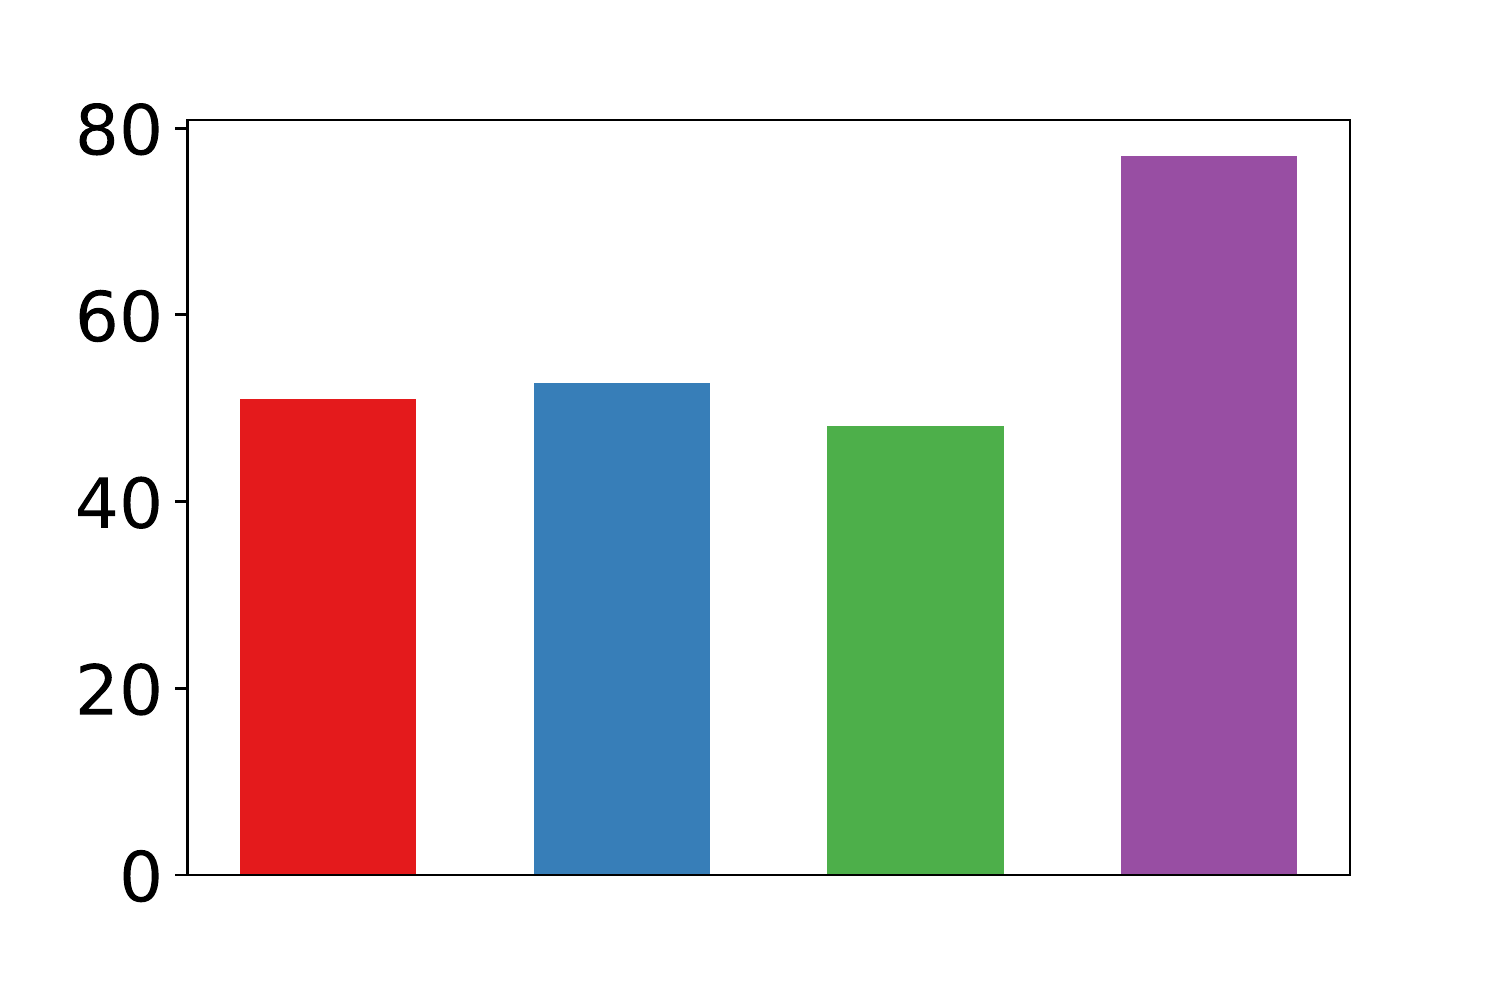_tex}
  \end{subfigure}
  \begin{subfigure}[c]{0.245\linewidth}
    \centering
    \def\svgwidth{0.99\columnwidth}
    \input{./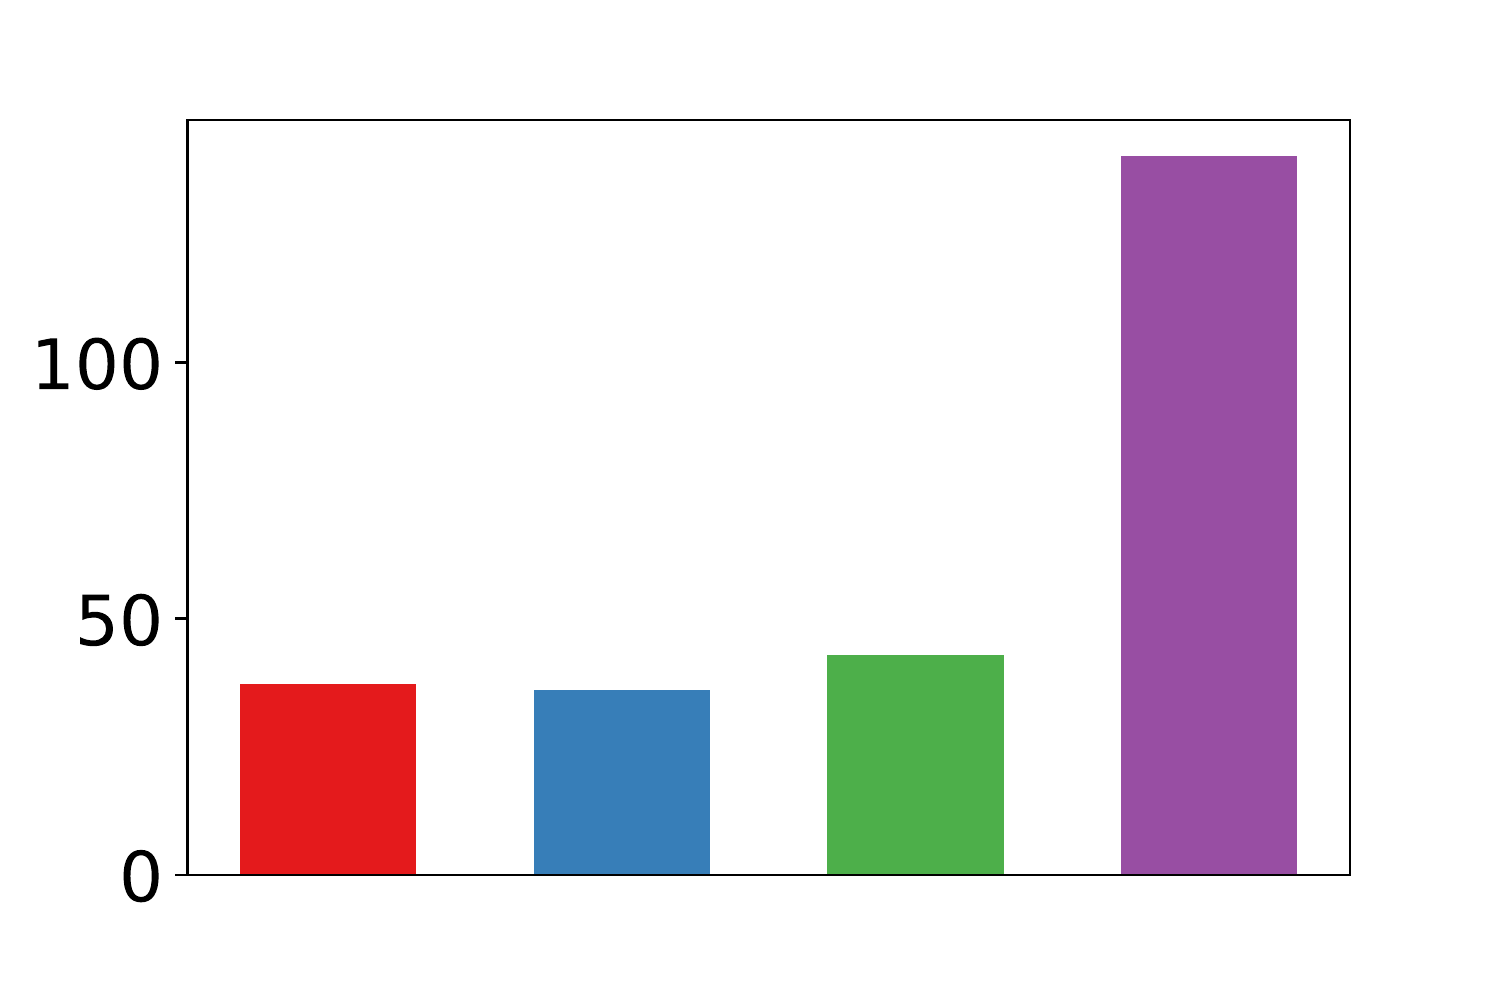_tex}
  \end{subfigure}
  \begin{subfigure}[c]{0.245\linewidth}
    \centering
    \def\svgwidth{0.99\columnwidth}
    \input{./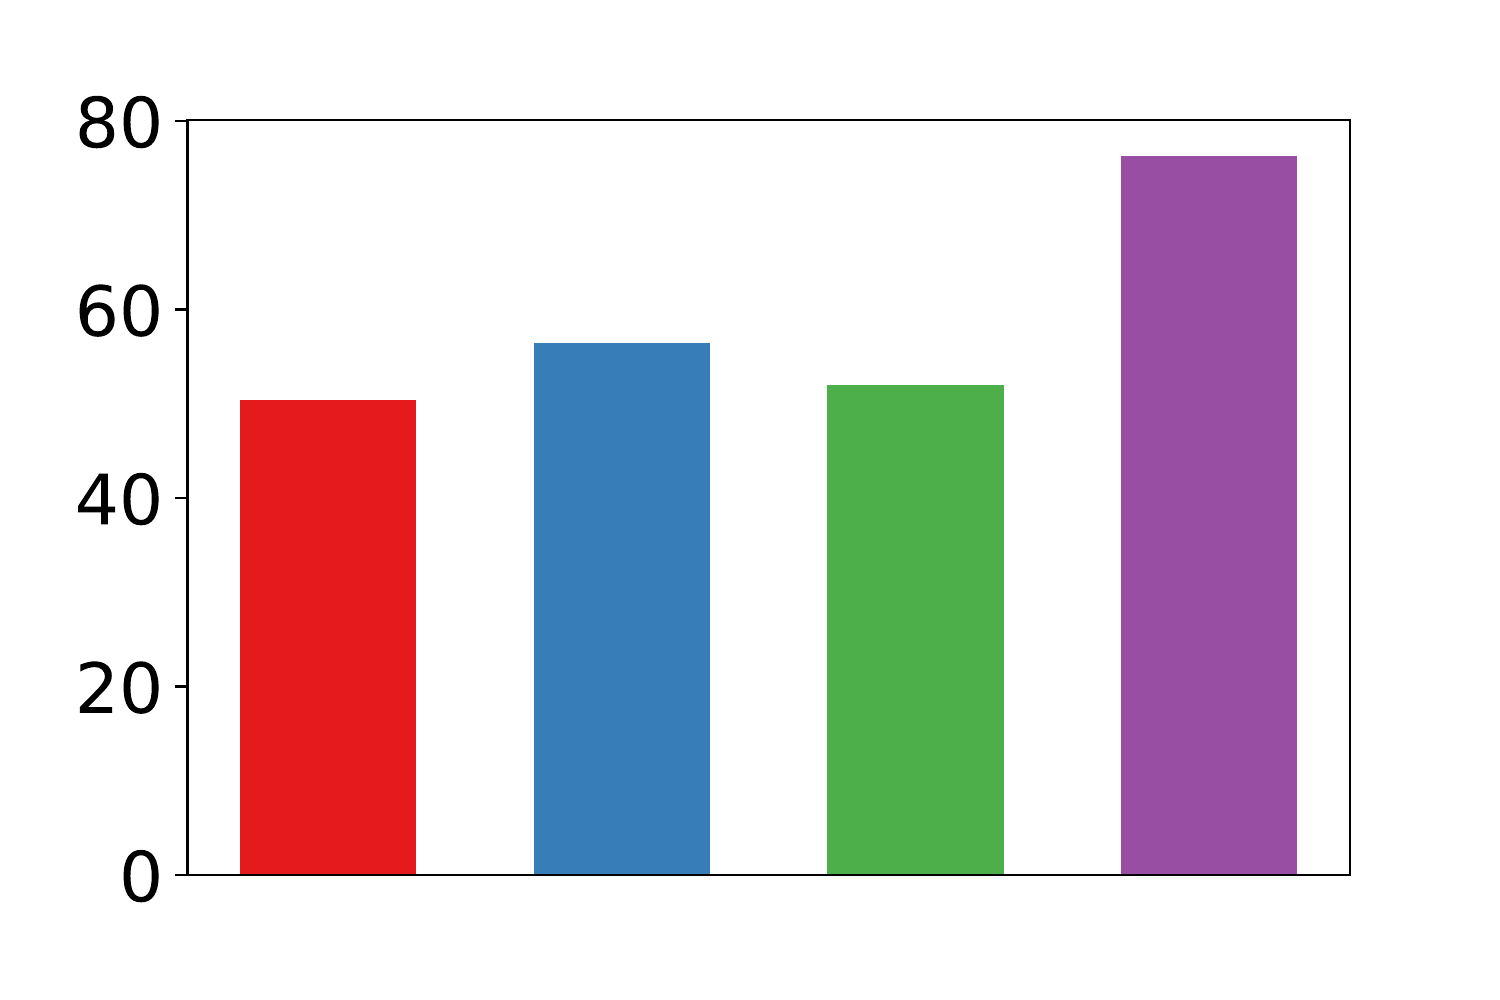_tex}
  \end{subfigure}
  \caption{Layer 2}
  \label{fig:int_stable_lyr2_cush}
\end{figure}
\end{center}

\begin{center}
  \begin{figure}[h!]
  \begin{subfigure}[c]{0.245\linewidth}
    \centering
    \def\svgwidth{0.99\columnwidth}
    \input{./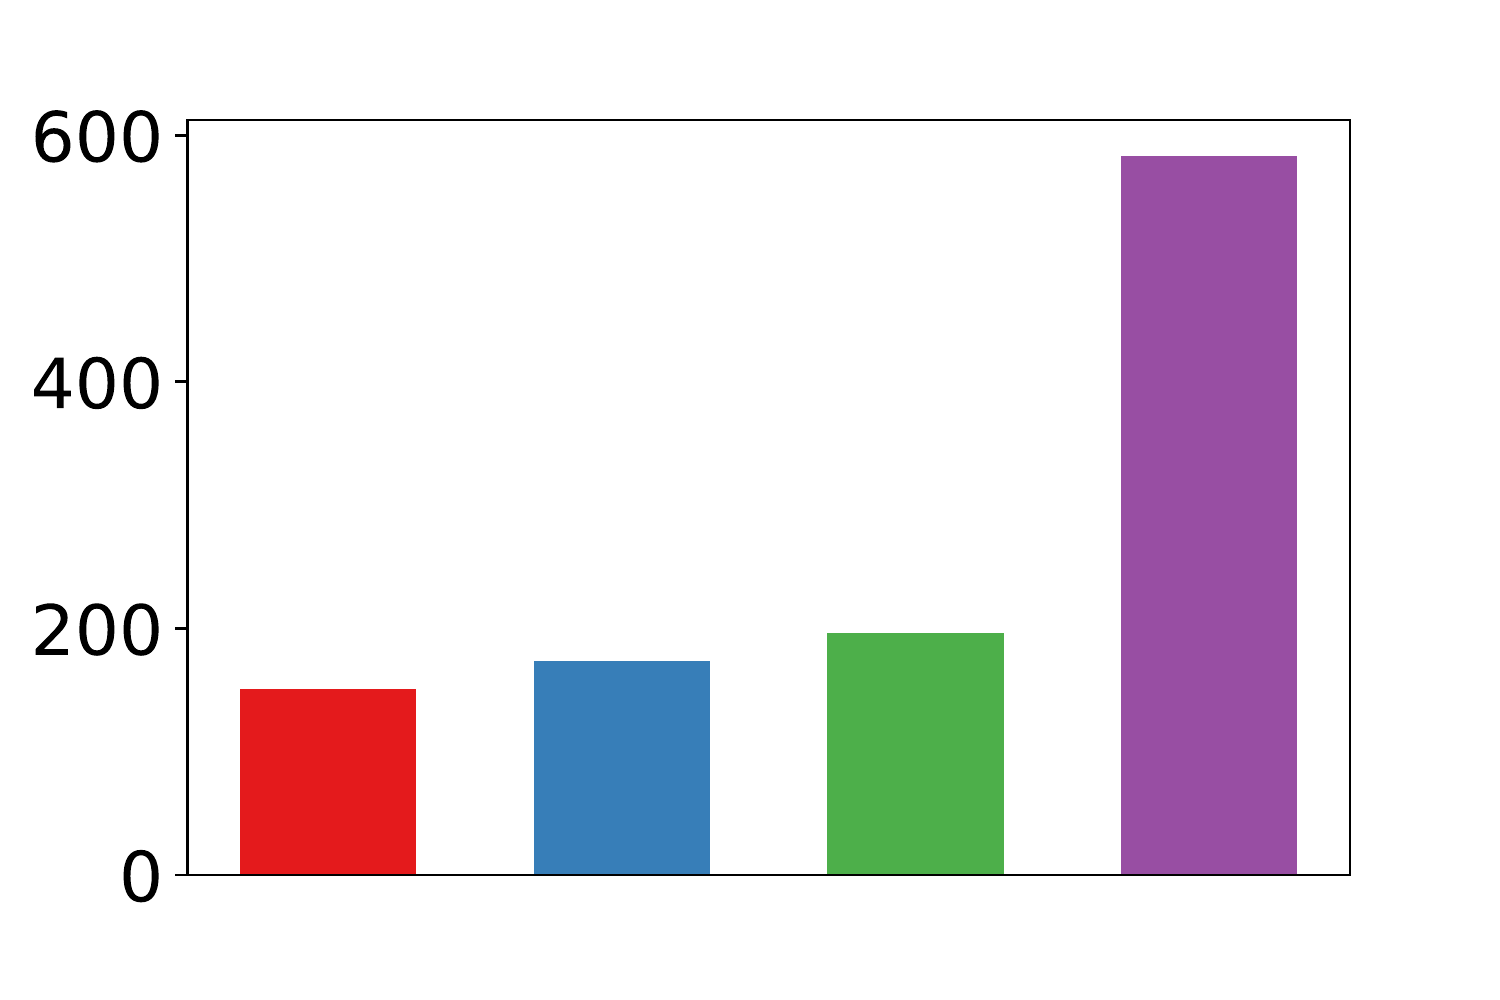_tex}
  \end{subfigure}
  \begin{subfigure}[c]{0.245\linewidth}
    \centering
    \def\svgwidth{0.99\columnwidth}
    \input{./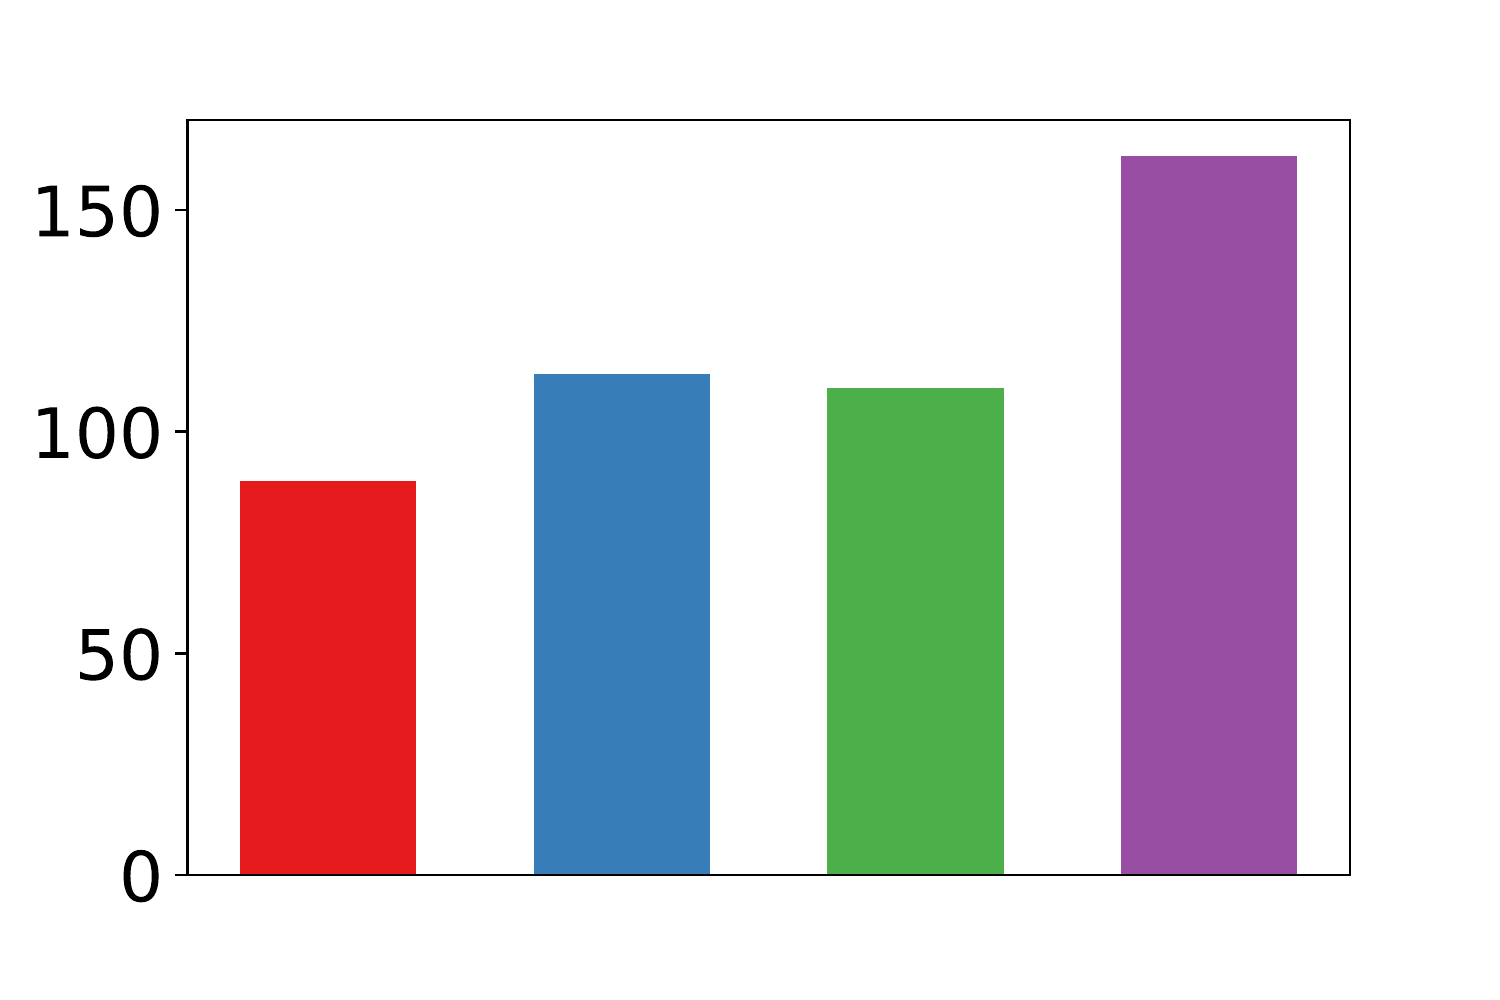_tex}
  \end{subfigure}
  \begin{subfigure}[c]{0.245\linewidth}
    \centering
    \def\svgwidth{0.99\columnwidth}
    \input{./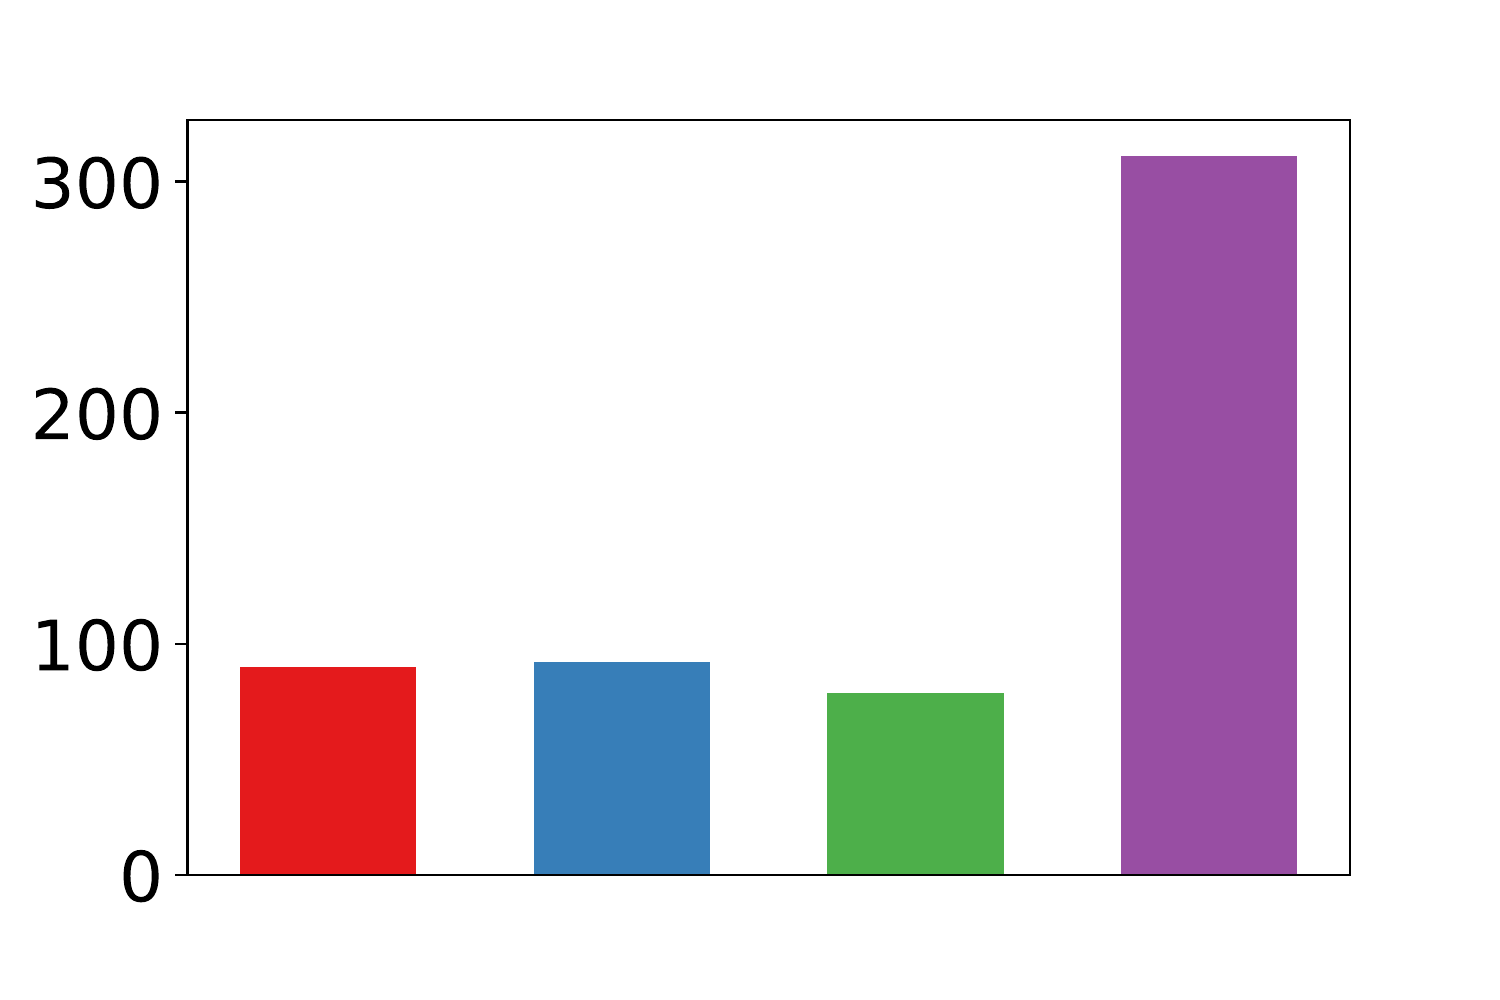_tex}
  \end{subfigure}
  \begin{subfigure}[c]{0.245\linewidth}
    \centering
    \def\svgwidth{0.99\columnwidth}
    \input{./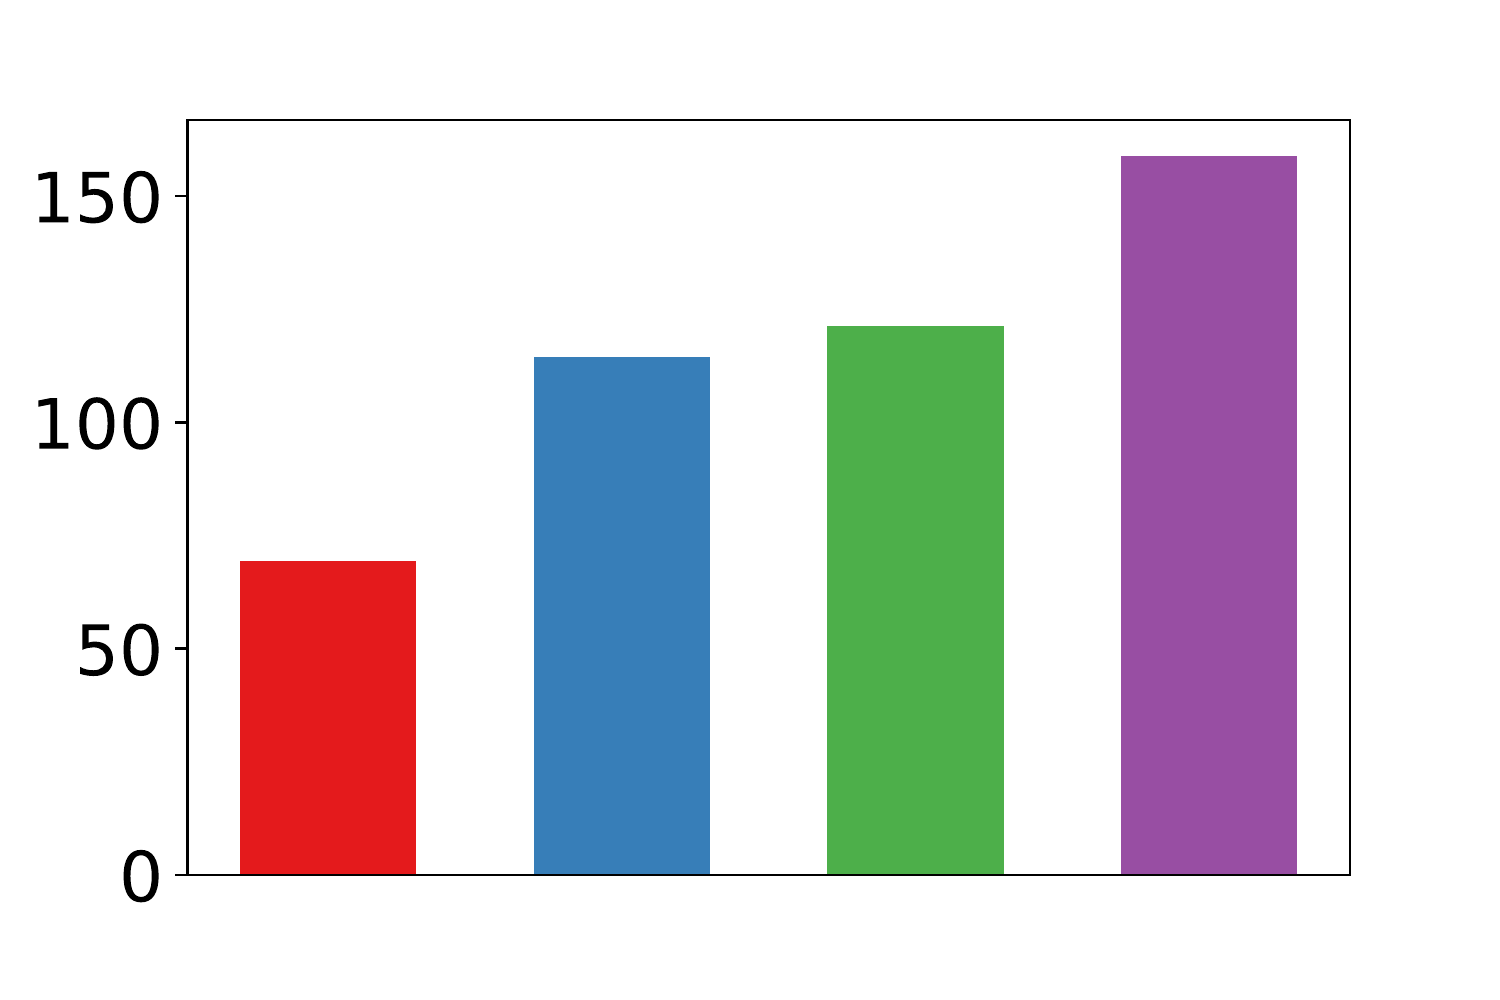_tex}
  \end{subfigure}
  \caption{Layer 3}
  \label{fig:int_stable_lyr3_cush}
\end{figure}
\end{center}
\vspace{-50pt}
  \begin{figure}[h!]
  \begin{subfigure}[c]{0.245\linewidth}
    \centering
    \def\svgwidth{0.99\columnwidth}
    \input{./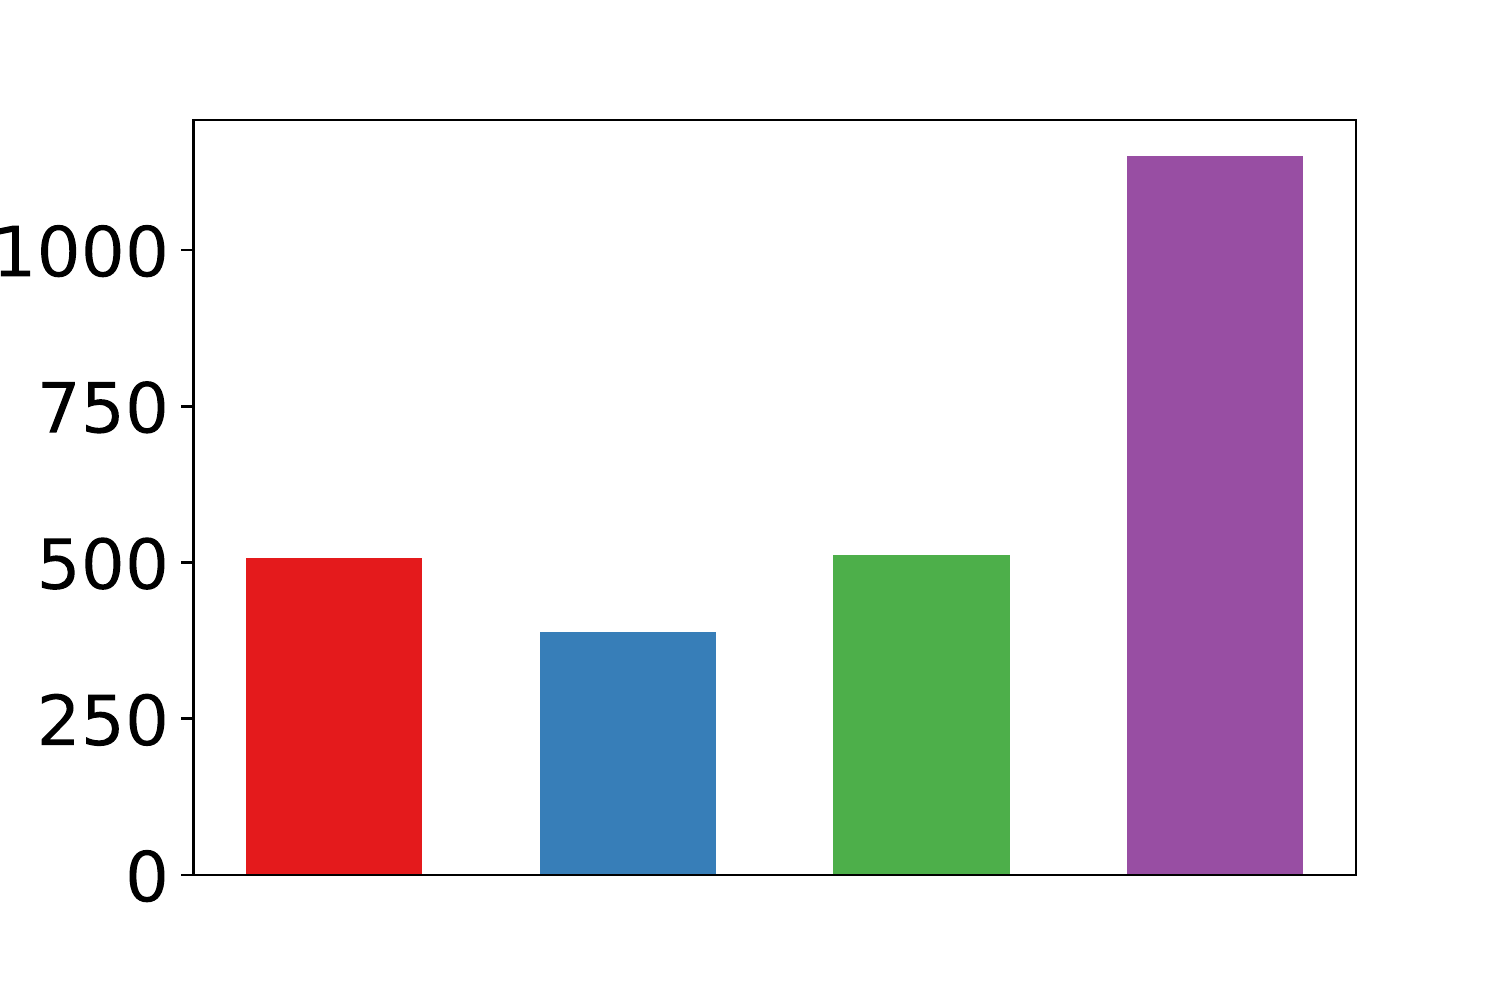_tex}
  \end{subfigure}
  \begin{subfigure}[c]{0.245\linewidth}
    \centering
    \def\svgwidth{0.99\columnwidth}
    \input{./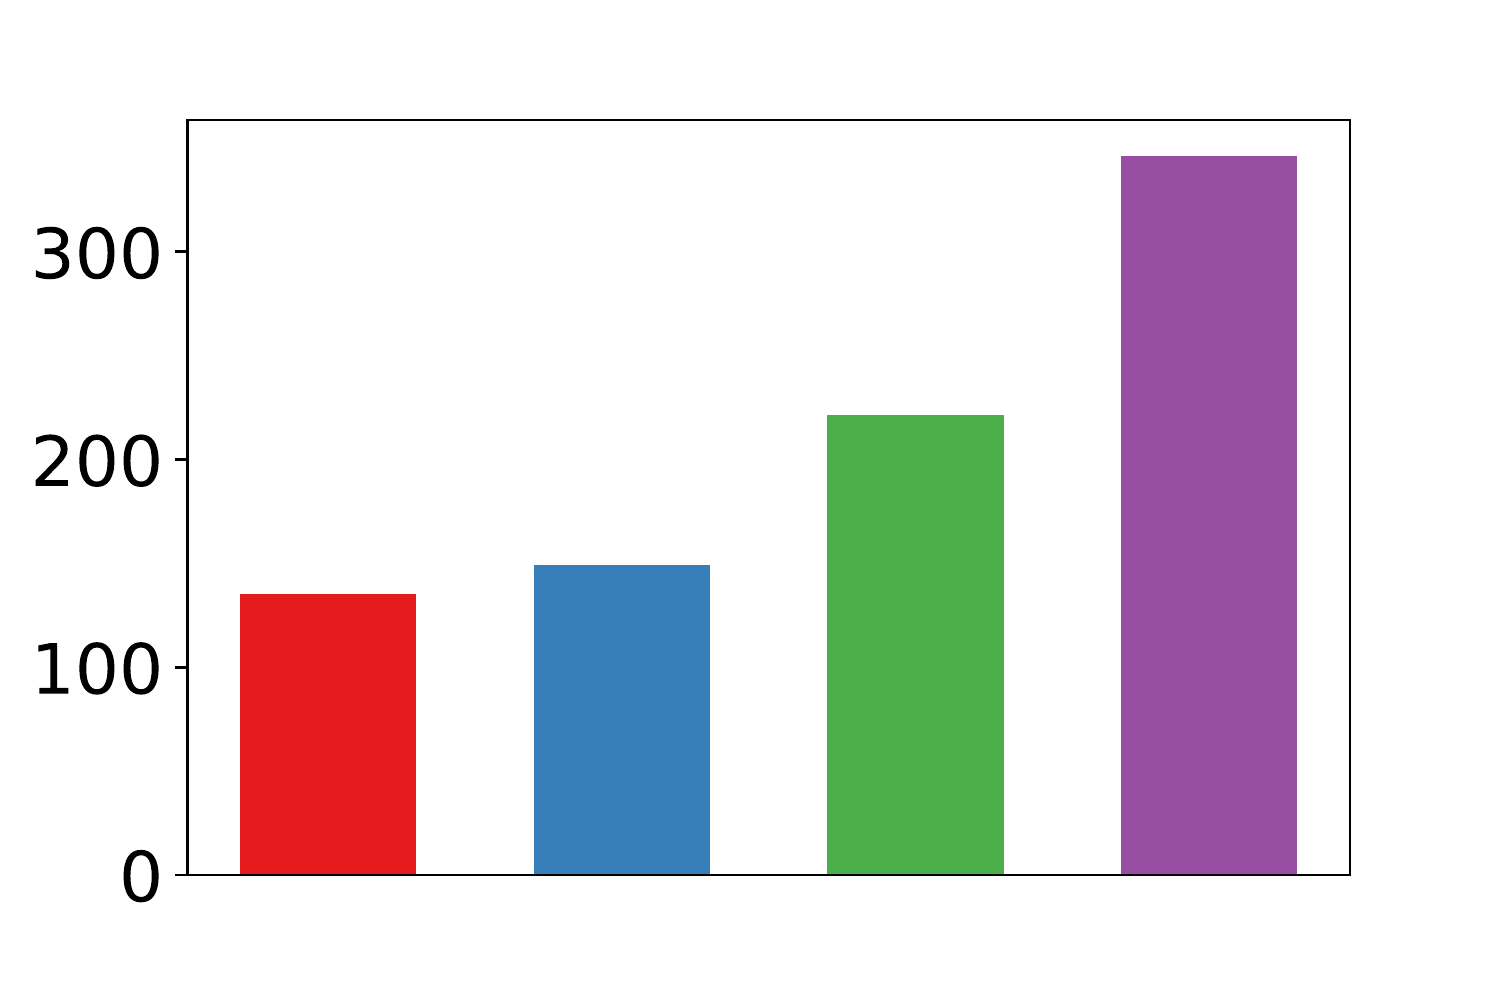_tex}
  \end{subfigure}
  \begin{subfigure}[c]{0.245\linewidth}
    \centering
    \def\svgwidth{0.99\columnwidth}
    \input{./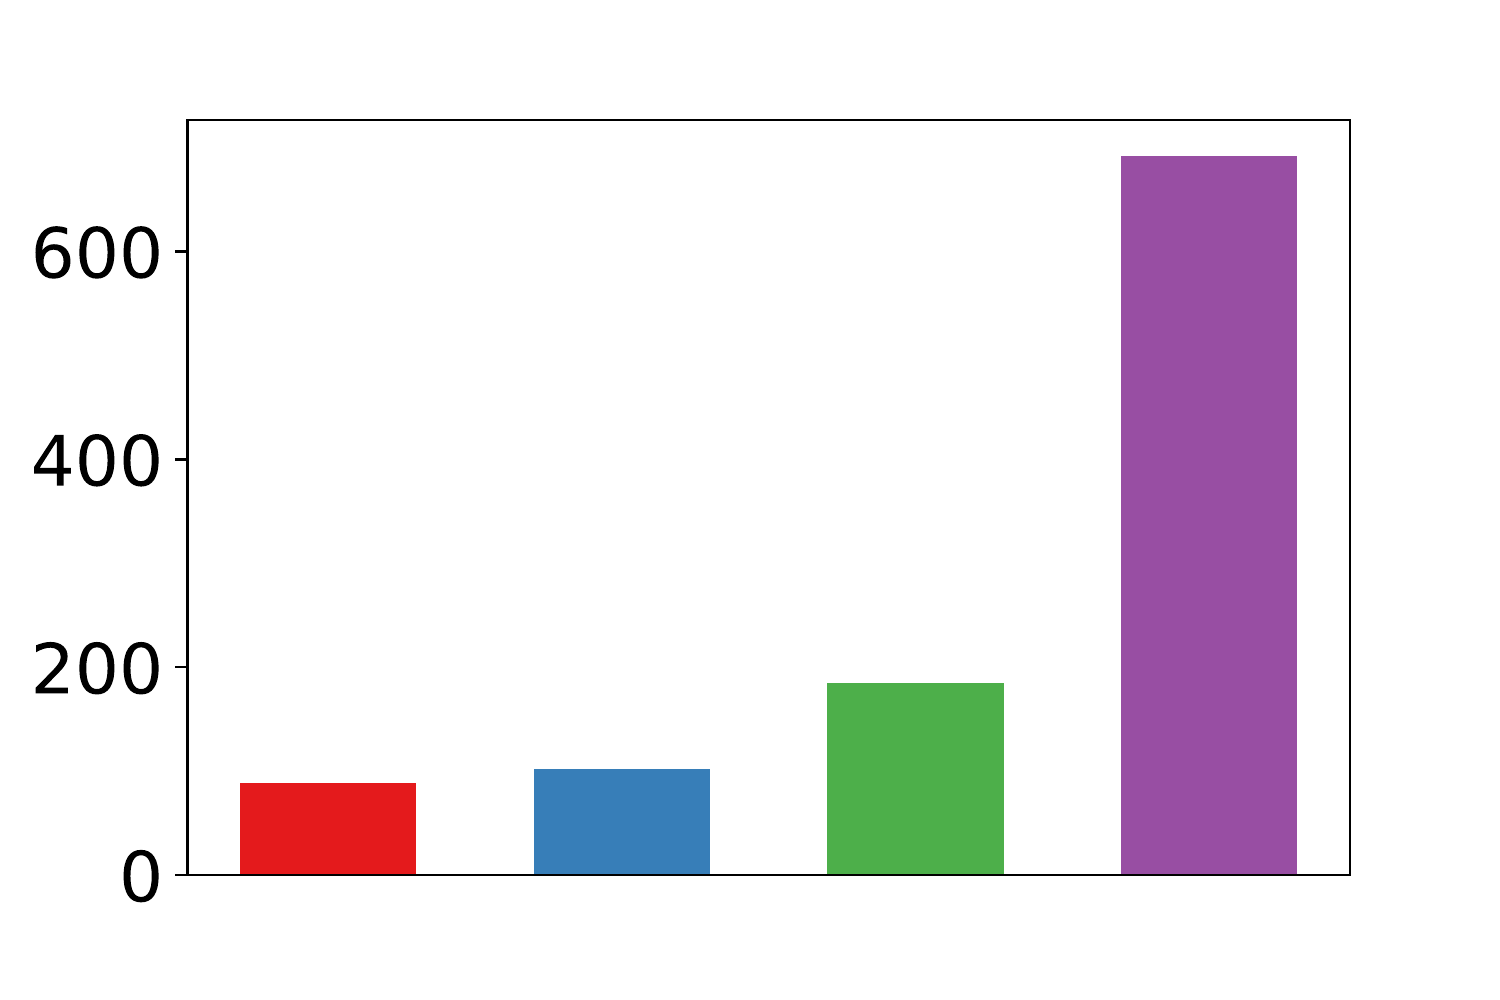_tex}
  \end{subfigure}
  \begin{subfigure}[c]{0.245\linewidth}
    \centering
    \def\svgwidth{0.99\columnwidth}
    \input{./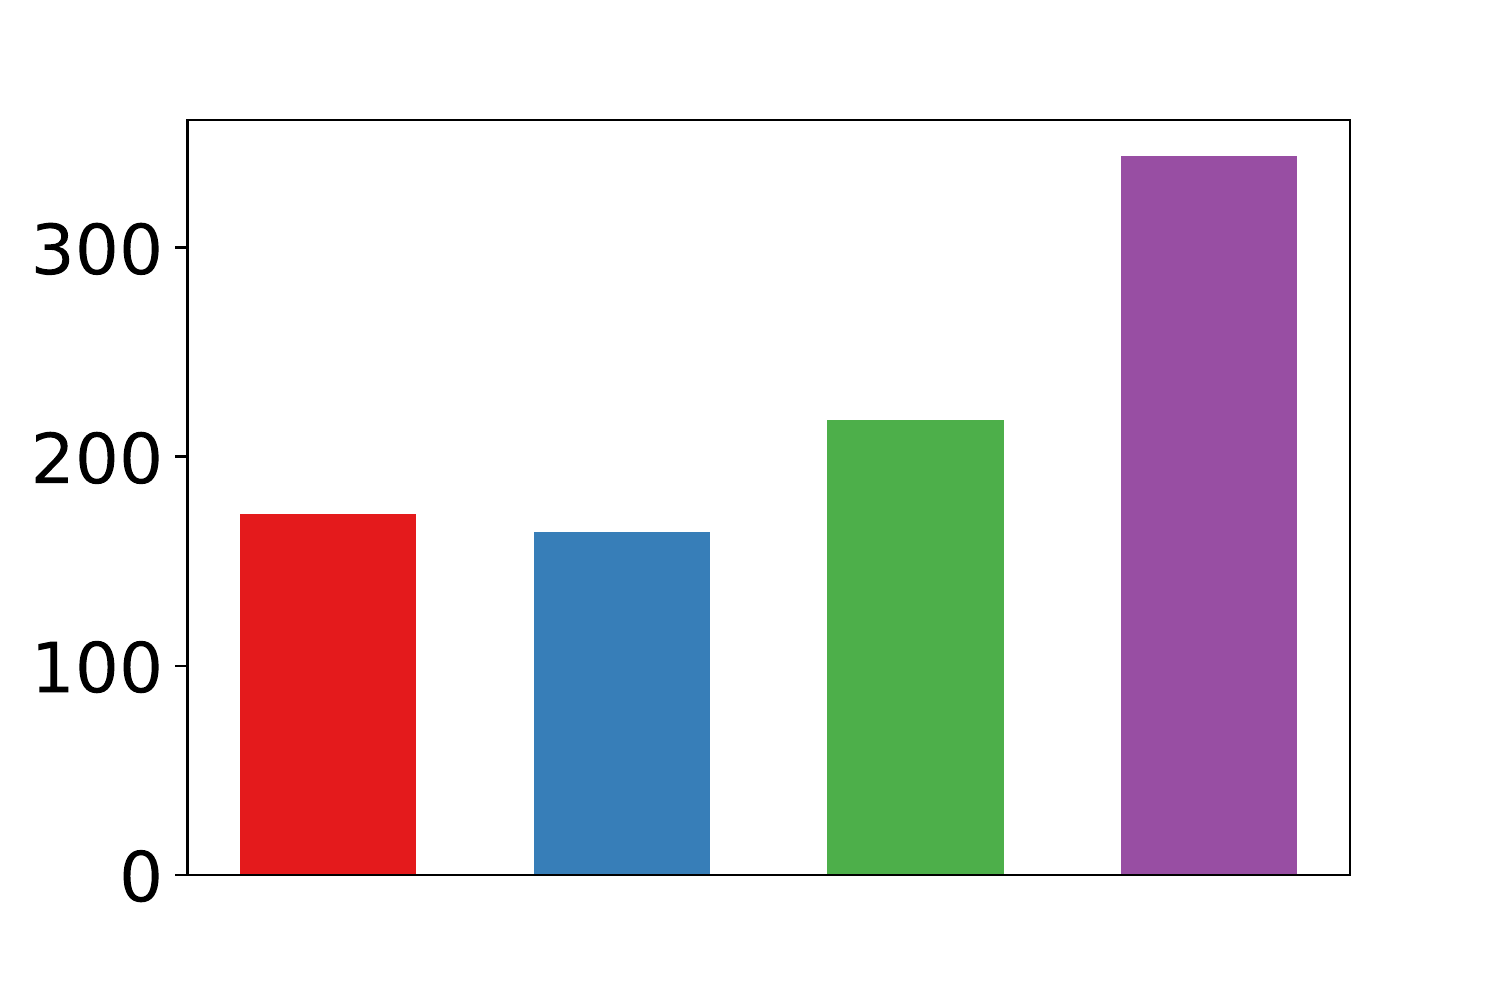_tex}
  \end{subfigure}
  \caption{Layer 4}
  \label{fig:int_stable_lyr4_cush}
\end{figure}
