# Supplementary material for: Identifying and Exploiting Structures for Reliable Deep Learning
Source: arXiv:2108.07083 source file (2021-08-16)
Supplement: Supplementary file 3 [file appendix.tex]

\chapter{Proofs for~\Cref{sec:math-prer-notat}}
\label{sec:proof-sect-eqrefs}

\clearpage
\section{Proofs for \ref{sec:generalisation}}
\label{sec:proofs-refs-gen}

\input{generalization_proofs}

\clearpage
